# Supplementary material for: Analytical Solution of Similar Oblate Spheroidal Coordinate System
Source: arXiv:2109.12057 ancillary file (2021-09-06)
Supplement: Supplementary file 1 [file Supplement_SOS_A.pdf]

# Analytical solution of Similar Oblate Spheroidal Coordinate System

---

Pavel Strunz

Nuclear Physics Institute of the CAS, Řež, Czech Republic

e-mail: strunz@ujf.cas.cz

## Supplement A

### Coordinates x and z as power series with generalized binomial coefficients

Let us list some useful identities which will be used in the modification of the form of power series with generalized binomial coefficients used in formulas for coordinate transformation. First, identities following from the definitions of generalized binomial coefficients and generalized factorial are listed. The rising factorial identities line is

$$\beta^{\bar{k}} = \frac{\Gamma(\beta + k)}{\Gamma(\beta)} = \frac{(\beta + k - 1)!}{(\beta - 1)!} = \binom{\beta + k - 1}{k} k! = \prod_{j=1}^k (\beta + j - 1) \quad , \quad (A1)$$

where  $\beta$  is a real number and  $k$  is a non-negative integer (the value of the rising factorial is taken to be 1, i.e. an empty product, when  $k=0$ ). The falling factorial identities line is

$$\beta^{\underline{k}} = \frac{\Gamma(\beta + 1)}{\Gamma(\beta - k + 1)} = \frac{\beta!}{(\beta - k)!} = \binom{\beta}{k} k! = \prod_{j=1}^k (\beta - j + 1) \quad (A2)$$

The last expression on the right side, the product, is of advantage for numerical calculations of generalized binomial coefficients.

In the derivations, the following series of expressions transforming  $\Gamma$  function values into the generalized binomial coefficients and their identities will be used:

$$\frac{\Gamma(k + \beta)}{\Gamma(1 + \beta)} = \frac{(k + \beta)^{\underline{k}}}{k + \beta} = \binom{\beta + k}{k} \frac{k!}{\beta + k} = \binom{\beta + k - 1}{k} \frac{k!}{\beta} = (-1)^{k+1} \binom{-\beta}{k} \frac{k!}{-\beta} = (-1)^k \frac{(-\beta)^{\underline{k}}}{\beta} \quad (A3)$$

Note, that this ratio of  $\Gamma$  function values (depending on the parameter  $\beta$ ) can be expressed in three distinct forms of binomial coefficients. In order to complete the set of binomial identities used later in the paper, the following identity is also listed:

$$\binom{\alpha}{k} = \binom{\alpha}{k-1} \frac{\alpha - k + 1}{k} \quad (A4)$$

where  $\alpha$  is a real number.

From (26) and using the part of the combinatorial identity (A3) including the first binomial coefficient (from the left) with  $\beta$  equal to  $\left[\frac{1+\mu}{2} + \mu k\right]$ , we arrive at the formula for  $z$  in the **small- $v$  region** in the form

$$\begin{aligned}
z &= W(1+\mu)^{1/2} \frac{R}{2} \sum_{k=0}^{\infty} \binom{\frac{1+\mu}{2} + (1+\mu)k}{k} \frac{(-W^2)^k}{\frac{1+\mu}{2} + (1+\mu)k} \\
&= W(1+\mu)^{1/2} \frac{R}{2} \sum_{k=0}^{\infty} \frac{\Gamma(k + [\frac{1+\mu}{2} + \mu k]) (-W^2)^k}{\Gamma(1 + [\frac{1+\mu}{2} + \mu k]) k!}
\end{aligned}
\tag{A5a}$$

or (when using the identity in the middle of (A3))

$$z = W(1+\mu)^{1/2} \frac{R}{2} \sum_{k=0}^{\infty} \binom{(\frac{1+\mu}{2} - 1) + (1+\mu)k}{k} \frac{(-W^2)^k}{\frac{1+\mu}{2} + \mu k}
\tag{A5b}$$

or (when using the identity in the right side of (A3)):

$$z = W(1+\mu)^{1/2} \frac{R}{2} \sum_{k=0}^{\infty} \binom{-\frac{1+\mu}{2} - \mu k}{k} \frac{-(W^2)^k}{-\frac{1+\mu}{2} - \mu k}
\tag{A5c}$$

Two of the above forms of  $z$  are to be used in the further calculation of derivatives.

In the special case of  $v=0$  (i.e. equatorial plane),  $W$  equals to zero and  $z=0$ , as would be expected.

Accordingly, the coordinate  $x$  in the small- $v$  region can be written using (27) and the identities (A3) with  $\beta$  equal to  $[\frac{1}{2} + \mu k]$  either in the form

$$x = \frac{R}{2} \sum_{k=0}^{\infty} \binom{\frac{1}{2} + (1+\mu)k}{k} \frac{(-W^2)^k}{\frac{1}{2} + (1+\mu)k} = \frac{R}{2} \sum_{k=0}^{\infty} \frac{\Gamma(k + [\frac{1}{2} + \mu k]) (-W^2)^k}{\Gamma(1 + [\frac{1}{2} + \mu k]) k!}
\tag{A6a}$$

or in the form

$$x = \frac{R}{2} \sum_{k=0}^{\infty} \binom{-\frac{1}{2} + (1+\mu)k}{k} \frac{(-W^2)^k}{\frac{1}{2} + \mu k}
\tag{A6b}$$

or in the equivalent form

$$x = \frac{R}{2} \sum_{k=0}^{\infty} \binom{-\frac{1}{2} - \mu k}{k} \frac{-(W^2)^k}{-\frac{1}{2} - \mu k}
\tag{A6c}$$

In the special case of  $v=0$  (i.e. equatorial plane),  $W$  equals to zero and the only non-zero term in the power series is the one with  $k=0$ . Then  $x=R$ , as would be expected.

For the **large- $v$  region**, the derivation of the appropriate forms of the  $x$  and  $z$  coordinates is only slightly more difficult. The coordinate  $z$  for the large- $v$  region can be obtained from (34) with the help of the split  $\frac{1}{1+\mu}k = k - \frac{\mu}{1+\mu}k$ , resulting in  $\beta$  used in the (A3) identity being equal to  $[\frac{1}{2} - \frac{\mu}{1+\mu}k]$ . Then

$$\begin{aligned}
z &= \frac{1}{(1+\mu)^{1/2}} \frac{R}{2} \sum_{k=0}^{\infty} \binom{\frac{1}{2} + \frac{1}{1+\mu}k}{k} \frac{\left(-W^{-\frac{2}{1+\mu}}\right)^k}{\frac{1}{2} + \frac{1}{1+\mu}k} = \\
&= \frac{1}{(1+\mu)^{1/2}} \frac{R}{2} \sum_{k=0}^{\infty} \binom{\left[\frac{1}{2} - \frac{\mu}{1+\mu}k\right] + k}{k} \frac{\left(-W^{-\frac{2}{1+\mu}}\right)^k}{\left[\frac{1}{2} - \frac{\mu}{1+\mu}k\right] + k} \\
&= \frac{1}{(1+\mu)^{1/2}} \frac{R}{2} \sum_{k=0}^{\infty} \frac{\Gamma\left(k + \left[\frac{1}{2} - \frac{\mu}{1+\mu}k\right]\right) \left(-W^{-\frac{2}{1+\mu}}\right)^k}{\Gamma\left(1 + \left[\frac{1}{2} - \frac{\mu}{1+\mu}k\right]\right) k!}
\end{aligned} \tag{A7a}$$

or (when using the identity in the middle of (A3)) equivalently

$$z = \frac{1}{(1+\mu)^{1/2}} \frac{R}{2} \sum_{k=0}^{\infty} \binom{-\frac{1}{2} + \frac{1}{1+\mu}k}{k} \frac{\left(-W^{-\frac{2}{1+\mu}}\right)^k}{\frac{1}{2} - \frac{\mu}{1+\mu}k} \tag{A7b}$$

or (when using the identity in the right side of (A3))

$$z = \frac{1}{(1+\mu)^{1/2}} \frac{R}{2} \sum_{k=0}^{\infty} \binom{-\frac{1}{2} + \frac{\mu}{1+\mu}k}{k} \frac{-\left(W^{-\frac{2}{1+\mu}}\right)^k}{-\frac{1}{2} + \frac{\mu}{1+\mu}k} \tag{A7c}$$

In the special case of  $\nu=\pi/2$  (i.e. polar axis),  $W^1$  equals to zero and the only non-zero term in the power series is the one with  $k=0$ . Then  $z=R/(1+\mu)^{1/2}$ , as would be expected.

The coordinate  $x$  for large  $\nu$  region can be obtained from (35) with the help of the split  $\frac{1}{1+\mu}k = k - \frac{\mu}{1+\mu}k$ , resulting in  $\beta$  used in the (A3) identity being equal to  $\left[\frac{1}{2(1+\mu)} - \frac{\mu}{1+\mu}k\right]$ . Then

$$\begin{aligned}
x &= \frac{W^{-\frac{1}{1+\mu}}}{1+\mu} \frac{R}{2} \sum_{k=0}^{\infty} \binom{\frac{1}{2(1+\mu)} + \frac{1}{1+\mu}k}{k} \frac{\left(-W^{-\frac{2}{1+\mu}}\right)^k}{\frac{1}{2(1+\mu)} + \frac{1}{1+\mu}k} \\
&= \frac{W^{-\frac{1}{1+\mu}}}{1+\mu} \frac{R}{2} \sum_{k=0}^{\infty} \binom{\left[\frac{1}{2(1+\mu)} - \frac{\mu}{1+\mu}k\right] + k}{k} \frac{\left(-W^{-\frac{2}{1+\mu}}\right)^k}{\left[\frac{1}{2(1+\mu)} - \frac{\mu}{1+\mu}k\right] + k} \\
&= \frac{W^{-\frac{1}{1+\mu}}}{1+\mu} \frac{R}{2} \sum_{k=0}^{\infty} \frac{\Gamma\left(k + \left[\frac{1}{2(1+\mu)} - \frac{\mu}{1+\mu}k\right]\right) \left(-W^{-\frac{2}{1+\mu}}\right)^k}{\Gamma\left(1 + \left[\frac{1}{2(1+\mu)} - \frac{\mu}{1+\mu}k\right]\right) k!}
\end{aligned} \tag{A8a}$$

or in the form

$$x = \frac{W^{-\frac{1}{1+\mu}}}{1+\mu} \frac{R}{2} \sum_{k=0}^{\infty} \binom{\left(\frac{1}{2(1+\mu)} - 1\right) + \frac{1}{1+\mu}k}{k} \frac{\left(-W^{-\frac{2}{1+\mu}}\right)^k}{\frac{1}{2(1+\mu)} - \frac{\mu}{1+\mu}k} \tag{A8b}$$

or in the form

$$x = \frac{W^{-\frac{1}{1+\mu}}}{1+\mu} \frac{R}{2} \sum_{k=0}^{\infty} \left( -\frac{1}{2(1+\mu)} + \frac{\mu}{1+\mu} k \right) \frac{-\left(W^{-\frac{2}{1+\mu}}\right)^k}{-\frac{1}{2(1+\mu)} + \frac{\mu}{1+\mu} k} . \quad (\text{A8c})$$

In the special case of  $\nu=\pi/2$  (i.e. polar axis),  $W^1$  equals to zero and thus  $x=0$ , as expected.
