# Supplementary material for: Analytical Solution of Similar Oblate Spheroidal Coordinate System
Source: arXiv:2109.12057 ancillary file (2021-09-06)
Supplement: Supplementary file 2 [file Supplement_SOS_C.pdf]

# Analytical solution of Similar Oblate Spheroidal Coordinate System

---

Pavel Strunz  
Nuclear Physics Institute of the CAS, Řež, Czech Republic  
e-mail: strunz@ujf.cas.cz

## Supplement C

### Partial derivatives with respect to $v$ in the large- $v$ region

Here, partial derivatives with respect to  $v$  are determined for the large- $v$  region.

#### *Derivative of $x$ with respect to $v$*

First, let's determine the partial derivative of the coordinate  $x$  with respect to  $v$ . In order to use Jensen (Gould 1972) and Hagen-Rothe (Chu 2010, Chu 2013) identities later, the 3<sup>rd</sup> form (A8c) of the coordinate  $x$  is used for the derivative determination. The dependence (22) of  $W$  on  $v$  has to be considered. Then

$$\begin{aligned}
\frac{\partial x(v, R)}{\partial v} &= \frac{\partial}{\partial v} \left\{ \frac{W^{-\frac{1}{1+\mu}}}{1+\mu} \frac{R}{2} \sum_{k=0}^{\infty} \left( -\frac{1}{2(1+\mu)} + \frac{\mu}{1+\mu} k \right) \frac{-\left(W^{-\frac{2}{1+\mu}}\right)^k}{-\frac{1}{2(1+\mu)} + \frac{\mu}{1+\mu} k} \right\} \\
&= \frac{1}{1+\mu} \frac{R}{2} \frac{\partial}{\partial v} \left\{ W^{-\frac{1}{\mu}} \sum_{k=0}^{\infty} \left( -\frac{1}{2(1+\mu)} + \frac{\mu}{1+\mu} k \right) \frac{-\left(W^{\frac{1}{\mu}}\right)^{-\frac{2\mu k}{1+\mu} - \frac{\mu}{1+\mu} + 1}}{-\frac{1}{2(1+\mu)} + \frac{\mu}{1+\mu} k} \right\} = \\
&= \frac{1}{1+\mu} \frac{R}{2} \left\{ \left[ \frac{\partial}{\partial v} \left( W^{-\frac{1}{\mu}} \right) \sum_{k=0}^{\infty} \left( -\frac{1}{2(1+\mu)} + \frac{\mu}{1+\mu} k \right) \frac{\left(W^{\frac{1}{\mu}}\right)^{-\frac{2\mu k}{1+\mu} - \frac{\mu}{1+\mu} + 1}}{\frac{1}{2(1+\mu)} - \frac{\mu}{1+\mu} k} \right] \right. \\
&\quad \left. + \left[ W^{-\frac{1}{\mu}} \sum_{k=0}^{\infty} \left( -\frac{1}{2(1+\mu)} + \frac{\mu}{1+\mu} k \right) \frac{\frac{\partial}{\partial v} \left( \left(W^{\frac{1}{\mu}}\right)^{-\frac{2\mu k}{1+\mu} - \frac{\mu}{1+\mu} + 1} \right)}{\frac{1}{2(1+\mu)} - \frac{\mu}{1+\mu} k} \right] \right\} = \\
&= \frac{1}{1+\mu} \frac{R}{2} \left\{ \left( W^{\frac{1}{\mu}} \right) \frac{\partial}{\partial v} \left( W^{-\frac{1}{\mu}} \right) \sum_{k=0}^{\infty} \left( -\frac{1}{2(1+\mu)} + \frac{\mu}{1+\mu} k \right) \frac{\left(W^{\frac{1}{\mu}}\right)^{-\frac{2\mu k}{1+\mu} - \frac{\mu}{1+\mu}}}{\frac{1}{2(1+\mu)} - \frac{\mu}{1+\mu} k} \right. \\
&\quad \left. + W^{-\frac{1}{\mu}} \frac{\partial}{\partial v} \left( W^{\frac{1}{\mu}} \right) \sum_{k=0}^{\infty} \left( -\frac{1}{2(1+\mu)} + \frac{\mu}{1+\mu} k \right) \frac{\left(-\frac{2\mu}{1+\mu} k + \frac{1}{1+\mu}\right) \left(W^{\frac{1}{\mu}}\right)^{-\frac{2\mu k}{1+\mu} - \frac{\mu}{1+\mu}}}{\frac{1}{2(1+\mu)} - \frac{\mu}{1+\mu} k} \right\} = \\
&= \frac{1}{1+\mu} \frac{R}{2} \frac{1}{\mu W} \frac{\partial W}{\partial v} \left\{ \sum_{k=0}^{\infty} \left( -\frac{1}{2(1+\mu)} + \frac{\mu}{1+\mu} k \right) \frac{\left(W^{-\frac{2}{1+\mu}}\right)^{k+\frac{1}{2}}}{-\frac{1}{2(1+\mu)} + \frac{\mu}{1+\mu} k} \right. \\
&\quad \left. + 2 \sum_{k=0}^{\infty} \left( -\frac{1}{2(1+\mu)} + \frac{\mu}{1+\mu} k \right) \left(W^{-\frac{2}{1+\mu}}\right)^{k+\frac{1}{2}} \right\} , \tag{C1}
\end{aligned}$$

which can be further shaped to

$$\begin{aligned} \frac{\partial x(v, R)}{\partial v} = \frac{1}{1+\mu} \frac{R}{2} \frac{1}{\mu W^{1+\frac{1}{1+\mu}}} \frac{\partial W}{\partial v} \left\{ \sum_{k=0}^{\infty} \left( -\frac{1}{2(1+\mu)} + \frac{\mu}{1+\mu} k \right) \frac{\left( W^{-\frac{2}{1+\mu}} \right)^k}{-\frac{1}{2(1+\mu)} + \frac{\mu}{1+\mu} k} \right. \\ \left. + 2 \sum_{k=0}^{\infty} \left( -\frac{1}{2(1+\mu)} + \frac{\mu}{1+\mu} k \right) \left( W^{-\frac{2}{1+\mu}} \right)^k \right\} \end{aligned} \quad (C2)$$

The terms in the sums with the same binomial coefficients can be put together, and then the derivative reads

$$\frac{\partial x(v, R)}{\partial v} = \frac{R}{1+\mu} \frac{1}{W^{1+\frac{1}{1+\mu}}} \frac{\partial W}{\partial v} \sum_{k=0}^{\infty} \left( -\frac{1}{2(1+\mu)} + \frac{\mu}{1+\mu} k \right) \frac{2k+1}{2\mu k-1} \left( W^{-\frac{2}{1+\mu}} \right)^k \quad (C3)$$

This formula works also for  $\mu=0$ . However, the  $\frac{\partial W}{\partial v}$  in front of the sum could indicate that the value of the derivative could be infinity for  $v=\pi/2$ , as there is the factor  $\cos^{2+\mu} v$  in the denominator of it (see eq. (74)). Nevertheless, if we make substitution according to (74) in all the terms containing  $W$ , we can see the following:

$$\begin{aligned} \frac{\partial x(v, R)}{\partial v} &= \frac{R}{1+\mu} \sum_{k=0}^{\infty} \left( -\frac{1}{2(1+\mu)} + \frac{\mu}{1+\mu} k \right) \frac{2k+1}{2\mu k-1} \frac{\partial W}{\partial v} W^{-\frac{2k}{1+\mu}-1-\frac{1}{1+\mu}} = \\ &= \frac{R}{1+\mu} \sum_{k=0}^{\infty} \left( -\frac{1}{2(1+\mu)} + \frac{\mu}{1+\mu} k \right) \frac{2k+1}{2\mu k-1} \frac{1+\mu \sin^2 v}{\cos^{2+\mu} v} \left( \frac{R}{R_0} \right)^{-\frac{2\mu k}{1+\mu}-\frac{\mu}{1+\mu}} \frac{(\sin v)^{-\frac{2k}{1+\mu}-1-\frac{1}{1+\mu}}}{(\cos v)^{-2k-(1+\mu)-1}} = \\ &= \frac{R}{1+\mu} \sum_{k=0}^{\infty} \left( -\frac{1}{2(1+\mu)} + \frac{\mu}{1+\mu} k \right) \frac{2k+1}{2\mu k-1} \frac{1+\mu \sin^2 v}{1} \left( \frac{R}{R_0} \right)^{-\frac{2\mu k}{1+\mu}-\frac{\mu}{1+\mu}} \frac{(\sin v)^{-\frac{2k}{1+\mu}-1-\frac{1}{1+\mu}}}{(\cos v)^{-2k}} \\ &= \frac{R}{1+\mu} \sum_{k=0}^{\infty} \left( -\frac{1}{2(1+\mu)} + \frac{\mu}{1+\mu} k \right) \frac{2k+1}{2\mu k-1} \left( \frac{R}{R_0} \right)^{-\frac{2\mu k}{1+\mu}-\frac{\mu}{1+\mu}} \frac{(1+\mu \sin^2 v) \cos^{2k} v}{(\sin v)^{\frac{2k}{1+\mu}+1+\frac{1}{1+\mu}}} \end{aligned} \quad (C4)$$

This has a finite value for  $v=\pi/2$ , equal to  $-R (R/R_0)^{-\frac{\mu}{1+\mu}}$ .

Nevertheless, the formula (C3) is not suitable for the further simplification of the metric scale factor formula for which the square of the derivative is needed. Neither Hagen-Rothe (Chu 2010, Chu 2013) nor Jensen (Gould 1972) combinatorial formulas could be employed due to the expression  $2k+1$  in the numerator of (C3). Therefore, the previous expression (C2) and rather a tedious approach (which first splits the expression into three parts) have to be used to proceed for the determination of the suitable shape of the square of the derivative:

$$\begin{aligned}
\left(\frac{\partial x(v, R)}{\partial v}\right)^2 &= \frac{1}{(1+\mu)^2} \left(\frac{R}{2}\right)^2 \frac{1}{\mu^2 W^{2+\frac{2}{1+\mu}}} \left(\frac{\partial W}{\partial v}\right)^2 \left\{ \sum_{k=0}^{\infty} \binom{-\frac{1}{2(1+\mu)} + \frac{\mu}{1+\mu}k}{k} \frac{\left(W^{-\frac{2}{1+\mu}}\right)^k}{-\frac{1}{2(1+\mu)} + \frac{\mu}{1+\mu}k} \right. \\
&\quad \left. + 2 \sum_{k=0}^{\infty} \binom{-\frac{1}{2(1+\mu)} + \frac{\mu}{1+\mu}k}{k} \left(W^{-\frac{2}{1+\mu}}\right)^k \right\}^2 \\
&= \frac{1}{(1+\mu)^2} \left(\frac{R}{2}\right)^2 \frac{1}{\mu^2 W^{2+\frac{2}{1+\mu}}} \left(\frac{\partial W}{\partial v}\right)^2 \left\{ \left[ \sum_{k=0}^{\infty} \binom{-\frac{1}{2(1+\mu)} + \frac{\mu}{1+\mu}k}{k} \frac{\left(W^{-\frac{2}{1+\mu}}\right)^k}{-\frac{1}{2(1+\mu)} + \frac{\mu}{1+\mu}k} \right] \right. \\
&\quad \left. + 2 \left[ \sum_{k=0}^{\infty} \binom{-\frac{1}{2(1+\mu)} + \frac{\mu}{1+\mu}k}{k} \frac{\left(W^{-\frac{2}{1+\mu}}\right)^k}{-\frac{1}{2(1+\mu)} + \frac{\mu}{1+\mu}k} \right] \left[ 2 \sum_{k=0}^{\infty} \binom{-\frac{1}{2(1+\mu)} + \frac{\mu}{1+\mu}k}{k} \left(W^{-\frac{2}{1+\mu}}\right)^k \right] \right. \\
&\quad \left. + \left[ 2 \sum_{k=0}^{\infty} \binom{\frac{1}{2(1+\mu)} - 1 + \frac{1}{1+\mu}k}{k} (-1)^k \left(W^{-\frac{2}{1+\mu}}\right)^k \right]^2 \right\}
\end{aligned} \tag{C5}$$

where the binomial identity (A3) was used in the third term. The Cauchy products are then used for the three terms:

$$\begin{aligned}
\left(\frac{\partial x(v, R)}{\partial v}\right)^2 &= \frac{1}{(1+\mu)^2} \left(\frac{R}{2}\right)^2 \frac{1}{\mu^2 W^{2+\frac{2}{1+\mu}}} \left(\frac{\partial W}{\partial v}\right)^2 \\
&\cdot \left\{ \left[ \sum_{k=0}^{\infty} \left(W^{-\frac{2}{1+\mu}}\right)^k \sum_{m=0}^k \frac{1}{-\frac{1}{2(1+\mu)} + \frac{\mu}{1+\mu}m} \binom{-\frac{1}{2(1+\mu)} + \frac{\mu}{1+\mu}m}{m} \frac{1}{-\frac{1}{2(1+\mu)} + \frac{\mu}{1+\mu}(k-m)} \binom{-\frac{1}{2(1+\mu)} + \frac{\mu}{1+\mu}(k-m)}{k-m} \right] \right. \\
&+ 4 \left[ \sum_{k=0}^{\infty} \left(W^{-\frac{2}{1+\mu}}\right)^k \sum_{m=0}^k \binom{-\frac{1}{2(1+\mu)} + \frac{\mu}{1+\mu}m}{m} \frac{1}{-\frac{1}{2(1+\mu)} + \frac{\mu}{1+\mu}m} \binom{-\frac{1}{2(1+\mu)} + \frac{\mu}{1+\mu}(k-m)}{k-m} \right] \\
&+ 4 \left[ \sum_{k=0}^{\infty} \left(-W^{-\frac{2}{1+\mu}}\right)^k \sum_{m=0}^k \binom{\frac{1}{2(1+\mu)} - 1 + \frac{1}{1+\mu}m}{m} \binom{\frac{1}{2(1+\mu)} - 1 + \frac{1}{1+\mu}(k-m)}{k-m} \right] \Big\}
\end{aligned} \tag{C6}$$

This operation is followed by the use of Hagen-Rothe ([Chu 2010, Chu 2013](#)) and Jensen ([Gould 1972](#)) identities in order to simplify the squared derivative:

$$\begin{aligned}
\left(\frac{\partial x(v, R)}{\partial v}\right)^2 &= \frac{1}{(1+\mu)^2} \left(\frac{R}{2}\right)^2 \frac{1}{\mu^2 W^{2+\frac{2}{1+\mu}}} \left(\frac{\partial W}{\partial v}\right)^2 \\
&\cdot \left\{ -4(1+\mu)^2 \sum_{k=0}^{\infty} \frac{1}{\mu k - 1} \binom{-\frac{1}{1+\mu} + \frac{\mu}{1+\mu}k}{k} \left(W^{-\frac{2}{1+\mu}}\right)^k \right. \\
&- 8 \sum_{k=0}^{\infty} (1+\mu) \binom{-\frac{1}{1+\mu} + \frac{\mu}{1+\mu}k}{k} \left(W^{-\frac{2}{1+\mu}}\right)^k \\
&+ 4 \sum_{k=0}^{\infty} \left[ \left(-W^{-\frac{2}{1+\mu}}\right)^k \sum_{m=0}^k \binom{\frac{1}{1+\mu} - 2 - \frac{\mu}{1+\mu}k + (k-m)}{k-m} \frac{1}{(1+\mu)^m} \right] \Bigg\} = \\
&= \left(\frac{R}{2}\right)^2 \frac{1}{\mu^2 W^{2+\frac{2}{1+\mu}}} \left(\frac{\partial W}{\partial v}\right)^2 \\
&\cdot \left\{ -4 \sum_{k=0}^{\infty} \frac{1}{\mu k - 1} \binom{-1 + \frac{\mu}{1+\mu}(k+1)}{k} \left(W^{-\frac{2}{1+\mu}}\right)^k \right. \\
&- \frac{8}{1+\mu} \sum_{k=0}^{\infty} \binom{-1 + \frac{\mu}{1+\mu}(k+1)}{k} \left(W^{-\frac{2}{1+\mu}}\right)^k \\
&+ \frac{4}{(1+\mu)^2} \sum_{k=0}^{\infty} \left[ \left(-W^{-\frac{2}{1+\mu}}\right)^k \sum_{m=0}^k \binom{-\frac{\mu}{1+\mu}(k+1) - 1 + m}{m} \frac{1}{(1+\mu)^{k-m}} \right] \Bigg\}
\end{aligned} \tag{C7}$$

where a reverse counting was used in the inner sum of the third term. For later use, it is advantageous to rewrite this expression using a substitution  $M=k+1$ ,

$$\begin{aligned}
\left(\frac{\partial x(v, R)}{\partial v}\right)^2 &= \left(\frac{R}{2}\right)^2 \frac{1}{\mu^2 W^{2+\frac{2}{1+\mu}}} \left(\frac{\partial W}{\partial v}\right)^2 \left\{ -4 \sum_{M=1}^{\infty} \frac{1}{\mu M - \mu - 1} \binom{\frac{\mu}{1+\mu}M - 1}{M-1} \left(W^{-\frac{2}{1+\mu}}\right)^{M-1} \right. \\
&- \frac{8}{1+\mu} \sum_{M=1}^{\infty} \binom{\frac{\mu}{1+\mu}M - 1}{M-1} \left(W^{-\frac{2}{1+\mu}}\right)^{M-1} \\
&+ \frac{4}{1+\mu} \sum_{M=1}^{\infty} \left[ \left(-W^{-\frac{2}{1+\mu}}\right)^{M-1} \sum_{m=0}^{M-1} \binom{-\frac{\mu}{1+\mu}M - 1 + m}{m} \frac{1}{(1+\mu)^{M-m}} \right] \Bigg\}
\end{aligned} \tag{C8}$$

Also for later use, and with the help of binomial identity  $\binom{\alpha-1}{k-1} = \binom{\alpha}{k} \frac{k}{\alpha}$ , it is of advantage to rewrite the expression to the form

$$\begin{aligned}
\left(\frac{\partial x(v, R)}{\partial v}\right)^2 &= \left(\frac{R}{2}\right)^2 \frac{1}{\mu^2 W^{2+\frac{2}{1+\mu}}} \left(\frac{\partial W}{\partial v}\right)^2 \left\{ -4 \frac{1+\mu}{\mu} \sum_{M=1}^{\infty} \frac{1}{\mu M - \mu - 1} \binom{\frac{\mu}{1+\mu} M}{M} \left(W^{-\frac{2}{1+\mu}}\right)^{M-1} \right. \\
&\quad - \frac{8}{\mu} \sum_{M=1}^{\infty} \binom{\frac{\mu}{1+\mu} M}{M} \left(W^{-\frac{2}{1+\mu}}\right)^{M-1} \\
&\quad + \frac{4}{1+\mu} \sum_{M=1}^{\infty} \left[ \left(-W^{-\frac{2}{1+\mu}}\right)^{M-1} \left( \sum_{m=0}^M \binom{-\frac{\mu}{1+\mu} M - 1 + m}{m} \frac{1}{(1+\mu)^{M-m}} \right. \right. \\
&\quad \left. \left. - \binom{-\frac{\mu}{1+\mu} M + M - 1}{M} \right) \right] \left. \right\} , \tag{C9}
\end{aligned}$$

where we also added and subtracted the term with  $m=M$  at the end of the third part, the inner sum, of the series. We further add and subtract the terms with  $M=0$  at the begin of the third series, arriving at the expression

$$\begin{aligned}
\left(\frac{\partial x(v, R)}{\partial v}\right)^2 &= \left(\frac{R}{2}\right)^2 \frac{1}{\mu^2 W^{2+\frac{2}{1+\mu}}} \left(\frac{\partial W}{\partial v}\right)^2 \left\{ -4 \frac{1+\mu}{\mu} \sum_{M=1}^{\infty} \frac{1}{\mu M - \mu - 1} \binom{\frac{\mu}{1+\mu} M}{M} \left(W^{-\frac{2}{1+\mu}}\right)^{M-1} \right. \\
&\quad - \frac{8}{\mu} \sum_{M=1}^{\infty} \binom{\frac{\mu}{1+\mu} M}{M} \left(W^{-\frac{2}{1+\mu}}\right)^{M-1} \\
&\quad + \frac{4}{1+\mu} \sum_{M=0}^{\infty} \left[ \left(-W^{-\frac{2}{1+\mu}}\right)^{M-1} \left( \sum_{m=0}^M \binom{-\frac{\mu}{1+\mu} M - 1 + m}{m} \frac{1}{(1+\mu)^{M-m}} - \binom{-\frac{\mu}{1+\mu} M + M - 1}{M} \right) \right] \left. \right\} . \tag{C10}
\end{aligned}$$

### ***Derivative of $z$ with respect to $v$***

Similarly, the partial derivative of  $z$  with respect to  $v$  in the **large- $v$  region** is obtained using eq. (A7c):

$$\begin{aligned}
\frac{\partial z(\nu, R)}{\partial \nu} &= \frac{\partial}{\partial \nu} \left\{ \frac{1}{(1+\mu)^{1/2}} \frac{R}{2} \sum_{k=0}^{\infty} \binom{-\frac{1}{2} + \frac{\mu}{1+\mu}k}{k} \frac{\left(W^{-\frac{2}{1+\mu}}\right)^k}{-\frac{1}{2} + \frac{\mu}{1+\mu}k} \right\} \\
&= \frac{1}{(1+\mu)^{1/2}} \frac{R}{2} \frac{\partial}{\partial \nu} \left\{ W^{-\frac{1}{\mu}} \frac{R}{2} \sum_{k=0}^{\infty} \binom{-\frac{1}{2} + \frac{\mu}{1+\mu}k}{k} \frac{\left(W^{\frac{1}{\mu}}\right)^{-\frac{2\mu}{1+\mu}k+1}}{\frac{1}{2} - \frac{\mu}{1+\mu}k} \right\} \\
&= \frac{1}{(1+\mu)^{1/2}} \frac{R}{2} \left\{ \left[ \frac{\partial}{\partial \nu} \left( W^{-\frac{1}{\mu}} \right) \sum_{k=0}^{\infty} \binom{-\frac{1}{2} + \frac{\mu}{1+\mu}k}{k} \frac{\left(W^{\frac{1}{\mu}}\right)^{-\frac{2\mu}{1+\mu}k+1}}{\frac{1}{2} - \frac{\mu}{1+\mu}k} \right] \right. \\
&\quad \left. + \left[ W^{-\frac{1}{\mu}} \sum_{k=0}^{\infty} \binom{-\frac{1}{2} + \frac{\mu}{1+\mu}k}{k} \frac{\frac{\partial}{\partial \nu} \left( \left(W^{\frac{1}{\mu}}\right)^{-\frac{2\mu}{1+\mu}k+1} \right)}{\frac{1}{2} - \frac{\mu}{1+\mu}k} \right] \right\} = \\
&= \frac{1}{(1+\mu)^{1/2}} \frac{R}{2} \left\{ \left( W^{\frac{1}{\mu}} \right) \frac{\partial}{\partial \nu} \left( W^{-\frac{1}{\mu}} \right) \sum_{k=0}^{\infty} \binom{-\frac{1}{2} + \frac{\mu}{1+\mu}k}{k} \frac{\left(W^{\frac{1}{\mu}}\right)^{-\frac{2\mu}{1+\mu}k}}{\frac{1}{2} - \frac{\mu}{1+\mu}k} \right. \\
&\quad \left. + W^{-\frac{1}{\mu}} \frac{\partial}{\partial \nu} \left( W^{\frac{1}{\mu}} \right) \sum_{k=0}^{\infty} \binom{-\frac{1}{2} + \frac{\mu}{1+\mu}k}{k} \frac{\left(-\frac{2\mu}{1+\mu}k+1\right) \left(W^{\frac{1}{\mu}}\right)^{-\frac{2\mu}{1+\mu}k}}{\frac{1}{2} - \frac{\mu}{1+\mu}k} \right\} = \\
&= \frac{1}{(1+\mu)^{1/2}} \frac{R}{2} \frac{1}{\mu W} \frac{\partial W}{\partial \nu} \left\{ \sum_{k=0}^{\infty} \binom{-\frac{1}{2} + \frac{\mu}{1+\mu}k}{k} \frac{\left(W^{-\frac{2}{1+\mu}}\right)^k}{-\frac{1}{2} + \frac{\mu}{1+\mu}k} \right. \\
&\quad \left. + 2 \sum_{k=0}^{\infty} \binom{-\frac{1}{2} + \frac{\mu}{1+\mu}k}{k} \left(W^{-\frac{2}{1+\mu}}\right)^k \right\}
\end{aligned} \tag{C11}$$

The terms in sums in (C11) with the same binomial coefficients can be put together and then the derivative reads

$$\begin{aligned}
\frac{\partial z(\nu, R)}{\partial \nu} &= \frac{R}{(1+\mu)^{1/2}} \frac{1}{W} \frac{\partial W}{\partial \nu} \sum_{k=0}^{\infty} \binom{-\frac{1}{2} + \frac{\mu}{1+\mu}k}{k} \frac{\frac{1}{1+\mu}k}{-\frac{1}{2} + \frac{\mu}{1+\mu}k} \left(W^{-\frac{2}{1+\mu}}\right)^k \\
&= \frac{R}{(1+\mu)^{1/2}} \frac{1}{W} \frac{\partial W}{\partial \nu} \sum_{k=1}^{\infty} \binom{-\frac{1}{2} + \frac{\mu}{1+\mu}k}{k} \frac{2k}{2\mu k - \mu - 1} \left(W^{-\frac{2}{1+\mu}}\right)^k
\end{aligned} \tag{C12}$$

This formula works also for  $\mu=0$ .

However, the  $\partial W / \partial v$  in front of the sum could indicate that the value of the derivative could be infinity for  $v=\pi/2$ , as there is the factor  $\cos^{2+\mu} v$  in the denominator of  $\partial W / \partial v$  (see Eq. (74)). Nevertheless, if we make substitution according to (74) in all the terms with  $W$ , we can see the following:

$$\begin{aligned}
\frac{\partial z(v, R)}{\partial v} &= \frac{R}{(1+\mu)^{1/2}} \sum_{k=1}^{\infty} \binom{-\frac{1}{2} + \frac{\mu}{1+\mu}k}{k} \frac{2k}{2\mu k - \mu - 1} \frac{\partial W}{\partial v} W^{-\frac{2k}{1+\mu}-1} = \\
&= \frac{R}{(1+\mu)^{1/2}} \sum_{k=1}^{\infty} \binom{-\frac{1}{2} + \frac{\mu}{1+\mu}k}{k} \frac{2k}{2\mu k - \mu - 1} \frac{1 + \mu \sin^2 v}{\cos^{2+\mu} v} \left( \frac{R}{R_0} \right)^{-\frac{2\mu k}{1+\mu}} \frac{(\sin v)^{-\frac{2k}{1+\mu}-1}}{(\cos v)^{-2k-(1+\mu)}} = \\
&= \frac{R}{(1+\mu)^{1/2}} \sum_{k=1}^{\infty} \binom{-\frac{1}{2} + \frac{\mu}{1+\mu}k}{k} \frac{2k}{2\mu k - \mu - 1} \frac{1 + \mu \sin^2 v}{1} \left( \frac{R}{R_0} \right)^{-\frac{2\mu k}{1+\mu} - \frac{\mu}{1+\mu}} \frac{(\sin v)^{-\frac{2k}{1+\mu}-1}}{(\cos v)^{-2k+1}} = \\
&= \frac{R}{(1+\mu)^{1/2}} \sum_{k=1}^{\infty} \binom{-\frac{1}{2} + \frac{\mu}{1+\mu}k}{k} \frac{2k}{2\mu k - \mu - 1} \left( \frac{R}{R_0} \right)^{-\frac{2\mu k}{1+\mu} - \frac{\mu}{1+\mu}} \frac{(1 + \mu \sin^2 v) \cos^{2k-1} v}{(\sin v)^{\frac{2k}{1+\mu}+1}} =
\end{aligned} \tag{C13}$$

This has a finite value for  $v=\pi/2$ , equal to 0.

For the metric scale factor calculation, which is to be carried out later, also the square of the derivative is needed. For further simplification, the (C11) expression of the derivative is best suited to proceed:

$$\begin{aligned}
\left( \frac{\partial z(v, R)}{\partial v} \right)^2 &= \frac{1}{1+\mu} \left( \frac{R}{2} \right)^2 \frac{1}{\mu^2 W^2} \left( \frac{\partial W}{\partial v} \right)^2 \left\{ \sum_{k=0}^{\infty} \binom{-\frac{1}{2} + \frac{\mu}{1+\mu}k}{k} \frac{\left( W^{-\frac{2}{1+\mu}} \right)^k}{-\frac{1}{2} + \frac{\mu}{1+\mu}k} \right. \\
&\quad \left. + 2 \sum_{k=0}^{\infty} \binom{-\frac{1}{2} + \frac{\mu}{1+\mu}k}{k} \left( W^{-\frac{2}{1+\mu}} \right)^k \right\}^2 = \\
&= \frac{1}{1+\mu} \left( \frac{R}{2} \right)^2 \frac{1}{\mu^2 W^2} \left( \frac{\partial W}{\partial v} \right)^2 \left\{ \left[ \sum_{k=0}^{\infty} \binom{-\frac{1}{2} + \frac{\mu}{1+\mu}k}{k} \frac{\left( W^{-\frac{2}{1+\mu}} \right)^k}{-\frac{1}{2} + \frac{\mu}{1+\mu}k} \right]^2 \right. \\
&\quad \left. + 2 \left[ \sum_{k=0}^{\infty} \binom{-\frac{1}{2} + \frac{\mu}{1+\mu}k}{k} \frac{\left( W^{-\frac{2}{1+\mu}} \right)^k}{-\frac{1}{2} + \frac{\mu}{1+\mu}k} \right] \left[ 2 \sum_{k=0}^{\infty} \binom{-\frac{1}{2} + \frac{\mu}{1+\mu}k}{k} \left( W^{-\frac{2}{1+\mu}} \right)^k \right] \right. \\
&\quad \left. + \left[ 2 \sum_{k=0}^{\infty} \binom{-\frac{1}{2} + \frac{\mu}{1+\mu}k}{k} (-1)^k \left( W^{-\frac{2}{1+\mu}} \right)^k \right]^2 \right\}
\end{aligned} \tag{C14}$$

where the binomial identity (A3) was used in the third term.

The Cauchy products are then used for the three terms:

$$\begin{aligned}
& \left( \frac{\partial z(v, R)}{\partial v} \right)^2 = \\
& = \frac{1}{1+\mu} \left( \frac{R}{2} \right)^2 \frac{1}{\mu^2 W^2} \left( \frac{\partial W}{\partial v} \right)^2 \left\{ \left[ \sum_{k=0}^{\infty} \left( W^{-\frac{2}{1+\mu}} \right)^k \sum_{m=0}^k \frac{1}{-\frac{1}{2} + \frac{\mu}{1+\mu} m} \binom{-\frac{1}{2} + \frac{\mu}{1+\mu} m}{m} \frac{1}{-\frac{1}{2} + \frac{\mu}{1+\mu} (k-m)} \binom{-\frac{1}{2} + \frac{\mu}{1+\mu} (k-m)}{k-m} \right] \right. \\
& + 4 \left[ \sum_{k=0}^{\infty} \left( W^{-\frac{2}{1+\mu}} \right)^k \sum_{m=0}^k \binom{-\frac{1}{2} + \frac{\mu}{1+\mu} m}{m} \frac{1}{-\frac{1}{2} + \frac{\mu}{1+\mu} m} \binom{-\frac{1}{2} + \frac{\mu}{1+\mu} (k-m)}{k-m} \right] \\
& \left. + 4 \left[ \sum_{k=0}^{\infty} \left( -W^{-\frac{2}{1+\mu}} \right)^k \sum_{m=0}^k \binom{-\frac{1}{2} + \frac{1}{1+\mu} m}{m} \binom{-\frac{1}{2} + \frac{1}{1+\mu} (k-m)}{k-m} \right] \right\} \quad (C15)
\end{aligned}$$

This operation is followed by the use of Hagen-Rothe (Chu 2010, Chu 2013) and Jensen (Gould 1972) identities in order to simplify the squared derivative:

$$\begin{aligned}
& \left( \frac{\partial z(v, R)}{\partial v} \right)^2 = \frac{1}{1+\mu} \left( \frac{R}{2} \right)^2 \frac{1}{\mu^2 W^2} \left( \frac{\partial W}{\partial v} \right)^2 \left\{ -4 \sum_{k=0}^{\infty} \frac{1}{-1 + \frac{\mu}{1+\mu} k} \binom{-1 + \frac{\mu}{1+\mu} k}{k} \left( W^{-\frac{2}{1+\mu}} \right)^k \right. \\
& - 8 \sum_{k=0}^{\infty} \binom{-1 + \frac{\mu}{1+\mu} k}{k} \left( W^{-\frac{2}{1+\mu}} \right)^k \\
& + 4 \sum_{k=0}^{\infty} \left[ -(-1)^{k-1} \left( W^{-\frac{2}{1+\mu}} \right)^k \sum_{m=0}^k \binom{-\frac{\mu}{1+\mu} k - 1 + (k-m)}{k-m} \frac{1}{(1+\mu)^m} \right] \Bigg\} = \\
& = \frac{1}{1+\mu} \left( \frac{R}{2} \right)^2 \frac{1}{\mu^2 W^{2+\frac{2}{1+\mu}}} \left( \frac{\partial W}{\partial v} \right)^2 \left\{ -4 \sum_{k=0}^{\infty} \frac{1}{-1 + \frac{\mu}{1+\mu} k} \binom{-1 + \frac{\mu}{1+\mu} k}{k} \left( W^{-\frac{2}{1+\mu}} \right)^{k-1} \right. \\
& - 8 \sum_{k=0}^{\infty} \binom{-1 + \frac{\mu}{1+\mu} k}{k} \left( W^{-\frac{2}{1+\mu}} \right)^{k-1} \\
& \left. - 4 \sum_{k=0}^{\infty} \left[ (-1)^{k-1} \left( W^{-\frac{2}{1+\mu}} \right)^{k-1} \sum_{m=0}^k \binom{-\frac{\mu}{1+\mu} k - 1 + m}{m} \frac{1}{(1+\mu)^{k-m}} \right] \right\} \quad (C16)
\end{aligned}$$

where reverse counting was used in the inner sum of the third term.

For later use, and with the help of binomial identity  $\binom{\alpha-1}{k} = \binom{\alpha}{k} \frac{\alpha-k}{\alpha}$  (which can be, however, used only when  $\alpha \neq 0$  and, therefore, some terms with  $k=0$  have to be treated separately), it is of advantage to rewrite the expression to the form

$$\begin{aligned}
\left(\frac{\partial z(v, R)}{\partial v}\right)^2 &= \frac{1}{1+\mu} \left(\frac{R}{2}\right)^2 \frac{1}{\mu^2 W^{2+\frac{2}{1+\mu}}} \left(\frac{\partial W}{\partial v}\right)^2 \left\{ -4 \sum_{k=1}^{\infty} \frac{1}{-1+\frac{\mu}{1+\mu}k} \binom{-1+\frac{\mu}{1+\mu}k}{k} \left(W^{-\frac{2}{1+\mu}}\right)^{k-1} + \frac{4}{W^{-\frac{2}{1+\mu}}} \right. \\
&\quad - 8 \sum_{k=1}^{\infty} \binom{-1+\frac{\mu}{1+\mu}k}{k} \left(W^{-\frac{2}{1+\mu}}\right)^{k-1} - \frac{8}{W^{-\frac{2}{1+\mu}}} \\
&\quad \left. - 4 \sum_{k=0}^{\infty} \left[ (-1)^{k-1} \left(W^{-\frac{2}{1+\mu}}\right)^{k-1} \sum_{m=0}^k \binom{-\frac{\mu}{1+\mu}k-1+m}{m} \frac{1}{(1+\mu)^{k-m}} \right] \right\} = \\
&= \frac{1}{1+\mu} \left(\frac{R}{2}\right)^2 \frac{1}{\mu^2 W^{2+\frac{2}{1+\mu}}} \left(\frac{\partial W}{\partial v}\right)^2 \left\{ \frac{4}{\mu} \sum_{k=1}^{\infty} \frac{1}{-1+\frac{\mu}{1+\mu}k} \binom{\frac{\mu}{1+\mu}k}{k} \left(W^{-\frac{2}{1+\mu}}\right)^{k-1} + \frac{4}{W^{-\frac{2}{1+\mu}}} \right. \\
&\quad + \frac{8}{\mu} \sum_{k=1}^{\infty} \binom{\frac{\mu}{1+\mu}k}{k} \left(W^{-\frac{2}{1+\mu}}\right)^{k-1} - \frac{8}{W^{-\frac{2}{1+\mu}}} \\
&\quad \left. - 4 \sum_{k=0}^{\infty} \left[ (-1)^{k-1} \left(W^{-\frac{2}{1+\mu}}\right)^{k-1} \sum_{m=0}^k \binom{-\frac{\mu}{1+\mu}k-1+m}{m} \frac{1}{(1+\mu)^{k-m}} \right] \right\} .
\end{aligned} \tag{C17}$$
