# Supplementary material for: Analytical Solution of Similar Oblate Spheroidal Coordinate System
Source: arXiv:2109.12057 ancillary file (2021-09-06)
Supplement: Supplementary file 3 [file Supplement_SOS_D.pdf]

# Analytical solution of Similar Oblate Spheroidal Coordinate System

---

Pavel Strunz

Nuclear Physics Institute of the CAS, Řež, Czech Republic

e-mail: strunz@ujf.cas.cz

## Supplement D

### Metric scale factors derivation

When derivatives are known, we have all means to calculate the scale factors of SOS coordinates according to Eq. (16). We have, however, to calculate it separately in the small- and in the large- $\nu$  regions.

#### *Small- $\nu$ region, $h_R$ metric scale factor*

For the derivation of  $h_R$ , Eqs. (66) and (67) are used. When the derivatives are input to the basic equation (16), we obtain

$$\begin{aligned} h_R &= \sqrt{\left(\frac{\partial x(\nu, R)}{\partial R}\right)^2 + \left(\frac{\partial z(\nu, R)}{\partial R}\right)^2} = \\ &= \sqrt{\left(\sum_{k=0}^{\infty} \left(-\frac{1}{2} + (1+\mu)k\right) \binom{\mu-1}{k} (-W^2)^k\right)^2 + \left(W(1+\mu)^{1/2} \sum_{k=0}^{\infty} \left(\frac{\mu-1}{2} + (1+\mu)k\right) \binom{\mu-1}{k} (-W^2)^k\right)^2} \end{aligned} \quad (D1)$$

When applying the Cauchy product formula to the squares of the individual derivatives, we obtain

$$\begin{aligned} h_R &= \left[ \sum_{k=0}^{\infty} (-W^2)^k \sum_{m=0}^k \left(-\frac{1}{2} + (1+\mu)m\right) \binom{\mu-1}{m} \left(-\frac{1}{2} + (1+\mu)(k-m)\right) \binom{\mu-1}{k-m} \right. \\ &\quad \left. + W^2(1+\mu) \sum_{k=0}^{\infty} (-W^2)^k \sum_{m=0}^k \left(\frac{\mu-1}{2} + (1+\mu)m\right) \binom{\mu-1}{m} \left(\frac{\mu-1}{2} + (1+\mu)(k-m)\right) \binom{\mu-1}{k-m} \right]^{\frac{1}{2}} \end{aligned} \quad (D2)$$

Using Jensen combinatorial formula (listed as No 3.144 in [Gould 1972](#)), we can simplify this to

$$\begin{aligned} h_R &= \left[ \sum_{k=0}^{\infty} (-W^2)^k \sum_{m=0}^k \binom{\mu k - 1 + (k-m)}{k-m} (1+\mu)^m \right. \\ &\quad \left. + W^2(1+\mu) \sum_{k=0}^{\infty} (-W^2)^k \sum_{m=0}^k \binom{\mu(k+1) - 1 + (k-m)}{k-m} (1+\mu)^m \right]^{\frac{1}{2}} \end{aligned}$$

(D3)

Using reverse counting in the inner sums, we have

$$h_R = \left[ \sum_{k=0}^{\infty} (-W^2)^k \sum_{m=0}^k \binom{\mu k - 1 + m}{m} (1 + \mu)^{k-m} + W^2(1 + \mu) \sum_{k=0}^{\infty} (-W^2)^k \sum_{m=0}^k \binom{\mu(k+1) - 1 + m}{m} (1 + \mu)^{k-m} \right]^{\frac{1}{2}} \quad (D4)$$

Now, substitution  $K=k+1$  can be used in the second term inside the square root, followed by adding and subtracting terms at the end and begin of the series, and resulting in its following shape:

$$\begin{aligned} W^2(1 + \mu) \sum_{K=1}^{\infty} (-W^2)^{K-1} \sum_{m=0}^{K-1} \binom{\mu K - 1 + m}{m} (1 + \mu)^{K-1-m} &= \\ &= - \sum_{K=1}^{\infty} (-W^2)^K \sum_{m=0}^{K-1} \binom{\mu K - 1 + m}{m} (1 + \mu)^{K-m} = \\ &= - \sum_{K=1}^{\infty} (-W^2)^K \left[ \sum_{m=0}^K \binom{\mu K - 1 + m}{m} (1 + \mu)^{K-m} - \binom{(\mu + 1)K - 1}{K} \right] = \\ &= - \sum_{K=0}^{\infty} (-W^2)^K \sum_{m=0}^K \binom{\mu K - 1 + m}{m} (1 + \mu)^{K-m} + 1 + \sum_{K=1}^{\infty} (-W^2)^K \binom{(\mu + 1)K - 1}{K} \end{aligned} \quad (D5)$$

where we employed the fact that anything calling zero in binomial coefficient is equal to one. Now, it can be recognized, that the left double sum is equal to the first term in (D4) but having an opposite sign.

Therefore,  $h_R$  equals to

$$h_R = \sqrt{1 + \sum_{K=1}^{\infty} (-W^2)^K \binom{(\mu + 1)K - 1}{K}} = \sqrt{\sum_{k=0}^{\infty} \binom{(\mu + 1)k - 1}{k} (-W^2)^k} \quad (D6)$$

When using the right-hand side binomial identity of (A3), we finally arrive at

$$h_R = \sqrt{\sum_{k=0}^{\infty} \binom{-\mu k}{k} (W^2)^k} \quad (D7)$$

The expression can be also directly used in case  $\nu=0$  (equatorial plane), i.e. when  $W$  equals 0. In that case  $h_R(\nu = 0) = 1$  (D8)

An immediate partial test of the validity of (D7) can be carried out for parameter  $\mu$  equal to 0 (spherical coordinate system) or  $\mu$  equal to 1, for which the solution of Eq. (8) can be still obtained also in a closed form.

The case of parameter  $\mu=0$  is trivial: all the binomial coefficients in (D7) are zero except the one for  $k=0$ , which is equal to 1. Then,  $h_R$  is equal to 1, which is a correct result for spherical coordinates.

In the particular case of parameter  $\mu=1$ , (D6) can be used to derive  $h_R$  in the following way:

$$h_R = \sqrt{\sum_{k=0}^{\infty} \binom{2k-1}{k} (-W^2)^k} = \sqrt{\frac{1}{\sqrt{1-4(-W)^2}} \left( \frac{1-\sqrt{1-4(-W)^2}}{2(-W)^2} \right)^{-1}} = \sqrt{\frac{2W^2}{1+4W^2-\sqrt{1+4W^2}}} \quad (D9)$$

where we used the well-known (Seiden 1994) closed form of the infinite series  $\sum_{k=0}^{\infty} \binom{2k+\alpha}{k} y^k$ . On the other hand, a closed-form solution of the equation (23) with  $\mu=1$

$$W^2 s^4 + s^2 - 1 = 0 \quad (D10)$$

where  $s=x/R$ , is

$$s^2 = \frac{-1 \pm \sqrt{1+4W^2}}{2W^2} \Rightarrow x = R \sqrt{\frac{-1 \pm \sqrt{1+4W^2}}{2W^2}} \quad \text{and (see (16))} \quad z = \frac{W}{(1+\mu)^{1/2} R^\mu} x^{1+\mu} = \frac{WR}{\sqrt{2}} \cdot \frac{-1 \pm \sqrt{1+4W^2}}{2W^2} \quad (D11)$$

where  $W$  is given by

$$W = \frac{R}{R_0} \frac{\sin v}{\cos^2 v} = RC \quad , \quad (D12)$$

Therefore, the derivatives are

$$\frac{\partial x(v, R)}{\partial R} = \frac{RC}{\sqrt{2R^2 C^2 + \frac{1}{2}} \sqrt{\sqrt{4R^2 C^2 + 1} - 1}} \quad \text{and} \quad \frac{\partial z(v, R)}{\partial R} = \frac{\sqrt{2} RC}{\sqrt{4R^2 C^2 + 1}} \quad (D13)$$

The metric scale factor for  $\mu=1$  is then

$$\begin{aligned} h_R &= \sqrt{\left( \frac{\partial x(v, R)}{\partial R} \right)^2 + \left( \frac{\partial z(v, R)}{\partial R} \right)^2} = \sqrt{\frac{R^2 C^2}{(2R^2 C^2 + \frac{1}{2}) (\sqrt{4R^2 C^2 + 1} - 1)} + \frac{2R^2 C^2}{4R^2 C^2 + 1}} \\ &= \sqrt{\frac{2W^2 + 2W^2 \sqrt{4W^2 + 1} - 2W^2}{(4W^2 + 1) (\sqrt{4W^2 + 1} - 1)}} = \sqrt{\frac{2W^2}{\sqrt{(4W^2 + 1)} (\sqrt{4W^2 + 1} - 1)}} \\ &= \sqrt{\frac{2W^2}{(4W^2 + 1) - \sqrt{(4W^2 + 1)}}} \quad , \quad (D14) \end{aligned}$$

which is identical with the solution (D9) found using power series.

The closed-form solution of the equation (23) is also possible for  $\mu=2$ . We state it here without a detailed derivation:

$$x = R \sqrt{\frac{-2}{\sqrt{3}W}} \sinh \left( \frac{1}{3} \operatorname{arsinh} \frac{-3\sqrt{3}}{2} W \right) \quad (D15)$$

The metric scale factor  $h_R$  is (again without a detailed derivation) then equal to

$$h_R = \sqrt{\frac{\sqrt{3}W}{\frac{27}{2}W^2 + 2} \cdot \frac{\cosh^2 A \cosh 2A}{\sinh A}} \quad , \quad \text{where} \quad A = \frac{1}{3} \operatorname{arsinh} \frac{3\sqrt{3}}{2} W \quad (D16)$$

At the same time, this solution has to be equal to the solution (D7) with  $\mu=2$ . In this way, a new combinatorial identity is derived:

$$\sum_{k=0}^{\infty} \binom{-2k}{k} (W^2)^k = \sum_{k=0}^{\infty} \binom{3k-1}{k} (-W^2)^k = \frac{\sqrt{3}W}{\frac{27}{2}W^2 + 2} \cdot \frac{\cosh^2 A \cosh 2A}{\sinh A} \quad (D17)$$

Further, (D6) form of  $h_R$  can be transformed to a form where the sum is in denominator. For this purpose, the Pólya and Szegő identity listed under Nr. 1.120 in [Gould 1972](#)] is used. Then

$$h_R = \sqrt{\sum_{k=0}^{\infty} \binom{(\mu+1)k-1}{k} (-W^2)^k} = \sqrt{\frac{p^{-1+1}}{(1-(1+\mu)p + (1+\mu))}} \quad \text{where} \quad -W^2 = \frac{p-1}{p^{1+\mu}} \quad (D18)$$

Then the expression for  $p$  is then

$$W^2 p^{1+\mu} + p = 1 \quad , \quad (D19)$$

resembles (9) and the solution for  $p$  can be thus obtained using (10). Then, we can write for  $h_R$

$$\begin{aligned} h_R &= \frac{1}{\sqrt{(1+\mu) - \mu p}} = \left[ (1+\mu) - \mu \sum_{k=0}^{\infty} \binom{1+(1+\mu)k}{k} \frac{(-W^2)^k}{1+(1+\mu)k} \right]^{-\frac{1}{2}} \\ &= \left[ (1+\mu) + \mu \sum_{k=0}^{\infty} \binom{-\mu k - 1}{k} \frac{(W^2)^k}{-\mu k - 1} \right]^{-\frac{1}{2}} \end{aligned} \quad (D20)$$

where the last expression comes from the identity (A3).

### ***Small- $v$ region, $h_v$ metric scale factor***

For the derivation of  $h_v$ , Eqs. (72) and (73) are employed:

$$\begin{aligned} h_v &= \sqrt{\left( \frac{\partial x(v, R)}{\partial v} \right)^2 + \left( \frac{\partial z(v, R)}{\partial v} \right)^2} \\ &= \frac{R}{2} \frac{1}{\mu} \left( \frac{\partial W}{\partial v} \right) \left\{ -4 \frac{\mu+1}{\mu} \sum_{k=1}^{\infty} \frac{1}{-\mu k - 1} \binom{-\mu k}{k} (W^2)^{k-1} + \frac{4}{W^2} \right. \\ &\quad - 8 \frac{\mu+1}{\mu} \sum_{k=1}^{\infty} \binom{-\mu k}{k} (W^2)^{k-1} - \frac{8}{W^2} \\ &\quad - 4 \sum_{k=0}^{\infty} \left[ (-W^2)^{k-1} \sum_{m=0}^k \binom{\mu k - 1 + m}{m} (1+\mu)^{k-m} \right] + \frac{4}{\mu} \sum_{M=1}^{\infty} \frac{1}{-\mu M - 1} \binom{-\mu M}{M} (W^2)^{M-1} \\ &\quad + \frac{8}{\mu} \sum_{M=1}^{\infty} \binom{-\mu M}{M} (W^2)^{M-1} + 4 \sum_{M=0}^{\infty} \left[ (-W^2)^{M-1} \sum_{m=0}^M \binom{\mu M - 1 + m}{m} (1+\mu)^{M-m} \right] \\ &\quad \left. + 4 \sum_{M=0}^{\infty} (W^2)^{M-1} \binom{-\mu M}{M} \right\}^{\frac{1}{2}} , \end{aligned} \quad (D21)$$

where we used the identity (A3) in the very last term. When we combine the similar terms, we get

$$\begin{aligned}
h_v &= \frac{R}{2} \frac{1}{\mu} \left( \frac{\partial W}{\partial v} \right) \left\{ -4 \sum_{k=1}^{\infty} \frac{1}{-\mu k - 1} \binom{-\mu k}{k} (W^2)^{k-1} + \frac{4}{W^2} - 8 \sum_{k=1}^{\infty} \binom{-\mu k}{k} (W^2)^{k-1} - \frac{8}{W^2} \right. \\
&\quad \left. + 4 \sum_{M=0}^{\infty} (W^2)^{M-1} \binom{-\mu M}{M} \right\}^{\frac{1}{2}} \\
&= \frac{R}{2} \frac{1}{\mu} \left( \frac{\partial W}{\partial v} \right) \left\{ -4 \sum_{k=0}^{\infty} \frac{1}{-\mu k - 1} \binom{-\mu k}{k} (W^2)^{k-1} - 8 \sum_{k=0}^{\infty} \binom{-\mu k}{k} (W^2)^{k-1} \right. \\
&\quad \left. + 4 \sum_{M=0}^{\infty} \binom{-\mu M}{M} (W^2)^{M-1} \right\}^{\frac{1}{2}} \\
&= \frac{R}{2} \frac{1}{\mu} \left( \frac{\partial W}{\partial v} \right) \left\{ -4 \sum_{k=0}^{\infty} \frac{1}{-\mu k - 1} \binom{-\mu k}{k} (W^2)^{k-1} - 4 \sum_{k=0}^{\infty} \binom{-\mu k}{k} (W^2)^{k-1} \right\}^{\frac{1}{2}} \\
&= R \frac{1}{\mu W} \left( \frac{\partial W}{\partial v} \right) \left\{ - \sum_{k=0}^{\infty} \frac{\mu k}{\mu k + 1} \binom{-\mu k}{k} (W^2)^k \right\}^{\frac{1}{2}}
\end{aligned} \tag{D22}$$

Then

$$h_v = R \frac{1}{\mu} \left( \frac{\partial W}{\partial v} \right) \sqrt{ - \sum_{k=1}^{\infty} \frac{\mu k}{\mu k + 1} \binom{-\mu k}{k} (W^2)^{k-1} } \tag{D23}$$

This formula can be used for  $\mu > 0$  (and in principle also for  $-1 < \mu < 0$ , except certain cases). For the limit  $\mu \rightarrow 0$ ,  $h_v$  should be finite, and, moreover, equal to  $R$  as the SOS coordinate system is equal to spherical coordinate system for  $\mu = 0$ . However, it cannot be directly seen from the formula (D23). Therefore, it is useful to rewrite this formula also to another shape using (A3) identity (its left hand side). Then

$$\begin{aligned}
h_v &= R \frac{1}{\mu} \frac{\partial W}{\partial v} \sqrt{ - \sum_{k=1}^{\infty} \frac{\mu k}{\mu k + 1} \cdot \frac{\mu k}{\mu k + k} (-1)^k \binom{\mu k + k}{k} (W^2)^{k-1} } \\
&= R \frac{\partial W}{\partial v} \sqrt{ \sum_{k=1}^{\infty} \frac{k}{(\mu k + 1)(\mu + 1)} \binom{(\mu + 1)k}{k} (-W^2)^{k-1} }
\end{aligned} \tag{D24}$$

which for  $\mu = 0$  equals to

$$h_v = R \frac{\partial W}{\partial v} \sqrt{ \sum_{k=1}^{\infty} k \binom{k}{k} (-W^2)^{k-1} } = R \frac{\partial W}{\partial v} \sqrt{ \frac{1}{-W^2} \frac{-W^2}{(1 + W^2)^2} } = R \frac{1}{\cos^2 v} \sqrt{ \frac{1}{\left( 1 + \frac{\sin^2 v}{\cos^2 v} \right)^2} } = R \tag{D25}$$

Above, we used the identity  $\binom{k}{k} = 1$ , the well-known closed form of the infinite series  $\sum_{k=1}^{\infty} k y^k = y/(1 - y)^2$ , and the formulas (74) for  $W$  and its derivative with  $\mu = 0$ . It can be seen, that the result equals to the one valid for spherical coordinates.

Further potential restriction with (D24) expression is that  $\mu$  cannot be equal to  $-1/2$ ,  $-1/3$ ,  $-1/4$  etc. as the denominator would then equal to zero for certain  $k$  (particularly for  $k = -1/\mu$ ) in these cases. This can

happen for certain prolate ellipsoidal coordinate systems (where  $-1 < \mu < 0$ ), for which the derived expressions could be possibly used as well. Nevertheless, also the binomial coefficient in (D24) goes to zero in these cases, and the limit of  $h_v$  is then finite. Only a proper expression has to be found. For its derivation, we use the binomial identities (A3) and (A4). With its help, (D24) formula can be rewritten into the form

$$h_v = \frac{R}{\sqrt{1+\mu}} \frac{\partial W}{\partial v} \sqrt{\sum_{k=1}^{\infty} \binom{(1+\mu)k}{k-1} (-W^2)^{k-1}} \quad , \quad (D26)$$

or even

$$h_v = \frac{R}{\sqrt{1+\mu}} \frac{\partial W}{\partial v} \sqrt{\sum_{M=0}^{\infty} \binom{(1+\mu)(M+1)}{M} (-W^2)^M} \quad , \quad (D27)$$

or even (with help of (A3) to

$$h_v = \frac{R}{\sqrt{1+\mu}} \frac{\partial W}{\partial v} \sqrt{\sum_{k=0}^{\infty} \binom{-\mu(k+1)-2}{k} (W^2)^k} \quad , \quad (D28)$$

where the terms with  $W$  are determined by Eq. (74). This formula can be directly used also in the abovementioned cases when  $\mu = -\frac{1}{2}, -\frac{1}{3}, -\frac{1}{4}$  etc. The expression can be also directly used in case  $v=0$  (equatorial plane), i.e. when  $W$  equals 0. In that case

$$h_v(v=0) = \frac{R}{\sqrt{1+\mu}} \frac{\partial W}{\partial v} = \frac{R}{\sqrt{1+\mu}} \left( \frac{R}{R_0} \right)^{\mu} \quad . \quad (D29)$$

The convergence limit of the power series has to be tested as well. We use the root test

$$\begin{aligned} 1 &> \limsup_{k \rightarrow \infty} \sqrt[k]{\left| \binom{(1+\mu)k}{k-1} \cdot (-W^2)^{k-1} \right|} = \limsup_{k \rightarrow \infty} \sqrt[k]{\left| \binom{(1+\mu)k}{k-1} \right|} (W^2)^{1-\frac{1}{k}} \\ &= \limsup_{k \rightarrow \infty} \sqrt[k]{\left| \frac{k}{(1+\mu)k+1-k} \binom{(1+\mu)k}{k} \right|} (W^2)^{1-\frac{1}{k}} \quad . \quad (D30) \end{aligned}$$

When Stirling's approximative formula for large binomial coefficients is used, it leads to

$$\begin{aligned}
1 &> (W^2) \limsup_{k \rightarrow \infty} \sqrt[k]{\left| \frac{k}{(1+\mu)k+1-k} \frac{1}{\sqrt{2\pi}} \frac{((1+\mu)k)^{(1+\mu)k+\frac{1}{2}}}{k^{k+\frac{1}{2}}((1+\mu)k-k)^{(1+\mu)k-k+\frac{1}{2}}} \right|} \\
&= (W^2) \limsup_{k \rightarrow \infty} \sqrt[k]{\left| \frac{k}{\mu k+1} \frac{1}{\sqrt{2\pi}} \frac{(1+\mu)^{(1+\mu)k+\frac{1}{2}} k^{(1+\mu)k+\frac{1}{2}}}{k^{k+\frac{1}{2}}(\mu k)^{\mu k+\frac{1}{2}}} \right|} = \\
&= (W^2) \limsup_{k \rightarrow \infty} \sqrt[k]{\left| \frac{k}{\mu k+1} \frac{1}{\sqrt{2\pi}} \frac{(1+\mu)^{(1+\mu)k+\frac{1}{2}} k^{\mu k}}{(\mu k)^{\mu k+\frac{1}{2}}} \right|} = \\
&= (W^2) \limsup_{k \rightarrow \infty} \sqrt[k]{\left| \frac{k^{\frac{1}{2}}}{\mu k+1} \frac{1}{\sqrt{2\pi}} \frac{(1+\mu)^{(1+\mu)k+\frac{1}{2}}}{(\mu)^{\mu k+\frac{1}{2}}} \right|} = \\
&= (W^2) \limsup_{k \rightarrow \infty} \left| \frac{1}{\left(\mu k^{\frac{1}{2}} + \frac{1}{k^{\frac{1}{2}}}\right)^{\frac{1}{k}}} \frac{1}{(2\pi)^{\frac{1}{2k}}} \frac{(1+\mu)^{(1+\mu)+\frac{1}{2k}}}{(\mu)^{\mu+\frac{1}{2k}}} \right| = \left| \frac{(1+\mu)^{1+\mu}}{\mu^\mu} \right| (W^2) < 1
\end{aligned} \tag{D31}$$

Then

$$W^2 < \left| \frac{\mu^\mu}{(1+\mu)^{1+\mu}} \right| \Rightarrow W < \sqrt{\frac{\mu^\mu}{(1+\mu)^{1+\mu}}} \tag{D32}$$

It is the same limit as for the coordinates calculation. It also does worth to note that the  $h_R$  metric scale factor in the small- $v$  region has also the same convergence limit.

### ***Large- $v$ region, $h_R$ metric scale factor***

For the derivation of  $h_R$ , Eqs. (68) and (69) are used. When the derivatives are input to the basic equation (16), we obtain

$$\begin{aligned}
h_R &= \sqrt{\left(\frac{\partial x(v, R)}{\partial R}\right)^2 + \left(\frac{\partial z(v, R)}{\partial R}\right)^2} = \\
&= \sqrt{\left(\frac{W^{-\frac{1}{1+\mu}}}{1+\mu} \sum_{k=0}^{\infty} \left(\left(\frac{1}{2(1+\mu)} - 1\right) + \frac{1}{1+\mu}k\right) \binom{k}{k} \left(-W^{-\frac{2}{1+\mu}}\right)^k\right)^2 + \left(\frac{1}{(1+\mu)^{1/2}} \sum_{k=0}^{\infty} \left(-\frac{1}{2} + \frac{1}{1+\mu}k\right) \binom{k}{k} \left(-W^{-\frac{2}{1+\mu}}\right)^k\right)^2}
\end{aligned} \tag{D33}$$

When applying the Cauchy product formula to the squares of the individual derivatives, we obtain

$$\begin{aligned}
h_R &= \left[ \frac{W^{-\frac{2}{1+\mu}}}{(1+\mu)^2} \sum_{k=0}^{\infty} \left(-W^{-\frac{2}{1+\mu}}\right)^k \sum_{m=0}^k \left(\left(\frac{1}{2(1+\mu)} - 1\right) + \frac{1}{1+\mu}m\right) \binom{k}{m} \left(\left(\frac{1}{2(1+\mu)} - 1\right) + \frac{1}{1+\mu}(k-m)\right) \binom{k-m}{k-m} \right. \\
&\quad \left. + \frac{1}{(1+\mu)} \sum_{k=0}^{\infty} \left(-W^{-\frac{2}{1+\mu}}\right)^k \sum_{m=0}^k \left(-\frac{1}{2} + \frac{1}{1+\mu}m\right) \binom{k}{m} \left(-\frac{1}{2} + \frac{1}{1+\mu}(k-m)\right) \binom{k-m}{k-m} \right]^{\frac{1}{2}}
\end{aligned} \tag{D34}$$

Using Jensen combinatorial formula (listed as No 3.144 in [Gould 1972](#)), we can simplify this to

$$h_R = \left[ \frac{W^{-\frac{2}{1+\mu}}}{(1+\mu)^2} \sum_{k=0}^{\infty} \left( -W^{-\frac{2}{1+\mu}} \right)^k \sum_{m=0}^k \binom{-1 - \frac{\mu}{1+\mu}(k+1) + k - m}{k-m} \left( \frac{1}{1+\mu} \right)^m + \frac{1}{(1+\mu)} \sum_{k=0}^{\infty} \left( -W^{-\frac{2}{1+\mu}} \right)^k \sum_{m=0}^k \binom{-1 - \frac{\mu}{1+\mu}k + k - m}{k-m} \left( \frac{1}{1+\mu} \right)^m \right]^{\frac{1}{2}} \quad (D35)$$

Using reverse counting in the inner sums we have

$$h_R = \left[ \frac{W^{-\frac{2}{1+\mu}}}{(1+\mu)^2} \sum_{k=0}^{\infty} \left( -W^{-\frac{2}{1+\mu}} \right)^k \sum_{m=0}^k \binom{-1 - \frac{\mu}{1+\mu}(k+1) + m}{m} \left( \frac{1}{1+\mu} \right)^{k-m} + \frac{1}{1+\mu} \sum_{k=0}^{\infty} \left( -W^{-\frac{2}{1+\mu}} \right)^k \sum_{m=0}^k \binom{-1 - \frac{\mu}{1+\mu}k + m}{m} \left( \frac{1}{1+\mu} \right)^{k-m} \right]^{\frac{1}{2}} \quad (D36)$$

Now, substitution  $K=k+1$  can be used in the first term, followed by adding and subtracting terms at the end and begin of the series, and resulting in the following shape:

$$\begin{aligned} & \frac{W^{-\frac{2}{1+\mu}}}{(1+\mu)^2} \sum_{K=1}^{\infty} \left( -W^{-\frac{2}{1+\mu}} \right)^{K-1} \sum_{m=0}^{K-1} \binom{-\frac{\mu}{1+\mu}K - 1 + m}{m} \left( \frac{1}{1+\mu} \right)^{K-1-m} \\ &= -\frac{1}{1+\mu} \sum_{K=1}^{\infty} \left( -W^{-\frac{2}{1+\mu}} \right)^K \sum_{m=0}^{K-1} \binom{-\frac{\mu}{1+\mu}K - 1 + m}{m} \left( \frac{1}{1+\mu} \right)^{K-m} = \\ &= -\frac{1}{1+\mu} \sum_{K=1}^{\infty} \left( -W^{-\frac{2}{1+\mu}} \right)^K \left[ \sum_{m=0}^K \binom{-\frac{\mu}{1+\mu}K - 1 + m}{m} \left( \frac{1}{1+\mu} \right)^{K-m} - \left( \left( 1 - \frac{\mu}{1+\mu} \right) K - 1 \right) \right] = \\ &= -\frac{1}{1+\mu} \sum_{K=0}^{\infty} \left( -W^{-\frac{2}{1+\mu}} \right)^K \sum_{m=0}^K \binom{-1 - \frac{\mu}{1+\mu}K + m}{m} \left( \frac{1}{1+\mu} \right)^{K-m} + \frac{1}{1+\mu} \\ &+ \frac{1}{1+\mu} \sum_{K=1}^{\infty} \left( -W^{-\frac{2}{1+\mu}} \right)^K \left( \left( 1 - \frac{\mu}{1+\mu} \right) K - 1 \right) \end{aligned} \quad (D37)$$

where we employed the fact that anything calling zero in generalized binomial coefficient is equal to one. Now, it can be recognized, that the left double sum is equal to the second term in (D36) but having an opposite sign. Therefore,  $h_R$  equals to

$$h_R = \frac{1}{\sqrt{1+\mu}} \sqrt{1 + \sum_{K=1}^{\infty} \binom{-\frac{\mu}{1+\mu}K + K - 1}{K} \left( -W^{-\frac{2}{1+\mu}} \right)^K} = \frac{1}{\sqrt{1+\mu}} \sqrt{\sum_{k=0}^{\infty} \binom{\frac{1}{1+\mu}k - 1}{k} \left( -W^{-\frac{2}{1+\mu}} \right)^k} \quad (D38)$$

When using the right-hand side binomial identity of (A3), we finally arrive at

$$h_R = \frac{1}{\sqrt{1+\mu}} \sqrt{\sum_{k=0}^{\infty} \binom{\frac{\mu}{1+\mu}k}{k} \left( W^{-\frac{2}{1+\mu}} \right)^k}$$

, (D39)

where  $W \equiv W(R, \nu)$  is given by Eq. (22).

On the polar axis ( $\nu=\pi/2$ ), the only nonzero term in the power sum is the one with  $k=0$ , and this expression thus simplifies to

$$h_R \left( \nu = \frac{\pi}{2} \right) = \frac{1}{\sqrt{1+\mu}} \quad . \quad (D40)$$

Further, (D38) form of  $h_R$  can be transformed to a form where the sum is in the denominator. For this purpose, the Pólya and Szegő identity listed under Nr. 1.120 in [Gould 1972](#) is used. Then

$$h_R = \frac{1}{\sqrt{1+\mu}} \sqrt{\sum_{k=0}^{\infty} \binom{\frac{1}{1+\mu}k-1}{k} \left( -W^{-\frac{2}{1+\mu}} \right)^k} = \frac{1}{\sqrt{1+\mu}} \sqrt{\frac{p^{-1+1}}{\left( 1 - \frac{1}{1+\mu} \right)p + \frac{1}{1+\mu}}} \quad \text{where } -W^{-\frac{2}{1+\mu}} = \frac{p-1}{p^{\frac{1}{1+\mu}}} \quad . \quad (D41)$$

The expression for  $p$  is then

$$W^{-\frac{2}{1+\mu}} p^{\frac{1}{1+\mu}} + p = 1 \quad , \quad (D42)$$

resembles (9), and the solution for  $p$  can be thus obtained using (10). Therefore, we can write for  $h_R$

$$h_R = \frac{1}{\sqrt{1+\mu}} \frac{1}{\sqrt{\frac{1}{1+\mu} + \frac{\mu}{1+\mu}p}} = \frac{1}{\sqrt{1+\mu}} \left[ \frac{1}{1+\mu} + \frac{\mu}{1+\mu} \sum_{k=0}^{\infty} \binom{1 + \frac{1}{1+\mu}k}{k} \frac{\left( -W^{-\frac{2}{1+\mu}} \right)^k}{1 + \frac{1}{1+\mu}k} \right]^{-\frac{1}{2}} \\ = \left[ 1 - \mu \sum_{k=0}^{\infty} \binom{\frac{\mu}{1+\mu}k-1}{k} \frac{\left( W^{-\frac{2}{1+\mu}} \right)^k}{\frac{\mu}{1+\mu}k-1} \right]^{-\frac{1}{2}} \quad . \quad (D43)$$

where the last expression comes from the use of the identity (A3).

### ***Large- $\nu$ region, $h_\nu$ metric scale factor***

With formulas for squared derivatives (see Eqs. (78) and (79)), we are able to calculate also the scale factor  $h_\nu$  of SOS coordinates according to Eq. (16) in the large- $\nu$  region:

$$\begin{aligned}
h_\nu &= \sqrt{\left(\frac{\partial x(\nu, R)}{\partial \nu}\right)^2 + \left(\frac{\partial z(\nu, R)}{\partial \nu}\right)^2} \\
&= \frac{R}{2} \frac{1}{\mu W^{1+\frac{1}{1+\mu}}} \frac{\partial W}{\partial \nu} \left\{ \left( -4 \frac{1+\mu}{\mu} \sum_{M=1}^{\infty} \frac{1}{\mu M - \mu - 1} \binom{\frac{\mu}{1+\mu} M}{M} \left(W^{-\frac{2}{1+\mu}}\right)^{M-1} \right. \right. \\
&\quad - \frac{8}{\mu} \sum_{M=1}^{\infty} \binom{\frac{\mu}{1+\mu} M}{M} \left(W^{-\frac{2}{1+\mu}}\right)^{M-1} \\
&\quad + \frac{4}{1+\mu} \sum_{M=0}^{\infty} \left(-W^{-\frac{2}{1+\mu}}\right)^{M-1} \sum_{m=0}^M \binom{-\frac{\mu}{1+\mu} M - 1 + m}{m} \frac{1}{(1+\mu)^{M-m}} \\
&\quad \left. - \frac{4}{1+\mu} \sum_{M=0}^{\infty} \binom{-\frac{\mu}{1+\mu} M + M - 1}{M} \left(-W^{-\frac{2}{1+\mu}}\right)^{M-1} \right\} \\
&\quad + \left\{ \frac{1}{1+\mu} \frac{4}{\mu} \sum_{k=1}^{\infty} \frac{1}{-1 + \frac{\mu}{1+\mu} k} \binom{\frac{\mu}{1+\mu} k}{k} \left(W^{-\frac{2}{1+\mu}}\right)^{k-1} + \frac{1}{1+\mu} \frac{4}{W^{-\frac{2}{1+\mu}}} \right. \\
&\quad + \frac{1}{1+\mu} \frac{8}{\mu} \sum_{k=1}^{\infty} \binom{\frac{\mu}{1+\mu} k}{k} \left(W^{-\frac{2}{1+\mu}}\right)^{k-1} - \frac{1}{1+\mu} \frac{8}{W^{-\frac{2}{1+\mu}}} \\
&\quad \left. - 4 \frac{1}{1+\mu} \sum_{k=0}^{\infty} \left[ (-1)^{k-1} \left(W^{-\frac{2}{1+\mu}}\right)^{k-1} \sum_{m=0}^k \binom{-\frac{\mu}{1+\mu} k - 1 + m}{m} \frac{1}{(1+\mu)^{k-m}} \right] \right\}^{\frac{1}{2}}, \tag{D44}
\end{aligned}$$

We now combine the similar sums, use the identity (A3) in one of the sums, and include two of the terms at the begin of the appropriate sums:

$$\begin{aligned}
h_\nu &= \frac{R}{2} \frac{1}{\mu W^{1+\frac{1}{1+\mu}}} \frac{\partial W}{\partial \nu} \left\{ -4 \sum_{M=1}^{\infty} \frac{1}{\mu M - \mu - 1} \binom{\frac{\mu}{1+\mu} M}{M} \left(W^{-\frac{2}{1+\mu}}\right)^{M-1} + \frac{1}{1+\mu} \frac{4}{W^{-\frac{2}{1+\mu}}} \right. \\
&\quad - \frac{8}{1+\mu} \sum_{M=1}^{\infty} \binom{\frac{\mu}{1+\mu} M}{M} \left(W^{-\frac{2}{1+\mu}}\right)^{M-1} - \frac{1}{1+\mu} \frac{8}{W^{-\frac{2}{1+\mu}}} \\
&\quad \left. - \frac{4}{1+\mu} \sum_{M=0}^{\infty} \binom{\frac{\mu}{1+\mu} M}{M} (-1)^M \left(-W^{-\frac{2}{1+\mu}}\right)^{M-1} \right\}^{\frac{1}{2}} = \\
&= \frac{R}{2} \frac{1}{\mu W^{1+\frac{1}{1+\mu}}} \frac{\partial W}{\partial \nu} \left\{ -4 \sum_{M=0}^{\infty} \frac{1}{\mu M - \mu - 1} \binom{\frac{\mu}{1+\mu} M}{M} \left(W^{-\frac{2}{1+\mu}}\right)^{M-1} \right. \\
&\quad \left. - \frac{8}{1+\mu} \sum_{M=0}^{\infty} \binom{\frac{\mu}{1+\mu} M}{M} \left(W^{-\frac{2}{1+\mu}}\right)^{M-1} + \frac{4}{1+\mu} \sum_{M=0}^{\infty} \binom{\frac{\mu}{1+\mu} M}{M} \left(W^{-\frac{2}{1+\mu}}\right)^{M-1} \right\}^{\frac{1}{2}} = \\
&= R \frac{1}{\mu W^{1+\frac{1}{1+\mu}}} \frac{\partial W}{\partial \nu} \left\{ - \sum_{M=0}^{\infty} \frac{\frac{\mu}{1+\mu} M}{\mu(M-1)-1} \binom{\frac{\mu}{1+\mu} M}{M} \left(W^{-\frac{2}{1+\mu}}\right)^{M-1} \right\}^{\frac{1}{2}}. \tag{D45}
\end{aligned}$$

Then

$$h_v = R \frac{1}{\mu W} \frac{\partial W}{\partial v} \sqrt{- \sum_{M=0}^{\infty} \frac{\frac{\mu}{1+\mu} M}{\mu(M-1)-1} \binom{\frac{\mu}{1+\mu} M}{M} \left(W^{-\frac{2}{1+\mu}}\right)^M} \quad (D46)$$

This formula can be directly used for  $\mu > -1$ , except the cases for which  $\mu$  is equal to 1,  $\frac{1}{2}$ ,  $\frac{1}{3}$ ,  $\frac{1}{4}$  etc. as the denominator would then equal to zero for certain  $M$  (particularly for  $M=1+1/\mu$ ) in these cases.

Also for this large- $v$  region holds that, for the limit  $\mu \rightarrow 0$ ,  $h_v$  should be finite, and, moreover, equal to  $R$  as the SOS coordinate system equals to spherical coordinate system for  $\mu=0$ . However, it cannot be directly seen from the formula (D46). Therefore, it is useful to rewrite this formula also to another shape using (A3) binomial identity (with  $\beta = -\frac{\mu}{1+\mu}M$ ). Then

$$\begin{aligned} h_v &= R \frac{1}{\mu W} \frac{\partial W}{\partial v} \sqrt{- \left[ 0 + \sum_{M=1}^{\infty} \frac{\frac{\mu}{1+\mu} M}{\mu(M-1)-1} \cdot \frac{-\frac{\mu}{1+\mu} M}{-\frac{\mu}{1+\mu} M + M} \binom{-\frac{\mu}{1+\mu} M + M}{M} (-1)^M \left(W^{-\frac{2}{1+\mu}}\right)^M \right]} \\ &= R \frac{1}{W} \frac{\partial W}{\partial v} \sqrt{\sum_{M=1}^{\infty} \frac{\frac{1}{1+\mu} M}{\mu(M-1)-1} \binom{\frac{1}{1+\mu} M}{M} \cdot \left(-W^{-\frac{2}{1+\mu}}\right)^M} \end{aligned} \quad (D47)$$

which for  $\mu=0$  equals to

$$h_v = R \frac{1}{W} \frac{\partial W}{\partial v} \sqrt{\sum_{M=1}^{\infty} \frac{M}{-1} \binom{M}{M} \cdot \left(-W^{-2}\right)^M} = R \frac{1}{W} \frac{\partial W}{\partial v} \sqrt{- \frac{-W^{-2}}{(1+W^{-2})^2}} = R \frac{\partial W}{\partial v} \frac{1}{W^2 + 1} = R \frac{1}{\cos^2 v} \frac{1}{\frac{\sin^2 v}{\cos^2 v} + 1} = R \quad (D48)$$

Above, we used the identity  $\binom{k}{k} = 1$ , the well-known closed form of the infinite series  $\sum_{k=1}^{\infty} k y^k = y/(1-y)^2$ , and the formulas (74) for  $W$  and its derivative with  $\mu=0$ . It can be seen, that the result equals to the one valid for spherical coordinates.

Further, already mentioned restriction with (D47) expression is that  $\mu$  cannot be equal to 1,  $\frac{1}{2}$ ,  $\frac{1}{3}$ ,  $\frac{1}{4}$  ... as the denominator would then be equal to zero for certain  $M$  (particularly for  $M=1+1/\mu$ ) in these cases. Nevertheless, also the binomial coefficient goes to zero in these cases and the limit of  $h_v$  is then finite, only a proper expression has to be found. For its derivation, we use the binomial identity (A4) with

$$k = M \quad \text{and} \quad \alpha = \frac{1}{1+\mu} M \quad (D49)$$

and the fact that the term with  $M=0$  has magnitude zero. With this, (D47) expression can be rewritten into the form

$$h_v = R \frac{1}{W} \frac{\partial W}{\partial v} \sqrt{\sum_{M=1}^{\infty} \frac{\frac{1}{1+\mu} M}{\mu(M-1)-1} \binom{\frac{1}{1+\mu} M}{M-1} \frac{-(\mu M - \mu - 1)}{M(1+\mu)} \cdot \left(-W^{-\frac{2}{1+\mu}}\right)^M} \quad (D50)$$

and, after the final simplification, we arrive at

$$h_v = \frac{R}{1+\mu} \frac{1}{W} \frac{\partial W}{\partial v} \sqrt{- \sum_{M=1}^{\infty} \binom{\frac{1}{1+\mu} M}{M-1} \cdot \left(-W^{-\frac{2}{1+\mu}}\right)^M} = \frac{R}{1+\mu} W^{-\frac{2+\mu}{1+\mu}} \frac{\partial W}{\partial v} \sqrt{\sum_{k=0}^{\infty} \binom{\frac{1}{1+\mu} k + \frac{1}{1+\mu}}{k} \cdot \left(-W^{-\frac{2}{1+\mu}}\right)^k} \quad (D51)$$

or even (with help of (A3) identity) at

$$h_v = \frac{R}{1+\mu} \frac{1}{W} \frac{\partial W}{\partial v} \sqrt{-\sum_{k=0}^{\infty} \binom{\frac{1}{1+\mu}(k+1)}{k} \cdot \left(-W^{-\frac{2}{1+\mu}}\right)^{k+1}} =$$

$$= \frac{R}{1+\mu} W^{-\frac{2+\mu}{1+\mu}} \frac{\partial W}{\partial v} \sqrt{\sum_{k=0}^{\infty} \binom{\frac{\mu}{1+\mu}k - \frac{2+\mu}{1+\mu}}{k} \cdot \left(W^{-\frac{2}{1+\mu}}\right)^k}$$
(D52)

which can be used for any  $\mu > -1$ . However, the  $\partial W / \partial v$  factor in front of the square root could indicate that the value of the metric scale factor could be infinity for  $v=\pi/2$  (i.e. at the polar axis), as there is a factor  $\cos^{2+\mu} v$  in the denominator of  $\partial W / \partial v$  (see Eq. (74)). Nevertheless, if we make substitution according to (74) in all the terms with  $W$ , we can see the following:

$$h_v = \frac{R}{1+\mu} \frac{1+\mu \sin^2 v}{\sin v \cos v} \sqrt{-\sum_{M=1}^{\infty} \binom{\frac{1}{1+\mu}M}{M-1} \cdot \left(-\left(\frac{R}{R_0}\right)^{\mu} \frac{\sin v}{\cos^{1+\mu} v}\right)^{-\frac{2}{1+\mu}}^M} =$$

$$= \frac{R}{1+\mu} \frac{1+\mu \sin^2 v}{\sin v \cos v} \sqrt{-\sum_{M=1}^{\infty} \binom{\frac{1}{1+\mu}M}{M-1} (-1)^M \left(\frac{R}{R_0}\right)^{-\frac{2\mu M}{1+\mu}} \frac{\sin^{-\frac{2M}{1+\mu}v}}{\cos^{-2M} v}}$$

$$= \frac{R}{1+\mu} \sqrt{-\sum_{M=1}^{\infty} \binom{\frac{1}{1+\mu}M}{M-1} (-1)^M \left(\frac{R}{R_0}\right)^{-\frac{2\mu M}{1+\mu}} \frac{(1+\mu \sin^2 v)^2 \sin^{-\frac{2M}{1+\mu}v}}{\sin^2 v \cos^{-2M+2} v}}$$

$$= \frac{R}{1+\mu} \sqrt{-\sum_{M=1}^{\infty} \binom{\frac{1}{1+\mu}M}{M-1} (-1)^M \left(\frac{R}{R_0}\right)^{-\frac{2\mu M}{1+\mu}} \frac{(1+\mu \sin^2 v)^2 \cos^{2M-2} v}{\sin^{\frac{2M}{1+\mu}+2} v}}$$
(D53)

This has a finite value for  $v=\pi/2$  (only the term with  $M=1$  in the power series is nonzero), equal to

$$h_v \left(v = \frac{\pi}{2}\right) = R \left(R/R_0\right)^{-\frac{\mu}{1+\mu}}.$$
(D54)

Convergence limit of the power series has to be tested as well. We use the root test

$$1 > \limsup_{M \rightarrow \infty} \sqrt[M]{\left| \binom{\frac{1}{1+\mu}M}{M-1} \cdot \left(-W^{-\frac{2}{1+\mu}}\right)^M \right|} = \limsup_{M \rightarrow \infty} \sqrt[M]{\left| \binom{\frac{1}{1+\mu}M}{M-1} \right|} \left(W^{-\frac{2}{1+\mu}}\right)$$

$$= \limsup_{M \rightarrow \infty} \sqrt[M]{\left| \frac{M}{\frac{1}{1+\mu}M + 1 - M} \binom{\frac{1}{1+\mu}M}{M} \right|} \left(W^{-\frac{2}{1+\mu}}\right)$$
(D55)

When Stirling's formula for large binomial coefficients is used, this leads to

$$\begin{aligned}
1 &> \limsup_{M \rightarrow \infty} \sqrt[M]{\left| \frac{M}{\frac{1}{1+\mu}M + 1 - M} \frac{1}{\sqrt{2\pi}} \frac{\left(\frac{1}{1+\mu}M\right)^{\frac{1}{1+\mu}M + \frac{1}{2}}}{M^{M+\frac{1}{2}} \left(\frac{1}{1+\mu}M - M\right)^{\frac{1}{1+\mu}M - M + \frac{1}{2}}} \right|} \left(W^{-\frac{2}{1+\mu}}\right) = \\
&= \limsup_{M \rightarrow \infty} \sqrt[M]{\left| \frac{M}{\frac{-\mu}{1+\mu}M + 1} \frac{1}{\sqrt{2\pi}} \frac{\left(\frac{1}{1+\mu}M\right)^{\frac{1}{1+\mu}M + \frac{1}{2}}}{M^{M+\frac{1}{2}} M^{\frac{1}{1+\mu}M - M + \frac{1}{2}} \left(\frac{-\mu}{1+\mu}\right)^{\frac{1}{1+\mu}M - M + \frac{1}{2}}} \right|} \left(W^{-\frac{2}{1+\mu}}\right) = \\
&= \limsup_{M \rightarrow \infty} \sqrt[M]{\left| \frac{M}{\frac{-\mu}{1+\mu}M + 1} \frac{1}{\sqrt{2\pi}} \frac{M^{\frac{1}{1+\mu}M + \frac{1}{2}} \left(\frac{1}{1+\mu}\right)^{\frac{1}{1+\mu}M + \frac{1}{2}}}{M^{\frac{1}{1+\mu}M + 1} \left(\frac{-\mu}{1+\mu}\right)^{\frac{1}{1+\mu}M - M + \frac{1}{2}}} \right|} \left(W^{-\frac{2}{1+\mu}}\right) = \\
&= \limsup_{M \rightarrow \infty} \sqrt[M]{\left| \frac{M}{\frac{-\mu}{1+\mu}M + 1} \frac{1}{\sqrt{2\pi}} \frac{1}{M^{\frac{1}{2}} (-\mu)^{\frac{1}{1+\mu}M - M + \frac{1}{2}} \left(\frac{1}{1+\mu}\right)^{-M}} \right|} \left(W^{-\frac{2}{1+\mu}}\right) = \\
&= \limsup_{M \rightarrow \infty} \sqrt[M]{\left| \frac{M^{\frac{1}{2}}}{\frac{-\mu}{1+\mu}M + 1} \frac{1}{\sqrt{2\pi}} \frac{1}{(-\mu)^{M \frac{-\mu}{1+\mu} + \frac{1}{2}} \left(\frac{1}{1+\mu}\right)^{-M}} \right|} \left(W^{-\frac{2}{1+\mu}}\right) = \\
&= \limsup_{M \rightarrow \infty} \left| \frac{M^{\frac{1}{2M}}}{\left(\frac{-\mu}{1+\mu}M + 1\right)^{\frac{1}{M}}} \frac{1}{(2\pi)^{\frac{1}{2M}}} \frac{1}{(-\mu)^{\frac{-\mu}{1+\mu} + \frac{1}{2M}} \left(\frac{1}{1+\mu}\right)^{-1}} \right| \left(W^{-\frac{2}{1+\mu}}\right) \\
&= \limsup_{M \rightarrow \infty} \left| \frac{1}{\left(\frac{-\mu}{1+\mu}M^{\frac{1}{2}} + \frac{1}{M^{\frac{1}{2}}}\right)^{\frac{1}{M}}} \frac{1}{(2\pi)^{\frac{1}{2M}}} \frac{\frac{1}{1+\mu}}{(-\mu)^{\frac{-\mu}{1+\mu} + \frac{1}{2M}}} \right| \left(W^{-\frac{2}{1+\mu}}\right) \\
&= \limsup_{M \rightarrow \infty} \left| \frac{\frac{1}{1+\mu}}{(-\mu)^{\frac{-\mu}{1+\mu}}} \right| \left(W^{-\frac{2}{1+\mu}}\right) = \left| \frac{(-\mu)^{\frac{\mu}{1+\mu}}}{(1+\mu)} \right| \left(W^{-\frac{2}{1+\mu}}\right) < 1
\end{aligned} \tag{D56}$$

Then

$$\begin{aligned}
&\left| \frac{(-\mu)^{\frac{\mu}{1+\mu}}}{(1+\mu)} \right| < W^{\frac{2}{1+\mu}} \\
W &> \sqrt{\left| \frac{(i^2\mu)^\mu}{(1+\mu)^{1+\mu}} \right|} \quad \text{and thus} \quad W > \sqrt{\frac{\mu^\mu}{(1+\mu)^{1+\mu}}}
\end{aligned} \tag{D57}$$

It is the same limit as for the coordinates calculation. It also does worth to note that the  $h_R$  metric scale factor in the large- $v$  region has also the same convergence limit. Further, the border line is shared by both regions, i.e. by the small- $v$  region and by the large- $v$  region.

### $h_R$ scale factor for $R = R_0$ in small- and large- $v$ regions

Another useful relations are the ones for  $h_R$  scale factor for  $R = R_0$ , i.e. at the reference oblate spheroid with equatorial radius  $R_0$ . The relation will be derived for both the small- and large- $v$  regions.

For  $R=R_0$ , the parameter  $W$  (see (22)) equals to

$$W_0 \equiv W_0(v) = \frac{\sin v}{\cos^{1+\mu} v} \quad . \quad (D58)$$

The power series in (D6) can be expressed using Polya and Szego identity ([GOULD], No. 1.120). Then (for the small- $v$  region)

$$h_{Rs0} = \sqrt{\sum_{k=0}^{\infty} \binom{(\mu+1)k-1}{k} (-W_0^2)^k} = \sqrt{\frac{p^{-1+1}}{(1-(\mu+1)p+(\mu+1))}} = \frac{1}{\sqrt{1+\mu(1-p)}} \quad \text{where} \quad -W_0^2 = \frac{p-1}{p^{\mu+1}} \quad (D59)$$

(extending the index of  $h_R$  by  $s_0$  means that we are at the reference spheroid in the small- $v$  part of the meridional coordinate range). After inserting relation (D58) we receive

$$h_{Rs0} = \frac{1}{\sqrt{1+\mu(1-p)}} \quad \text{where} \quad -\frac{\sin^2 v}{(\cos^2 v)^{1+\mu}} = \frac{p-1}{p^{\mu+1}} \quad . \quad (D60)$$

If we suppose that  $p=\cos^2 v$ , then it can be seen that the right-side equation is fulfilled. Therefore,

$$h_{Rs0} = \frac{1}{\sqrt{1+\mu(1-\cos^2 v)}} = \frac{1}{\sqrt{1+\mu \sin^2 v}} \quad . \quad (D61)$$

Similarly, for the large- $v$  region (Eq. (D38)), we can perform the same analysis and arrive at

$$h_{Rl0} = \frac{1}{\sqrt{1+\mu}} \sqrt{\sum_{k=0}^{\infty} \binom{\frac{1}{1+\mu}k-1}{k} (-W_0^{-\frac{2}{1+\mu}})^k} = \frac{1}{\sqrt{1+\mu}} \sqrt{\frac{q^{-1+1}}{(1-\frac{1}{1+\mu})q+\frac{1}{1+\mu}}} = \frac{1}{\sqrt{1+\mu}} \frac{1}{\sqrt{\frac{1+\mu q}{1+\mu}}} \quad \text{where} \quad -W_0^{-\frac{2}{1+\mu}} = \frac{q-1}{q^{\frac{1}{1+\mu}}} \quad (D62)$$

(extending the index of  $h_R$  by  $l_0$  means that we are at the reference spheroid in the large- $v$  part of the meridional coordinate range). After inserting (D58), we receive

$$h_{Rl0} = \frac{1}{\sqrt{1+\mu q}} \quad \text{where} \quad -\left[\frac{\sin^2 v}{(\cos^2 v)^{1+\mu}}\right]^{-\frac{1}{1+\mu}} = -\frac{\cos^2 v}{(\sin^2 v)^{\frac{1}{1+\mu}}} = \frac{q-1}{q^{\frac{1}{1+\mu}}} \quad . \quad (D63)$$

If we suppose that  $q=\sin^2 v$ , then it can be seen that the right-side equation is fulfilled. Therefore,

$$h_{Rl0} = \frac{1}{\sqrt{1+\mu \sin^2 v}} \quad . \quad (D64)$$

Therefore,  $h_R$  magnitude exactly at the reference spheroid, i.e. for  $R=R_0$ , has the same closed form for the **small-** and for the **large- $v$  region**:

$$h_{R0} = h_{Rs0} = h_{RI0} = \frac{1}{\sqrt{1+\mu \sin^2 v}} . \quad (D65)$$

Due to continuity, the metric scale factor has to have the same magnitude also on the intersection of the reference spheroid with the border between the **small-** and the **large- $v$  regions**.

The above derivations also represent new (to the extent the author is informed) binomial identities in the respective  $v$  regions:

$$\sum_{k=0}^{\infty} \binom{-\mu k}{k} \left( \frac{\sin v}{\cos^{1+\mu} v} \right)^{2k} = \sum_{k=0}^{\infty} \binom{(\mu+1)k-1}{k} \left( - \left( \frac{\sin v}{\cos^{1+\mu} v} \right)^2 \right)^k = \frac{1}{1+\mu \sin^2 v} . \quad (D66)$$

$$\sum_{k=0}^{\infty} \binom{\frac{\mu}{1+\mu} k}{k} \left( \frac{\cos v}{\sin^{1+\mu} v} \right)^{2k} = \sum_{k=0}^{\infty} \binom{\frac{1}{1+\mu} k-1}{k} \left( - \left( \frac{\cos v}{\sin^{1+\mu} v} \right)^2 \right)^k = \frac{1+\mu}{1+\mu \sin^2 v} . \quad (D67)$$

#### **$h_v$ scale factor for $R = R_0$ in small- and large- $v$ regions**

Another useful relations are the ones for  $h_v$  scale factor for  $R = R_0$ , i.e. at the reference oblate spheroid with equatorial radius  $R_0$ . The relation will be derived for both the small- and the large- $v$  region.

For  $R=R_0$ , the parameter  $W$  equals to (D58). The power series in (D27) (i.e. for the **small- $v$  region**) can be expressed using Polya and Szego identity ([GOULD], No. 1.120)

$$\sqrt{\sum_{k=0}^{\infty} \binom{(1+\mu)k+(1+\mu)}{k} (-W_0^2)^k} = \sqrt{\frac{p^{(1+\mu)+1}}{(1-(\mu+1)p+(\mu+1))}} = \frac{\sqrt{p^{2+\mu}}}{\sqrt{1+\mu(1-p)}} \quad \text{where} \quad -\frac{\sin^2 v}{(\cos^2 v)^{1+\mu}} = \frac{p-1}{p^{\mu+1}} , \quad (D68)$$

Similarly as previously for  $h_R$  in (D60) and (D61), we can deduce that  $p=\cos^2 v$ . Then, it can be derived

$$\sqrt{\sum_{k=0}^{\infty} \binom{(1+\mu)k+(1+\mu)}{k} (-W_0^2)^k} = \frac{\cos^{2+\mu} v}{\sqrt{1+\mu \sin^2 v}} , \quad (D69)$$

The metric scale factor  $h_v$  at the reference spheroid is thus (see (D27))

$$h_{vs0} = \frac{R_0}{\sqrt{1+\mu}} \frac{\partial W}{\partial v} \Big|_0 \frac{\cos^{2+\mu} v}{\sqrt{1+\mu \sin^2 v}} \quad \text{where} \quad \frac{\partial W}{\partial v} \Big|_0 = \frac{1+\mu \sin^2 v}{\cos^{2+\mu} v} , \quad (D70)$$

the  $W$ -derivative on the reference spheroid determined using (74). After insertion of the formula for derivative we have

$$h_{vs0} = \frac{R_0}{\sqrt{1+\mu}} \sqrt{1 + \mu \sin^2 v} \quad (D71)$$

in the **small- $v$  region** region.

Similarly, this analysis can be carried out also for the **large- $v$  region**. The power series in (D51) (i.e. for the **large- $v$  region**) can be also expressed using Polya and Szego identity ([GOULD], No. 1.120)

$$\sqrt{\sum_{k=0}^{\infty} \left( \frac{1}{1+\mu} k + \frac{1}{1+\mu} \right) \cdot \left( -W_0^{-\frac{2}{1+\mu}} \right)^k} = \sqrt{\frac{q^{\frac{1}{1+\mu}+1}}{\left(1-\frac{1}{1+\mu}\right)^q + \frac{1}{1+\mu}}} = \sqrt{\frac{q^{\frac{2+\mu}{1+\mu}}}{\frac{1+\mu q}{1+\mu}}} \quad \text{where} \quad -W_0^{-\frac{2}{1+\mu}} = -\frac{(\sin^2 v)^{-\frac{1}{1+\mu}}}{(\cos^2 v)^{-1}} = \frac{q-1}{q^{\frac{1}{1+\mu}}} \quad (D72)$$

Then

$$-\frac{(\cos^2 v)^{\frac{1}{1+\mu}}}{(\sin^2 v)^{\frac{1}{1+\mu}}} = \frac{q-1}{q^{\frac{1}{1+\mu}}} \Rightarrow \frac{(\cos^2 v)^{1+\mu}}{\sin^2 v} = \frac{(1-q)^{1+\mu}}{q} \Rightarrow q = \sin^2 v \quad (D73)$$

and

$$\sqrt{\sum_{k=0}^{\infty} \left( \frac{1}{1+\mu} k + \frac{1}{1+\mu} \right) \cdot \left( -W_0^{-\frac{2}{1+\mu}} \right)^k} = \frac{(\sin v)^{\frac{2+\mu}{1+\mu}}}{\sqrt{\frac{1+\mu \sin^2 v}{1+\mu}}} \quad (D74)$$

The metric scale factor  $h_v$  at the reference spheroid is thus in the **large- $v$  region** (see (D51))

$$h_{vl0} = \frac{R_0}{1+\mu} W_0^{-\frac{2+\mu}{1+\mu}} \frac{\partial W}{\partial v} \Big|_0 \frac{(\sin v)^{\frac{2+\mu}{1+\mu}}}{\sqrt{\frac{1+\mu \sin^2 v}{1+\mu}}} = \frac{R_0}{1+\mu} \left( \frac{\sin v}{\cos^{1+\mu} v} \right)^{-\frac{2+\mu}{1+\mu}} \frac{1+\mu \sin^2 v}{\cos^{2+\mu} v} \frac{(\sin v)^{\frac{2+\mu}{1+\mu}}}{\sqrt{\frac{1+\mu \sin^2 v}{1+\mu}}} = \frac{R_0}{\sqrt{1+\mu}} \sqrt{1 + \mu \sin^2 v} \quad (D75)$$

Therefore,  $h_v$  magnitude exactly at the reference spheroid, i.e. for  $R=R_0$ , has the same closed form for the **small-** (see (D71)) and for the **large- $v$**  (see (D75)) regions:

$$h_{v0} = h_{vs0} = h_{vl0} = R_0 \sqrt{\frac{1+\mu \sin^2 v}{1+\mu}} \quad (D76)$$

Due to continuity, the metric scale factor has to have the same magnitude also on the intersection of the reference spheroid with the border between the **small-** and the **large- $v$  regions**.
