# Supplementary material for: Analytical Solution of Similar Oblate Spheroidal Coordinate System
Source: arXiv:2109.12057 ancillary file (2021-09-06)
Supplement: Supplementary file 4 [file Supplement_SOS_E.pdf]

# Analytical solution of Similar Oblate Spheroidal Coordinate System

---

Pavel Strunz

Nuclear Physics Institute of the CAS, Řež, Czech Republic

e-mail: strunz@ujf.cas.cz

## Supplement E

### Jacobian determinant derivation

#### Jacobian for small- $\nu$ region

First, let's calculate the following products for **small- $\nu$  region** using the derived scale factors (80), (82), (88):

$$\begin{aligned}
 \sqrt{h_\lambda} h_R &= \sqrt{\frac{R}{2}} \sqrt{\left[ \sum_{k=0}^{\infty} \binom{-\frac{1}{2}-\mu k}{k} \frac{-(W^2)^k}{-\frac{1}{2}-\mu k} \right] \left[ \sum_{k=0}^{\infty} \binom{-\mu k}{k} (W^2)^k \right]} \\
 &= \sqrt{\frac{R}{2}} \sqrt{\sum_{k=0}^{\infty} (W^2)^k \sum_{m=0}^k \binom{-\frac{1}{2}-\mu m}{m} \frac{-1}{-\frac{1}{2}-\mu m} \binom{-\mu(k-m)}{k-m}} \\
 &= \sqrt{R} \sqrt{\sum_{k=0}^{\infty} \binom{-\frac{1}{2}-\mu k}{k} (W^2)^k}
 \end{aligned} \tag{E1}$$

and

$$\begin{aligned}
 \sqrt{h_\lambda} h_\nu &= \sqrt{\frac{R}{2}} \frac{R}{\sqrt{1+\mu}} \frac{\partial W}{\partial \nu} \sqrt{\left[ \sum_{k=0}^{\infty} \binom{-\frac{1}{2}-\mu k}{k} \frac{-(W^2)^k}{-\frac{1}{2}-\mu k} \right] \left[ \sum_{k=0}^{\infty} \binom{-\mu(k+1)-2}{k} (W^2)^k \right]} \\
 &= \sqrt{\frac{R}{2}} \frac{R}{\sqrt{1+\mu}} \frac{\partial W}{\partial \nu} \sqrt{\sum_{k=0}^{\infty} (W^2)^k \sum_{m=0}^k \binom{-\frac{1}{2}-\mu m}{m} \frac{-1}{-\frac{1}{2}-\mu m} \binom{-\mu(k-m)-\mu-2}{k-m}} \\
 &= \frac{R\sqrt{R}}{\sqrt{1+\mu}} \frac{\partial W}{\partial \nu} \sqrt{\sum_{k=0}^{\infty} \binom{-\mu(k+1)-\frac{5}{2}}{k} (W^2)^k}
 \end{aligned} \tag{E2}$$

where we employed Cauchy product of infinite series followed by the Hagen-Rothe identity (Chu 2010, Chu 2013). Now, the Jacobian determinant is

$$\begin{aligned}
J &= h_R h_\nu h_\lambda = \sqrt{h_\lambda} h_\nu \sqrt{h_\lambda} h_R = \frac{R^2}{\sqrt{1+\mu}} \frac{\partial W}{\partial \nu} \sqrt{\left[ \sum_{k=0}^{\infty} \binom{-\mu(k+1) - \frac{5}{2}}{k} (W^2)^k \right] \left[ \sum_{k=0}^{\infty} \binom{-\frac{1}{2} - \mu k}{k} (W^2)^k \right]} \\
&= \frac{R^2}{\sqrt{1+\mu}} \frac{\partial W}{\partial \nu} \sqrt{\left[ \sum_{k=0}^{\infty} (W^2)^k \sum_{m=0}^k \binom{-\mu(m+1) - \frac{5}{2}}{m} \binom{-\frac{1}{2} - \mu(k-m)}{k-m} \right]} \\
&= \frac{R^2}{\sqrt{1+\mu}} \frac{\partial W}{\partial \nu} \sqrt{\left[ \sum_{k=0}^{\infty} (W^2)^k \sum_{m=0}^k \binom{-\mu m - \mu - \frac{5}{2} + (\frac{\mu}{2} + 1)}{m} \binom{-\frac{1}{2} - \mu(k-m) - (\frac{\mu}{2} + 1)}{k-m} \right]} \\
&= \frac{R^2}{\sqrt{1+\mu}} \frac{\partial W}{\partial \nu} \sqrt{\left[ \sum_{k=0}^{\infty} \binom{-\frac{\mu}{2} - \frac{3}{2} - \mu k}{k} (W^2)^k \right]^2}
\end{aligned} \tag{E3}$$

where we used the Cauchy product followed by Jensen identity (Gould 1972, No. 3.143, with  $t=1+\mu/2$ ), followed by the inverse Cauchy product. Then, the Jacobian is

$$J = h_R h_\nu h_\lambda = \frac{R^2}{\sqrt{1+\mu}} \frac{\partial W}{\partial \nu} \sum_{k=0}^{\infty} \binom{-\mu(k + \frac{1}{2}) - \frac{3}{2}}{k} (W^2)^k \tag{E4}$$

This result can be tested for  $\mu=0$ , for which the calculated Jacobian should be equivalent with the one for the spherical coordinates. For  $\mu=0$ ,  $W = \tan \nu$  and  $\partial W / \partial \nu = 1 / \cos^2 \nu$ . Therefore,

$$J_{\mu=0} = R^2 \frac{1}{\cos^2 \nu} \sum_{k=0}^{\infty} \binom{-\frac{3}{2}}{k} (\tan^2 \nu)^k = \frac{R^2}{\cos^2 \nu} (1 + \tan^2 \nu)^{-\frac{3}{2}} = \frac{R^2}{\cos^2 \nu} \left( \frac{1}{\cos^2 \nu} \right)^{-\frac{3}{2}} = R^2 \cos \nu \tag{E5}$$

where the binomial theorem was used. Taking into account that the polar angle used in spherical coordinates  $\theta$  is equal to  $\pi/2 - \nu$ , this resulting Jacobian is the same as the one for the spherical coordinates.

### Jacobian for large- $\nu$ region

For large- $\nu$  region, the derivation procedure is similar (scale factors listed in (81), (85), (89)), only the factors at various terms and the exponents are different:

$$\begin{aligned}
\sqrt{h_\lambda} h_R &= \sqrt{\frac{R}{2}} \sqrt{W^{-\frac{1}{1+\mu}}} \frac{1}{\sqrt{1+\mu}} \sqrt{\left[ \sum_{k=0}^{\infty} \left( -\frac{1}{2(1+\mu)} + \frac{\mu}{1+\mu} k \right) \frac{-\left(W^{-\frac{2}{1+\mu}}\right)^k}{-\frac{1}{2} + \mu k} \right] \left[ \sum_{k=0}^{\infty} \left( \frac{\mu}{1+\mu} k \right) \left(W^{-\frac{2}{1+\mu}}\right)^k \right]} \\
&= \sqrt{\frac{R}{2}} \sqrt{W^{-\frac{1}{1+\mu}}} \frac{1}{\sqrt{1+\mu}} \frac{1}{\sqrt{1+\mu}} \sqrt{\left[ \sum_{k=0}^{\infty} \left( -\frac{1}{2(1+\mu)} + \frac{\mu}{1+\mu} k \right) \frac{-\left(W^{-\frac{2}{1+\mu}}\right)^k}{-\frac{1}{2(1+\mu)} + \frac{\mu}{(1+\mu)} k} \right] \left[ \sum_{k=0}^{\infty} \left( \frac{\mu}{1+\mu} k \right) \left(W^{-\frac{2}{1+\mu}}\right)^k \right]} \\
&= \sqrt{\frac{R}{2}} \sqrt{W^{-\frac{1}{1+\mu}}} \frac{1}{\sqrt{1+\mu}} \frac{1}{\sqrt{1+\mu}} \sqrt{\sum_{k=0}^{\infty} \left(W^{-\frac{2}{1+\mu}}\right)^k \sum_{m=0}^k \left( -\frac{1}{2(1+\mu)} + \frac{\mu}{1+\mu} m \right) \frac{-1}{-\frac{1}{2(1+\mu)} + \frac{\mu}{(1+\mu)} m} \binom{\frac{\mu}{1+\mu}(k-m)}{k-m}} \\
&= \sqrt{\frac{R}{2}} \sqrt{W^{-\frac{1}{1+\mu}}} \frac{1}{\sqrt{1+\mu}} \frac{1}{\sqrt{1+\mu}} \sqrt{\sum_{k=0}^{\infty} \left(W^{-\frac{2}{1+\mu}}\right)^k \frac{-1}{-\frac{1}{2(1+\mu)}} \binom{-\frac{1}{2(1+\mu)} + \frac{\mu}{1+\mu} k}{k}} \\
&= W^{-\frac{1/2}{1+\mu}} \frac{\sqrt{R}}{\sqrt{1+\mu}} \sqrt{\sum_{k=0}^{\infty} \binom{\frac{\mu}{1+\mu} k - \frac{1/2}{1+\mu}}{k} \left(W^{-\frac{2}{1+\mu}}\right)^k} \tag{E6}
\end{aligned}$$

and

$$\sqrt{h_\lambda} h_\nu =$$

$$\begin{aligned}
&= \sqrt{\frac{R}{2}} \sqrt{W^{-\frac{1}{1+\mu}}} \frac{R}{1+\mu} W^{-\frac{2+\mu}{1+\mu}} \frac{\partial W}{\partial \nu} \sqrt{\left[ \sum_{k=0}^{\infty} \left( -\frac{1}{2(1+\mu)} + \frac{\mu}{1+\mu} k \right) \frac{-\left(W^{-\frac{2}{1+\mu}}\right)^k}{-\frac{1}{2} + \mu k} \right] \left[ \sum_{k=0}^{\infty} \left( \frac{\mu}{1+\mu} k - \frac{2+\mu}{1+\mu} \right) \left(W^{-\frac{2}{1+\mu}}\right)^k \right]} \\
&= R \sqrt{\frac{R}{2}} \frac{W^{-\frac{5/2+\mu}{1+\mu}}}{1+\mu} \frac{\partial W}{\partial \nu} \frac{1}{\sqrt{1+\mu}} \sqrt{\sum_{k=0}^{\infty} \left(W^{-\frac{2}{1+\mu}}\right)^k \sum_{m=0}^k \left( -\frac{1}{2(1+\mu)} + \frac{\mu}{1+\mu} m \right) \frac{-1}{-\frac{1}{2(1+\mu)} + \frac{\mu}{(1+\mu)} m} \binom{\frac{\mu}{1+\mu}(k-m) - \frac{2+\mu}{1+\mu}}{k-m}} \\
&= R \sqrt{\frac{R}{2}} \frac{W^{-\frac{5/2+\mu}{1+\mu}}}{1+\mu} \frac{\partial W}{\partial \nu} \frac{1}{\sqrt{1+\mu}} \sqrt{\sum_{k=0}^{\infty} \frac{-1}{-\frac{1}{2(1+\mu)}} \binom{-\frac{1}{2(1+\mu)} + \frac{\mu}{1+\mu} k - \frac{2+\mu}{1+\mu}}{k} \left(W^{-\frac{2}{1+\mu}}\right)^k} \\
&= \frac{R\sqrt{R}}{1+\mu} W^{-\frac{5/2+\mu}{1+\mu}} \frac{\partial W}{\partial \nu} \sqrt{\sum_{k=0}^{\infty} \binom{\frac{\mu}{1+\mu} k - \frac{5/2+\mu}{1+\mu}}{k} \left(W^{-\frac{2}{1+\mu}}\right)^k} \tag{E7}
\end{aligned}$$

where we employed Cauchy product of infinite series followed by the Hagen-Rothe identity (Chu 2010, Chu 2013). The Jacobian determinant is

$$\begin{aligned}
J &= h_R h_\nu h_\lambda = \sqrt{h_\lambda} h_\nu \sqrt{h_\lambda} h_R = \\
&= W^{-\frac{1/2}{1+\mu}} \frac{\sqrt{R}}{\sqrt{1+\mu}} \frac{R\sqrt{R}}{1+\mu} W^{-\frac{5/2+\mu}{1+\mu}} \frac{\partial W}{\partial \nu} \sqrt{\left[ \sum_{k=0}^{\infty} \binom{\frac{\mu}{1+\mu}k - \frac{5/2+\mu}{1+\mu}}{k} \left(W^{-\frac{2}{1+\mu}}\right)^k \right] \left[ \sum_{k=0}^{\infty} \binom{\frac{\mu}{1+\mu}k - \frac{1/2}{1+\mu}}{k} \left(W^{-\frac{2}{1+\mu}}\right)^k \right]} \\
&= \frac{R^2}{\sqrt{1+\mu}} \frac{W^{-\frac{3+\mu}{1+\mu}}}{1+\mu} \frac{\partial W}{\partial \nu} \sqrt{\left[ \sum_{k=0}^{\infty} \left(W^{-\frac{2}{1+\mu}}\right)^k \sum_{m=0}^k \binom{\frac{\mu}{1+\mu}m - \frac{5/2+\mu}{1+\mu}}{m} \binom{\frac{\mu}{1+\mu}(k-m) - \frac{1/2}{1+\mu}}{k-m} \right]} \\
&= \frac{R^2}{\sqrt{1+\mu}} \frac{W^{-\frac{3+\mu}{1+\mu}}}{1+\mu} \frac{\partial W}{\partial \nu} \sqrt{\left[ \sum_{k=0}^{\infty} \left(W^{-\frac{2}{1+\mu}}\right)^k \sum_{m=0}^k \binom{\frac{\mu}{1+\mu}m - \frac{5/2+\mu}{1+\mu} + \frac{2/2+\mu/2}{1+\mu}}{m} \binom{\frac{\mu}{1+\mu}(k-m) - \frac{1/2}{1+\mu} - \frac{2/2+\mu/2}{1+\mu}}{k-m} \right]} \\
&= \frac{R^2}{\sqrt{1+\mu}} \frac{W^{-\frac{3+\mu}{1+\mu}}}{1+\mu} \frac{\partial W}{\partial \nu} \sqrt{\left[ \sum_{k=0}^{\infty} \left(W^{-\frac{2}{1+\mu}}\right)^k \sum_{m=0}^k \binom{\frac{\mu}{1+\mu}m - \frac{3/2+\mu/2}{1+\mu}}{m} \binom{\frac{\mu}{1+\mu}(k-m) - \frac{3/2+\mu/2}{1+\mu}}{k-m} \right]} \\
&= \frac{R^2}{\sqrt{1+\mu}} \frac{W^{-\frac{3+\mu}{1+\mu}}}{1+\mu} \frac{\partial W}{\partial \nu} \sqrt{\left[ \sum_{k=0}^{\infty} \binom{\frac{\mu}{1+\mu}k - \frac{3/2+\mu/2}{1+\mu}}{k} \left(W^{-\frac{2}{1+\mu}}\right)^k \right]^2}
\end{aligned} \tag{E8}$$

where we used Cauchy product followed by Jensen identity (Gould 1972, No. 3.143, with  $t=[1+\mu/2]/[1+\mu]$ ), followed by the inverse of the Cauchy product. Then, the Jacobian is

$$J = h_R h_\nu h_\lambda = \frac{R^2 W^{-\frac{3+\mu}{1+\mu}}}{(1+\mu)^{\frac{3}{2}}} \frac{\partial W}{\partial \nu} \sum_{k=0}^{\infty} \binom{\frac{\mu}{1+\mu}(k - \frac{1}{2}) - \frac{3/2}{1+\mu}}{k} \left(W^{-\frac{2}{1+\mu}}\right)^k \tag{E9}$$

Also this result can be tested for  $\mu=0$ , for which the calculated Jacobian should be equivalent with the one for the spherical coordinates. For  $\mu=0$ ,  $W = \tan \nu$  and  $\partial W / \partial \nu = 1 / \cos^2 \nu$ . Therefore,

$$\begin{aligned}
J_{\mu=0} &= R^2 \tan^{-3} \nu \frac{1}{\cos^2 \nu} \sum_{k=0}^{\infty} \binom{-\frac{3}{2}}{k} (\tan^{-2} \nu)^k = R^2 \tan^{-3} \nu \frac{1}{\cos^2 \nu} (1 + \tan^{-2} \nu)^{-\frac{3}{2}} \\
&= R^2 \frac{\cos^3 \nu}{\sin^3 \nu} \frac{1}{\cos^2 \nu} \left( \frac{1}{\sin^2 \nu} \right)^{-\frac{3}{2}} = R^2 \frac{\cos \nu}{\sin^3 \nu} \frac{1}{\sin^{-3} \nu} = R^2 \cos \nu
\end{aligned} \tag{E10}$$

where the binomial theorem was used. This result is the same as for the small- $\nu$  region (and the same as the one for the spherical coordinates).

### Jacobian divided by the square of the $h_R$ scale factor for small- $\nu$ region

For the further use, we derive here also the Jacobian divided by the square of the  $h_R$  scale factor in the small- $\nu$  region. This quantity is needed in case of Laplacian calculation in SOS coordinates. We start with a division of Eq. (E4) by the squared Eq. (82):

$$\frac{J}{h_R^2} = \frac{\frac{R^2}{\sqrt{1+\mu}} \frac{\partial W}{\partial \nu} \sum_{k=0}^{\infty} \binom{-\mu(k+\frac{1}{2})-\frac{3}{2}}{k} (W^2)^k}{\sum_{k=0}^{\infty} \binom{-\mu k}{k} (W^2)^k} \tag{E11}$$

For the determination of the ratio of power series in (E11), Cauchy product formula can be used for expression of the power series in the numerator. We can write

$$\frac{\sum_{k=0}^{\infty} \binom{-\mu(k+\frac{1}{2})-\frac{3}{2}}{k} (W^2)^k}{\sum_{k=0}^{\infty} \binom{-\mu k}{k} (W^2)^k} = \sum_{k=0}^{\infty} \frac{a}{a+bk} \binom{a+bk}{k} (W^2)^k \quad (E12)$$

where the series on the right is selected in a suitable form to use Hagen-Rothe identity (Chu 2010, Chu 2013) later. If this Cauchy product is written in the standard form and then Hagen-Rothe summation formula is used, we get

$$\begin{aligned} \sum_{k=0}^{\infty} \binom{-\mu(k+\frac{1}{2})-\frac{3}{2}}{k} (W^2)^k &= \sum_{k=0}^{\infty} \binom{-\mu k}{k} (W^2)^k \sum_{k=0}^{\infty} \frac{a}{a+bk} \binom{a+bk}{k} (W^2)^k \\ &= \sum_{k=0}^{\infty} (W^2)^k \sum_{m=0}^k \frac{a}{a+bm} \binom{a+bm}{m} \binom{-\mu(k-m)}{k-m} = \sum_{k=0}^{\infty} (W^2)^k \binom{a+c}{k} \end{aligned} \quad (E13)$$

where the  $b, c$  terms in the Hagen-Rothe formula are clearly  $b=-\mu$ ,  $c=-\mu k$ , and – by comparison of the leftmost and the rightmost expressions – we can see that  $a=-\frac{1}{2}\mu-3/2$ . Therefore,

$$\frac{\sum_{k=0}^{\infty} \binom{-\mu(k+\frac{1}{2})-\frac{3}{2}}{k} (W^2)^k}{\sum_{k=0}^{\infty} \binom{-\mu k}{k} (W^2)^k} = \sum_{k=0}^{\infty} \frac{-\frac{\mu}{2}-\frac{3}{2}}{-\frac{\mu}{2}-\frac{3}{2}-\mu k} \binom{-\frac{\mu}{2}-\frac{3}{2}-\mu k}{k} (W^2)^k, \quad (E14)$$

and then

$$\frac{J}{h_R^2} = \frac{R^2}{\sqrt{1+\mu}} \frac{\partial W}{\partial v} \sum_{k=0}^{\infty} \frac{-\frac{\mu+3}{2}}{-\mu(k+\frac{1}{2})-\frac{3}{2}} \binom{-\mu(k+\frac{1}{2})-\frac{3}{2}}{k} (W^2)^k \quad (E15)$$

### Jacobian divided by the square of the $h_R$ scale factor for large- $v$ region

$J/h_R^2$  ratio derivation for large- $v$  region is carried out here in a similar way.

When we divide Eq. (E9) by the squared Eq. (85), we obtain:

$$\frac{J}{h_R^2} = \frac{\frac{R^2 W^{-\frac{3+\mu}{1+\mu}}}{(1+\mu)^{\frac{3}{2}}} \frac{\partial W}{\partial v} \sum_{k=0}^{\infty} \binom{\frac{\mu}{1+\mu}(k-\frac{1}{2})-\frac{3/2}{1+\mu}}{k} \left(W^{-\frac{2}{1+\mu}}\right)^k}{\frac{1}{1+\mu} \sum_{k=0}^{\infty} \binom{\frac{\mu}{1+\mu}k}{k} \left(W^{-\frac{2}{1+\mu}}\right)^k} \quad (E16)$$

For the determination of the ratio of power series in (E16), Cauchy product formula can be used for the expression of the power series in the numerator in such a way, that one term in the Cauchy product is the power series equal the one in the denominator. We can then write this ratio of the power series as

$$\frac{\sum_{k=0}^{\infty} \binom{\frac{\mu}{1+\mu}(k-\frac{1}{2})-\frac{3/2}{1+\mu}}{k} \left(W^{-\frac{2}{1+\mu}}\right)^k}{\sum_{k=0}^{\infty} \binom{\frac{\mu}{1+\mu}k}{k} \left(W^{-\frac{2}{1+\mu}}\right)^k} = \sum_{k=0}^{\infty} \frac{a}{a+bk} \binom{a+bk}{k} \left(W^{-\frac{2}{1+\mu}}\right)^k$$

(E17)

where the series on the right is selected in a suitable form to use Hagen-Rothe identity (Chu 2010, Chu 2013) later. If this Cauchy product is written in the standard form and then Hagen-Rothe summation formula is used, we get

$$\begin{aligned} \sum_{k=0}^{\infty} \binom{\frac{\mu}{1+\mu}(k-\frac{1}{2})-\frac{3/2}{1+\mu}}{k} \left(W^{-\frac{2}{1+\mu}}\right)^k &= \sum_{k=0}^{\infty} \binom{\frac{\mu}{1+\mu}k}{k} \left(W^{-\frac{2}{1+\mu}}\right)^k \sum_{k=0}^{\infty} \frac{a}{a+bk} \binom{a+bk}{k} \left(W^{-\frac{2}{1+\mu}}\right)^k \\ &= \sum_{k=0}^{\infty} \left(W^{-\frac{2}{1+\mu}}\right)^k \sum_{m=0}^k \frac{a}{a+bm} \binom{a+bm}{m} \binom{\frac{\mu}{1+\mu}(k-m)}{k-m} = \sum_{k=0}^{\infty} \left(W^{-\frac{2}{1+\mu}}\right)^k \binom{a+c}{k} \end{aligned} \quad (E18)$$

where the  $b, c$  terms in the Hagen-Rothe formula are clearly  $b=\mu/(1+\mu)$ ,  $c=\mu k/(1+\mu)$ , and – by comparison of the leftmost and the rightmost expressions – we can see that  $a=-(\mu/2+3/2)/(1+\mu)$ . Therefore,

$$\frac{\sum_{k=0}^{\infty} \binom{\frac{\mu}{1+\mu}(k-\frac{1}{2})-\frac{3/2}{1+\mu}}{k} \left(W^{-\frac{2}{1+\mu}}\right)^k}{\sum_{k=0}^{\infty} \binom{\frac{\mu}{1+\mu}k}{k} \left(W^{-\frac{2}{1+\mu}}\right)^k} = \sum_{k=0}^{\infty} \frac{-\frac{1}{2} \frac{\mu+3}{\mu+1}}{-\frac{1}{2} \frac{\mu+3}{1+\mu} + \frac{\mu}{1+\mu} k} \binom{-\frac{1}{2} \frac{\mu+3}{1+\mu} + \frac{\mu}{1+\mu} k}{k} \left(W^{-\frac{2}{1+\mu}}\right)^k, \quad (E19)$$

and then

$$\boxed{\frac{J}{h_R^2} = \frac{R^2}{\sqrt{1+\mu}} W^{-\frac{3+\mu}{1+\mu}} \frac{\partial W}{\partial v} \sum_{k=0}^{\infty} \frac{-\frac{1}{2} \frac{\mu+3}{\mu+1}}{-\frac{1}{2} \frac{\mu+3}{1+\mu} + \frac{\mu}{1+\mu} k} \binom{-\frac{1}{2} \frac{\mu+3}{1+\mu} + \frac{\mu}{1+\mu} k}{k} \left(W^{-\frac{2}{1+\mu}}\right)^k} \quad (E20)$$

in the large- $v$  region.
