# Supplementary material for: Analytical Solution of Similar Oblate Spheroidal Coordinate System
Source: arXiv:2109.12057 ancillary file (2021-09-06)
Supplement: Supplementary file 5 [file Supplement_SOS_F.pdf]

# Analytical solution of Similar Oblate Spheroidal Coordinate System

---

Pavel Strunz

Nuclear Physics Institute of the CAS, Řež, Czech Republic

e-mail: strunz@ujf.cas.cz

## Supplement F

### Expression of the terms containing derivatives of the metric scale factors in the advection formula by using metric scale factors.

In order to write the components of the momentum equation in the curvilinear orthogonal system, the decomposition of the velocity advection term

$$-(\mathbf{u} \cdot \nabla)\mathbf{u} = \mathbf{u} \times (\nabla \times \mathbf{u}) - \nabla\left(\frac{\mathbf{u}^2}{2}\right) \quad (\text{F1})$$

into its components is required. The components of the advection term are

$$-[(\mathbf{u} \cdot \nabla)\mathbf{u}]_R = \frac{u_v}{h_R h_v} \left( u_v \frac{\partial h_v}{\partial R} - u_R \frac{\partial h_R}{\partial v} \right) + \frac{u_\lambda}{h_R h_\lambda} \left( u_\lambda \frac{\partial h_\lambda}{\partial R} - u_R \frac{\partial h_R}{\partial \lambda} \right) - (\mathbf{u} \cdot \nabla)u_R \quad (\text{F2a})$$

$$-[(\mathbf{u} \cdot \nabla)\mathbf{u}]_v = \frac{u_\lambda}{h_v h_\lambda} \left( u_\lambda \frac{\partial h_\lambda}{\partial v} - u_v \frac{\partial h_v}{\partial \lambda} \right) + \frac{u_R}{h_v h_R} \left( u_R \frac{\partial h_R}{\partial v} - u_v \frac{\partial h_v}{\partial R} \right) - (\mathbf{u} \cdot \nabla)u_v \quad (\text{F2b})$$

$$-[(\mathbf{u} \cdot \nabla)\mathbf{u}]_\lambda = \frac{u_R}{h_\lambda h_R} \left( u_R \frac{\partial h_R}{\partial \lambda} - u_\lambda \frac{\partial h_\lambda}{\partial R} \right) + \frac{u_v}{h_\lambda h_v} \left( u_v \frac{\partial h_v}{\partial \lambda} - u_\lambda \frac{\partial h_\lambda}{\partial v} \right) - (\mathbf{u} \cdot \nabla)u_\lambda. \quad (\text{F2c})$$

As the partial derivatives of the metric scale factors with respect to  $\lambda$  are zero, the expressions simplify to

$$-[(\mathbf{u} \cdot \nabla)\mathbf{u}]_R = \frac{u_v}{h_R h_v} \left( u_v \frac{\partial h_v}{\partial R} - u_R \frac{\partial h_R}{\partial v} \right) + \frac{u_\lambda}{h_R h_\lambda} u_\lambda \frac{\partial h_\lambda}{\partial R} - (\mathbf{u} \cdot \nabla)u_R \quad (\text{F3a})$$

$$-[(\mathbf{u} \cdot \nabla)\mathbf{u}]_v = \frac{u_\lambda}{h_v h_\lambda} u_\lambda \frac{\partial h_\lambda}{\partial v} + \frac{u_R}{h_v h_R} \left( u_R \frac{\partial h_R}{\partial v} - u_v \frac{\partial h_v}{\partial R} \right) - (\mathbf{u} \cdot \nabla)u_v \quad (\text{F3b})$$

$$-[(\mathbf{u} \cdot \nabla)\mathbf{u}]_\lambda = -\frac{u_R}{h_\lambda h_R} u_\lambda \frac{\partial h_\lambda}{\partial R} - \frac{u_v}{h_\lambda h_v} u_\lambda \frac{\partial h_\lambda}{\partial v} - (\mathbf{u} \cdot \nabla)u_\lambda \quad (\text{F3c})$$

It can be seen that the individual terms contain derivatives of the metric scale factors. There is eight terms containing such derivatives to be determined. Nevertheless, the unique coefficients in these terms containing only metric scale factors and their derivative are only four:

$$\frac{1}{h_R h_\lambda} \frac{\partial h_\lambda}{\partial R}, \quad \frac{1}{h_v h_\lambda} \frac{\partial h_\lambda}{\partial v}, \quad \frac{1}{h_R h_v} \frac{\partial h_v}{\partial R}, \quad \frac{1}{h_R h_v} \frac{\partial h_R}{\partial v}. \quad (\text{F4})$$

It would be certainly useful to express the whole terms, or at least the derivatives in it, with the help of the already known expressions for  $h_R$ ,  $h_v$  and  $h_\lambda$  (see the expressions (80), (81), (82), (85), (88) and (89)). This is done in the following paragraphs.

***Small- $v$  region, term containing  $\partial h_\lambda / \partial R$***

As the first derivation, we evaluate  $\frac{\partial h_\lambda}{\partial R}$  in **the small- $v$  region**.

$$\frac{\partial h_\lambda}{\partial R} = \frac{\partial}{\partial R} \left[ \frac{R}{2} \sum_{k=0}^{\infty} \binom{-\frac{1}{2}-\mu k}{k} \frac{-(W^2)^k}{-\frac{1}{2}-\mu k} \right] = \frac{1}{2} \sum_{k=0}^{\infty} \binom{-\frac{1}{2}-\mu k}{k} \frac{-(2\mu k+1)}{-\frac{1}{2}-\mu k} (W^2)^k = \sum_{k=0}^{\infty} \binom{-\frac{1}{2}-\mu k}{k} (W^2)^k \quad (\text{F5})$$

where the formula (22) for  $W$  was used. By using  $h_\lambda$  (see (80)) and using similar way as done in **Supplement E**, expressions (E12), (E13) and (E14), for computing the ratio of sums, we arrive at:

$$\frac{1}{h_R h_\lambda} \frac{\partial h_\lambda}{\partial R} = \frac{\sum_{k=0}^{\infty} \binom{-\frac{1}{2}-\mu k}{k} (W^2)^k}{h_R R \sum_{k=0}^{\infty} \binom{-\frac{1}{2}-\mu k}{k} \frac{-\frac{1}{2}}{-\frac{1}{2}-\mu k} (W^2)^k} = \frac{\sum_{k=0}^{\infty} \binom{-\mu k}{k} (W^2)^k}{h_R R} = \frac{h_R^2}{h_R R} = \frac{h_R}{R} \quad (\text{F6})$$

Although we achieved the goal in this subsection (derivation of the coefficient containing  $\frac{\partial h_\lambda}{\partial R}$  derivative, it is also of advantage to derive the square of the derivative. With the help of Cauchy product and Jensen binomial identity (listed in **Gould 1972** collection of combinatorial identities under the number 3.143), we have:

$$\left( \frac{\partial h_\lambda}{\partial R} \right)^2 = \left[ \sum_{k=0}^{\infty} \binom{-\frac{1}{2}-\mu k}{k} (W^2)^k \right] \left[ \sum_{k=0}^{\infty} \binom{-\frac{1}{2}-\mu k}{k} (W^2)^k \right] = \sum_{k=0}^{\infty} \left[ (W^2)^k \sum_{m=0}^k \binom{-\frac{1}{2}-\mu m}{m} \binom{-\frac{1}{2}-\mu(k-m)}{k-m} \right] = \sum_{k=0}^{\infty} \left[ (W^2)^k \sum_{m=0}^k \binom{-\mu m}{m} \binom{-1-\mu(k-m)}{k-m} \right] = \left[ \sum_{k=0}^{\infty} \binom{-\mu k}{k} (W^2)^k \right] \left[ \sum_{k=0}^{\infty} \binom{-1-\mu k}{k} (W^2)^k \right] \quad (\text{F7})$$

where the inverse Cauchy product was used as the last manipulation.

By comparison with  $h_R$  metric scale factor, we see

$$\left( \frac{\partial h_\lambda}{\partial R} \right)^2 = h_R^2 \left[ \sum_{k=0}^{\infty} \binom{-1-\mu k}{k} (W^2)^k \right] = h_R^2 \left[ 1 + \sum_{k=1}^{\infty} \binom{-1-\mu k}{k} (W^2)^k \right] \quad (\text{F8})$$

Further derivation is split to the case when  $\mu \neq 0$  and when  $\mu = 0$  in order to avoid division by 0.

When  $\mu \neq 0$ , we can use (A3) identity from **Supplement A**, and arrive at

$$\left( \frac{\partial h_\lambda}{\partial R} \right)^2 = h_R^2 \left[ 1 + \sum_{k=1}^{\infty} \binom{-\mu k}{k} \frac{-k(\mu+1)}{-\mu k} (W^2)^k \right] = h_R^2 \left[ 1 + \frac{\mu+1}{\mu} \sum_{k=1}^{\infty} \binom{-\mu k}{k} (W^2)^k \right] = h_R^2 \frac{\mu+1}{\mu} \left[ \frac{\mu}{\mu+1} - 1 + \sum_{k=0}^{\infty} \binom{-\mu k}{k} (W^2)^k \right] = h_R^2 \frac{\mu+1}{\mu} \left[ -\frac{1}{\mu+1} + h_R^2 \right] = h_R^2 \left( \frac{\mu+1}{\mu} h_R^2 - \frac{1}{\mu} \right) \quad (\text{F9})$$

When  $\mu = 0$ , then it follows from (82), (22), (F8) and from binomial theorem that

$$h_R^2 = \sum_{k=0}^{\infty} \binom{0}{k} (\tan^2 v)^k = 1 \quad \text{and} \quad \left( \frac{\partial h_\lambda}{\partial R} \right)^2 = h_R^2 \left[ \sum_{k=0}^{\infty} \binom{-1}{k} (\tan^2 v)^k \right] = (1 + \tan^2 v)^{-1} = \cos^2 v \quad (\text{F10})$$

which is, as expected, equivalent to the result for spherical coordinates.

When  $\mu \neq 0$ , we finally have with help of (F9)

$$\frac{1}{h_R h_\lambda} \frac{\partial h_\lambda}{\partial R} = \frac{1}{h_\lambda} \sqrt{\frac{\mu+1}{\mu} h_R^2 - \frac{1}{\mu}} \quad (\text{F11})$$

By comparison with (F6), it follows that we can write for  $\mu \neq 0$  the relation

$$\frac{h_\lambda^2}{R^2} = \frac{\mu+1}{\mu} - \frac{1}{\mu h_R^2} \quad (\text{F12})$$

### **Small- $v$ region, term containing $\partial h_\lambda / \partial v$**

As the second step, we can employ the previous result for  $\frac{\partial h_\lambda}{\partial R}$  and the formula (20) from the main text for  $\frac{\partial h_\lambda}{\partial v}$  determination in **the small- $v$  region**. It follows from (20) and (F6) that

$$\frac{\partial h_\lambda}{\partial v} = -\frac{h_v}{h_R} \sqrt{h_R^2 - \left( \frac{\partial h_\lambda}{\partial R} \right)^2} = -\frac{h_v}{h_R} \sqrt{h_R^2 - \left( \frac{h_R^2 h_\lambda^2}{R^2} \right)^2} = -h_v \sqrt{1 - \frac{h_R^2 h_\lambda^2}{R^2}} \quad (\text{F13})$$

Then

$$\frac{1}{h_\nu h_\lambda} \frac{\partial h_\lambda}{\partial \nu} = -\frac{1}{h_\lambda} \sqrt{1 - \frac{h_R^2 h_\lambda^2}{R^2}} = -\sqrt{\frac{1}{h_\lambda^2} - \frac{h_R^2}{R^2}} \quad (\text{F14})$$

### *Small- $\nu$ region, term containing $\partial h_\nu / \partial R$*

Before proceeding to the final derivation, we first find some preliminary identities:

$$\frac{\partial(h_\nu^2/h_R^2)}{\partial R} = \frac{1}{h_R^4} \left( h_R^2 \frac{\partial h_\nu^2}{\partial R} - h_\nu^2 \frac{\partial h_R^2}{\partial R} \right) \Rightarrow \frac{\partial h_\nu^2}{\partial R} = h_R^2 \frac{\partial(h_\nu^2/h_R^2)}{\partial R} + \frac{h_\nu^2}{h_R^2} \frac{\partial h_R^2}{\partial R} \quad (\text{F15})$$

In the same way as done in **Supplement E**, expressions (E12), (E13) and (E14), it is possible to derive the ratio of squared scale factors  $h_R$  and  $h_\nu$  (given by (82) and (88))

$$\frac{h_\nu^2}{h_R^2} = \frac{\frac{R^2}{1+\mu} \left( \frac{\partial W}{\partial \nu} \right)^2 \sum_{k=0}^{\infty} \binom{-(\mu+2)-\mu k}{k} (W^2)^k}{\sum_{k=0}^{\infty} \binom{-\mu k}{k} (W^2)^k} = \frac{R^2}{1+\mu} \left( \frac{\partial W}{\partial \nu} \right)^2 \sum_{k=0}^{\infty} \frac{-(\mu+2)}{-(\mu+2)-\mu k} \binom{-(\mu+2)-\mu k}{k} (W^2)^k \quad (\text{F16})$$

Further, we can derive the derivative of this ratio with respect to  $R$  by a smart manipulation:

$$\begin{aligned} \frac{\partial(h_\nu^2/h_R^2)}{\partial R} &= \frac{\partial}{\partial R} \left[ R^{-2} R^2 \frac{h_\nu^2}{h_R^2} \right] = -2R^{-3} R^2 \frac{h_\nu^2}{h_R^2} + R^{-2} \frac{\partial}{\partial R} \left[ R^2 \frac{R^2}{1+\mu} \left( \frac{\partial W}{\partial \nu} \right)^2 \sum_{k=0}^{\infty} \frac{-(\mu+2)}{-(\mu+2)-\mu k} \binom{-(\mu+2)-\mu k}{k} (W^2)^k \right] = \\ &= -\frac{2}{R} \frac{h_\nu^2}{h_R^2} + \frac{1}{R^2} \left[ \frac{R^3}{1+\mu} \left( \frac{\partial W}{\partial \nu} \right)^2 \sum_{k=0}^{\infty} \frac{-(\mu+2)}{-(\mu+2)-\mu k} \binom{-(\mu+2)-\mu k}{k} (2\mu k + 2\mu + 4) (W^2)^k \right] = \\ &= -\frac{2}{R} \frac{h_\nu^2}{h_R^2} + \frac{2(\mu+2)}{R} \frac{R^2}{1+\mu} \left( \frac{\partial W}{\partial \nu} \right)^2 \sum_{k=0}^{\infty} \binom{-(\mu+2)-\mu k}{k} (W^2)^k = -\frac{2}{R} \frac{h_\nu^2}{h_R^2} + \frac{2(\mu+2)}{R} h_\nu^2 = \frac{2h_\nu^2}{R} \left( \mu + 2 - \frac{1}{h_R^2} \right). \end{aligned} \quad (\text{F17})$$

Final relation we need is Eq. (83) which tells that

$$h_R^2 = \left[ (1+\mu) + \mu \sum_{k=0}^{\infty} \binom{-1-\mu k}{k} \frac{(W^2)^k}{-1-\mu k} \right]^{-1} = \frac{1}{g} \quad \text{where} \quad g = \frac{1}{h_R^2} = (1+\mu) + \mu \sum_{k=0}^{\infty} \binom{-1-\mu k}{k} \frac{(W^2)^k}{-1-\mu k} \quad (\text{F18})$$

and thus

$$\begin{aligned} \frac{\partial h_R^2}{\partial R} &= \frac{\partial}{\partial R} \left( \frac{1}{g} \right) = -\frac{1}{g^2} \frac{\partial g}{\partial R} = -\frac{1}{\frac{1}{h_R^4}} \frac{\partial}{\partial R} \left[ (1+\mu) + \mu \sum_{k=0}^{\infty} \binom{-1-\mu k}{k} \frac{(W^2)^k}{-1-\mu k} \right] = \\ &= -h_R^4 \left[ \mu \sum_{k=0}^{\infty} \binom{-1-\mu k}{k} \frac{2\mu k}{-1-\mu k} \frac{1}{R} (W^2)^k \right] = -h_R^4 \frac{2\mu^2}{R} \left[ 0 + \sum_{k=1}^{\infty} \binom{-1-\mu k}{k} \frac{k}{-1-\mu k} (W^2)^k \right] \quad (\text{F19}) \end{aligned}$$

After the use of (A4) identity from **Supplement A**, and subsequently the identity (A3), we arrive at

$$\begin{aligned} \frac{\partial h_R^2}{\partial R} &= -h_R^4 \frac{2\mu^2}{R} \sum_{k=1}^{\infty} \binom{-1-\mu k}{k-1} \frac{-k(1+\mu)}{k} \frac{k}{-1-\mu k} (W^2)^k = \\ &= -h_R^4 \frac{2\mu^2}{R} \sum_{M=0}^{\infty} \binom{-1-\mu(M+1)}{M} \frac{-(M+1)(1+\mu)}{-1-\mu(M+1)} (W^2)^{M+1} = \\ &= -h_R^4 \frac{2\mu^2}{R} \sum_{M=0}^{\infty} \binom{-(\mu+2)-\mu M}{M} \frac{-(1+\mu)-M(1+\mu)}{-\mu-1-M(\mu+1)} (W^2)^{M+1} = -h_R^4 \frac{2\mu^2}{R} W^2 \sum_{M=0}^{\infty} \binom{-(\mu+2)-\mu M}{M} (W^2)^M = \\ &= -h_R^4 \frac{2\mu^2}{R} W^2 \frac{h_\nu^2}{\frac{R^2}{1+\mu} \left( \frac{\partial W}{\partial \nu} \right)^2} = -\frac{2(1+\mu)\mu^2}{R^3} h_R^4 h_\nu^2 \frac{W^2}{\left( \frac{\partial W}{\partial \nu} \right)^2} \quad (\text{F20}) \end{aligned}$$

Now, we have all the relations (see (F17) and (F20)) needed to finalize the relation from (F15)

$$\begin{aligned} \frac{\partial h_\nu^2}{\partial R} &= h_R^2 \frac{\partial(h_\nu^2/h_R^2)}{\partial R} + \frac{h_\nu^2}{h_R^2} \frac{\partial h_R^2}{\partial R} = h_R^2 \frac{2h_\nu^2}{R} \left( \mu + 2 - \frac{1}{h_R^2} \right) - \frac{h_\nu^2}{h_R^2} \frac{2(1+\mu)\mu^2}{R^3} h_R^4 h_\nu^2 \frac{W^2}{\left( \frac{\partial W}{\partial \nu} \right)^2} = \\ &= \frac{2}{R} h_R^2 h_\nu^2 \left( \mu + 2 - \frac{1}{h_R^2} \right) - \frac{2(1+\mu)\mu^2}{R^3} h_R^2 h_\nu^4 \left( \frac{\sin \nu \cos \nu}{1+\mu \sin^2 \nu} \right)^2, \end{aligned} \quad (\text{F21})$$

and thus

$$\frac{1}{h_R h_v} \frac{\partial h_v}{\partial R} = \frac{h_R}{2 h_R^2 h_v^2} \frac{\partial h_v^2}{\partial R} = \frac{h_R}{2} \left[ \frac{2(\mu+2)}{R} - \frac{2}{R h_R^2} - \frac{2(1+\mu)\mu^2}{R^3} h_v^2 \left( \frac{\sin v \cos v}{1+\mu \sin^2 v} \right)^2 \right] = \frac{1}{R} \left[ (\mu+2) h_R - \frac{1}{h_R} - \frac{(1+\mu)\mu^2}{R^2} \left( \frac{\sin v \cos v}{1+\mu \sin^2 v} \right)^2 h_R h_v^2 \right] , \quad (\text{F22})$$

### *Small- $v$ region, term containing $\partial h_R / \partial v$*

When we again use Eq. (83), we arrive - for the derivative of the squared  $h_R$  with respect to  $v$  - to

$$\frac{\partial h_R^2}{\partial v} = \frac{\partial}{\partial v} \left( \frac{1}{g} \right) = - \frac{1}{g^2} \frac{\partial g}{\partial v} = - \frac{1}{h_R^4} \frac{\partial}{\partial v} \left[ (1+\mu) + \mu \sum_{k=0}^{\infty} \binom{-1-\mu k}{k} \frac{(W^2)^k}{-1-\mu k} \right] = -h_R^4 \left[ \mu \sum_{k=0}^{\infty} \binom{-1-\mu k}{k} \frac{2k}{-1-\mu k} (W^2)^k \frac{1}{W} \frac{\partial W}{\partial v} \right] = -2\mu h_R^4 \frac{1}{W} \frac{\partial W}{\partial v} \left[ 0 + \sum_{k=1}^{\infty} \binom{-1-\mu k}{k} \frac{k}{-1-\mu k} (W^2)^k \right] . \quad (\text{F23})$$

After the use of (A4) identity from **Supplement A**, and subsequently the identity (A3) in a similar way as for (F20), we arrive at

$$\frac{\partial h_R^2}{\partial v} = - \frac{2\mu(1+\mu)}{R^2} \frac{W}{\frac{\partial W}{\partial v}} h_R^4 h_v^2 . \quad (\text{F24})$$

Thus

$$\frac{1}{h_R h_v} \frac{\partial h_R}{\partial v} = \frac{1}{2 h_R^2 h_v} \frac{\partial h_R^2}{\partial v} = - \frac{\mu(1+\mu)}{R^2} \frac{W}{\frac{\partial W}{\partial v}} h_R^2 h_v = - \frac{\mu(1+\mu)}{R^2} \frac{\sin v \cos v}{1+\mu \sin^2 v} h_R^2 h_v , \quad (\text{F25})$$

### *Large- $v$ region, term containing $\partial h_\lambda / \partial R$*

$\frac{\partial h_\lambda}{\partial R}$  in the large- $v$  region is evaluated in a similar way as in the small- $v$  region:

$$\begin{aligned} \frac{\partial h_\lambda}{\partial R} &= \frac{\partial}{\partial R} \left[ \frac{W^{-\frac{1}{1+\mu}}}{1+\mu} \frac{R}{2} \sum_{k=0}^{\infty} \binom{-\frac{1}{2(1+\mu)} + \frac{\mu}{1+\mu} k}{k} \frac{-\left(W^{-\frac{2}{1+\mu}}\right)^k}{-\frac{1}{2(1+\mu)} + \frac{\mu}{1+\mu} k} \right] = \\ &= \frac{1}{2} \frac{W^{-\frac{1}{1+\mu}}}{1+\mu} \sum_{k=0}^{\infty} \binom{-\frac{1}{2(1+\mu)} + \frac{\mu}{1+\mu} k}{k} \frac{-\left(-\frac{2\mu k}{1+\mu} - \frac{\mu}{1+\mu} + 1\right)}{-\frac{1}{2(1+\mu)} + \frac{\mu}{1+\mu} k} \left(W^{-\frac{2}{1+\mu}}\right)^k = \\ &= \frac{W^{-\frac{1}{1+\mu}}}{1+\mu} \sum_{k=0}^{\infty} \binom{-\frac{1}{2(1+\mu)} + \frac{\mu}{1+\mu} k}{k} \frac{-\left(-\frac{2\mu k}{1+\mu} + \frac{1}{1+\mu}\right)}{-\frac{1}{1+\mu} + \frac{2\mu}{1+\mu} k} \left(W^{-\frac{2}{1+\mu}}\right)^k = \frac{W^{-\frac{1}{1+\mu}}}{1+\mu} \sum_{k=0}^{\infty} \binom{-\frac{1}{2(1+\mu)} + \frac{\mu}{1+\mu} k}{k} \left(W^{-\frac{2}{1+\mu}}\right)^k \quad (\text{F26}) \end{aligned}$$

where the formula (22) from the main text, showing  $R^\mu$  dependence of  $W$ , has to be observed. By using  $h_\lambda$  (see (81)) and using similar way as done in **Supplement E**, expressions (E17), (E18) and (E19), for computing the ratio of sums (i.e. using Cauchy product and Hagen-Rothe identity (Chu 2013)), we arrive at

$$\frac{1}{h_R h_\lambda} \frac{\partial h_\lambda}{\partial R} = \frac{\frac{W^{-\frac{1}{1+\mu}}}{1+\mu} \sum_{k=0}^{\infty} \binom{-\frac{1}{2(1+\mu)} + \frac{\mu}{1+\mu} k}{k} \left(W^{-\frac{2}{1+\mu}}\right)^k}{h_R \frac{W^{-\frac{1}{1+\mu}}}{1+\mu} R \sum_{k=0}^{\infty} \binom{-\frac{1}{2(1+\mu)} + \frac{\mu}{1+\mu} k}{k} \frac{-\left(W^{-\frac{2}{1+\mu}}\right)^k}{-\frac{1}{2(1+\mu)} + \frac{\mu}{1+\mu} k}} = \frac{\frac{1}{1+\mu} \sum_{k=0}^{\infty} \binom{-\frac{1}{2(1+\mu)} + \frac{\mu}{1+\mu} k}{k} \left(W^{-\frac{2}{1+\mu}}\right)^k}{h_R R \sum_{k=0}^{\infty} \binom{-\frac{1}{2(1+\mu)} + \frac{\mu}{1+\mu} k}{k} \frac{-\frac{1}{2(1+\mu)}}{-\frac{1}{2(1+\mu)} + \frac{\mu}{1+\mu} k} \left(W^{-\frac{2}{1+\mu}}\right)^k} = \frac{\frac{1}{1+\mu} \sum_{k=0}^{\infty} \binom{\frac{\mu}{1+\mu} k}{k} \left(W^{-\frac{2}{1+\mu}}\right)^k}{h_R R} = \frac{h_R^2}{h_R R} = \frac{h_R}{R}, \quad (\text{F27})$$

i.e. a relation which has the form identical to the relation in the small- $v$  region.

Although we achieved the goal in this subsection (derivation of the coefficient containing  $\frac{\partial h_\lambda}{\partial R}$  derivative), it is also of advantage to derive the square of the derivative. With the help of Cauchy product and Jensen binomial identity (listed in [Gould 1972](#) collection of combinatorial identities under the number 3.143), we have:

$$\begin{aligned} \left(\frac{\partial h_\lambda}{\partial R}\right)^2 &= \left[ \frac{W^{-\frac{1}{1+\mu}}}{1+\mu} \sum_{k=0}^{\infty} \binom{-\frac{1}{2(1+\mu)} + \frac{\mu}{1+\mu} k}{k} \left(W^{-\frac{2}{1+\mu}}\right)^k \right] \left[ \frac{W^{-\frac{1}{1+\mu}}}{1+\mu} \sum_{k=0}^{\infty} \binom{-\frac{1}{2(1+\mu)} + \frac{\mu}{1+\mu} k}{k} \left(W^{-\frac{2}{1+\mu}}\right)^k \right] = \\ &= \frac{W^{-\frac{2}{1+\mu}}}{(1+\mu)^2} \sum_{k=0}^{\infty} \left[ \left(W^{-\frac{2}{1+\mu}}\right)^k \sum_{m=0}^k \binom{-\frac{1}{2(1+\mu)} + \frac{\mu}{1+\mu} m}{m} \binom{-\frac{1}{2(1+\mu)} + \frac{\mu}{1+\mu} (k-m)}{k-m} \right] = \\ &= \frac{W^{-\frac{2}{1+\mu}}}{(1+\mu)^2} \sum_{k=0}^{\infty} \left[ \left(W^{-\frac{2}{1+\mu}}\right)^k \sum_{m=0}^k \binom{\frac{\mu}{1+\mu} m}{m} \binom{-\frac{1}{1+\mu} + \frac{\mu}{1+\mu} (k-m)}{k-m} \right] = \\ &= \frac{W^{-\frac{2}{1+\mu}}}{(1+\mu)^2} \left[ \sum_{k=0}^{\infty} \binom{\frac{\mu}{1+\mu} k}{k} \left(W^{-\frac{2}{1+\mu}}\right)^k \right] \left[ \sum_{k=0}^{\infty} \binom{-\frac{1}{1+\mu} + \frac{\mu}{1+\mu} k}{k} \left(W^{-\frac{2}{1+\mu}}\right)^k \right] \quad (\text{F28}) \end{aligned}$$

By comparison of the first sum with  $h_R$  metric scale factor (see (85)), by re-indexing of the second sum ( $M=k+1$ ), and by the use of (A4) identity from **Supplement A**, we see that

$$\begin{aligned} \left(\frac{\partial h_\lambda}{\partial R}\right)^2 &= \frac{W^{-\frac{2}{1+\mu}}}{1+\mu} h_R^2 \left[ \sum_{k=0}^{\infty} \binom{-\frac{1}{1+\mu} + \frac{\mu}{1+\mu} k}{k} \left(W^{-\frac{2}{1+\mu}}\right)^k \right] = \frac{W^{-\frac{2}{1+\mu}}}{1+\mu} h_R^2 \left[ \sum_{k=0}^{\infty} \binom{\frac{\mu}{1+\mu} (k+1)-1}{k} \left(W^{-\frac{2}{1+\mu}}\right)^k \right] = \\ &= \frac{W^{-\frac{2}{1+\mu}}}{1+\mu} h_R^2 \left[ \sum_{M=1}^{\infty} \binom{\frac{\mu}{1+\mu} M-1}{M-1} \left(W^{-\frac{2}{1+\mu}}\right)^{M-1} \right] = \frac{1}{1+\mu} h_R^2 \left[ \sum_{M=1}^{\infty} \binom{\frac{\mu}{1+\mu} M-1}{M} \frac{M}{\frac{\mu}{1+\mu} M-M} \left(W^{-\frac{2}{1+\mu}}\right)^M \right] = \\ &= \frac{1}{1+\mu} h_R^2 \left[ \sum_{M=1}^{\infty} \binom{\frac{\mu}{1+\mu} M-1}{M} (-1)(1+\mu) \left(W^{-\frac{2}{1+\mu}}\right)^M \right]. \quad (\text{F29}) \end{aligned}$$

Further derivation is split to the case when  $\mu \neq 0$  and when  $\mu = 0$  in order to avoid division by 0.

When  $\mu \neq 0$ , we can use (A3) identity from **Supplement A**, and arrive at

$$\begin{aligned} \left(\frac{\partial h_\lambda}{\partial R}\right)^2 &= \frac{1}{1+\mu} h_R^2 \left[ \sum_{M=1}^{\infty} \binom{\frac{\mu}{1+\mu} M}{M} \frac{-1}{\frac{\mu}{1+\mu} M} (-1)(1+\mu) \left(W^{-\frac{2}{1+\mu}}\right)^M \right] = \\ &= \frac{1}{1+\mu} h_R^2 \frac{1}{\mu} (1+\mu) \left[ \sum_{M=1}^{\infty} \binom{\frac{\mu}{1+\mu} M}{M} \left(W^{-\frac{2}{1+\mu}}\right)^M \right] = \frac{1}{1+\mu} h_R^2 \frac{1}{\mu} (1+\mu) \left[ -1 + \sum_{M=0}^{\infty} \binom{\frac{\mu}{1+\mu} M}{M} \left(W^{-\frac{2}{1+\mu}}\right)^M \right] = \\ &= h_R^2 \frac{1}{\mu} (1+\mu) \left[ -\frac{1}{1+\mu} + \frac{1}{1+\mu} \sum_{M=0}^{\infty} \binom{\frac{\mu}{1+\mu} M}{M} \left(W^{-\frac{2}{1+\mu}}\right)^M \right] = h_R^2 \frac{1}{\mu} (1+\mu) \left[ -\frac{1}{1+\mu} + h_R^2 \right] = h_R^2 \left[ \frac{1+\mu}{\mu} h_R^2 - \frac{1}{\mu} \right] \quad (\text{F30}) \end{aligned}$$

When compared with the small- $v$  region, we can see that the form of the squared derivative is identical.

When  $\mu=0$ , then it follows from (85), (22), (F29) and from the binomial theorem that

$$h_R^2 = \sum_{k=0}^{\infty} \binom{0}{k} (\tan^{-2} \nu)^k = 1 \quad \text{and} \quad \left( \frac{\partial h_\lambda}{\partial R} \right)^2 = h_R^2 \left[ \sum_{M=1}^{\infty} \binom{-1}{M} (-1)^M (\tan^{-2} \nu)^M \right] = 1 \left[ 1 - \sum_{M=0}^{\infty} \binom{-1}{M} (\tan^{-2} \nu)^M \right] = 1 - (1 + \tan^{-2} \nu)^{-1} = \cos^2 \nu \quad (\text{F31})$$

which is, as expected, equivalent to the result for spherical coordinates.

When  $\mu \neq 0$ , we finally have with help of (F30) the relation

$$\frac{1}{h_R h_\lambda} \frac{\partial h_\lambda}{\partial R} = \frac{1}{h_\lambda} \sqrt{\frac{\mu+1}{\mu} h_R^2 - \frac{1}{\mu}} \quad (\text{F32})$$

By comparison with (F27), it follows that we can write, for  $\mu \neq 0$ , also in the large- $\nu$  region the relation

$$\frac{h_\lambda^2}{R^2} = \frac{\mu+1}{\mu} - \frac{1}{\mu h_R^2} \quad (\text{F33})$$

### ***Large- $\nu$ region, term containing $\partial h_\lambda / \partial \nu$***

We can employ the previous result for  $\frac{\partial h_\lambda}{\partial R}$  and the formula (20) from the main text for  $\frac{\partial h_\lambda}{\partial \nu}$  determination in **the large- $\nu$  region**. It follows from (20) and (F27) that

$$\frac{\partial h_\lambda}{\partial \nu} = -\frac{h_\nu}{h_R} \sqrt{h_R^2 - \left( \frac{\partial h_\lambda}{\partial R} \right)^2} = -\frac{h_\nu}{h_R} \sqrt{h_R^2 - \left( \frac{h_R^2 h_\lambda^2}{R^2} \right)^2} = -h_\nu \sqrt{1 - \frac{h_R^2 h_\lambda^2}{R^2}} \quad (\text{F34})$$

also in the **the large- $\nu$  region**. Then

$$\frac{1}{h_\nu h_\lambda} \frac{\partial h_\lambda}{\partial \nu} = -\frac{1}{h_\lambda} \sqrt{1 - \frac{h_R^2 h_\lambda^2}{R^2}} = -\sqrt{\frac{1}{h_\lambda^2} - \frac{h_R^2}{R^2}} \quad (\text{F35})$$

### ***Large- $\nu$ region, term containing $\partial h_\nu / \partial R$***

Before proceeding to the final derivation, we first find some preliminary identities.

Expression (F15) is valid also in the large- $\nu$  region.

In the same way as done in **Supplement E**, expressions (E17), (E18) and (E19), it is possible to derive the ratio of squared scale factors  $h_R$  and  $h_\nu$  (given by (85) and (88))

$$\frac{h_\nu^2}{h_R^2} = \frac{\frac{R^2}{(1+\mu)^2} W^{-2 \frac{2+\mu}{1+\mu}} \left( \frac{\partial W}{\partial \nu} \right)^2 \sum_{k=0}^{\infty} \binom{\frac{\mu}{1+\mu} k - \frac{2+\mu}{1+\mu}}{k} \left( W^{-\frac{2}{1+\mu}} \right)^k}{\frac{1}{1+\mu} \sum_{k=0}^{\infty} \binom{\frac{\mu}{1+\mu} k}{k} \left( W^{-\frac{2}{1+\mu}} \right)^k} = \frac{\frac{R^2}{1+\mu} W^{-2 \frac{2+\mu}{1+\mu}} \left( \frac{\partial W}{\partial \nu} \right)^2 \sum_{k=0}^{\infty} \frac{-\frac{2+\mu}{1+\mu}}{-\frac{2+\mu}{1+\mu} + \frac{\mu}{1+\mu} k} \binom{-\frac{2+\mu}{1+\mu} + \frac{\mu}{1+\mu} k}{k} \left( W^{-\frac{2}{1+\mu}} \right)^k}{}, \quad (\text{F36})$$

Further, we can derive the derivative of this ratio with respect to  $R$  by a smart manipulation:

$$\begin{aligned} \frac{\partial (h_\nu^2 / h_R^2)}{\partial R} &= \frac{\partial}{\partial R} \left[ R^{-2} R^2 \frac{h_\nu^2}{h_R^2} \right] = \\ &= -2R^{-3} R^2 \frac{h_\nu^2}{h_R^2} + R^{-2} \frac{\partial}{\partial R} \left[ R^2 \frac{R^2}{1+\mu} W^{-2} W^{-\frac{2}{1+\mu}} \left( \frac{\partial W}{\partial \nu} \right)^2 \sum_{k=0}^{\infty} \frac{-\frac{2+\mu}{1+\mu}}{-\frac{2+\mu}{1+\mu} + \frac{\mu}{1+\mu} k} \binom{-\frac{2+\mu}{1+\mu} + \frac{\mu}{1+\mu} k}{k} \left( W^{-\frac{2}{1+\mu}} \right)^k \right] = -\frac{2}{R} \frac{h_\nu^2}{h_R^2} + \\ &= \frac{1}{R^2} \left[ \frac{R^3}{1+\mu} W^{-2} W^{-\frac{2}{1+\mu}} \left( \frac{\partial W}{\partial \nu} \right)^2 \sum_{k=0}^{\infty} \frac{-\frac{2+\mu}{1+\mu}}{-\frac{2+\mu}{1+\mu} + \frac{\mu}{1+\mu} k} \binom{-\frac{2+\mu}{1+\mu} + \frac{\mu}{1+\mu} k}{k} \left( -\frac{2\mu(k+1)}{1+\mu} - 2\mu + 4 + 2\mu \right) \left( W^{-\frac{2}{1+\mu}} \right)^k \right] = \end{aligned}$$

$$\begin{aligned}
& -\frac{2}{R} \frac{h_v^2}{h_R^2} + \frac{1}{R^2} \left[ \frac{R^3}{1+\mu} W^{-2} W^{-\frac{2}{1+\mu}} \left( \frac{\partial W}{\partial v} \right)^2 \sum_{k=0}^{\infty} 2_{1+\mu}^{2+\mu} \binom{-\frac{2+\mu}{1+\mu} + \frac{\mu}{1+\mu} k}{k} \left( W^{-\frac{2}{1+\mu}} \right)^k \right] = \\
& -\frac{2}{R} \frac{h_v^2}{h_R^2} + 2 \frac{2+\mu}{R} \frac{R^2}{(1+\mu)^2} W^{-2} \frac{2+\mu}{1+\mu} \left( \frac{\partial W}{\partial v} \right)^2 \sum_{k=0}^{\infty} \binom{-\frac{2+\mu}{1+\mu} + \frac{\mu}{1+\mu} k}{k} \left( W^{-\frac{2}{1+\mu}} \right)^k = -\frac{2}{R} \frac{h_v^2}{h_R^2} + 2 \frac{2+\mu}{R} h_v^2 = \frac{2h_v^2}{R} \left( \mu + 2 - \frac{1}{h_R^2} \right)
\end{aligned} \quad (F37)$$

which is equivalent to the small- $v$  region form. The final relation we need is Eq. (86) which tells that

$$h_R^2 = \left[ 1 - \mu \sum_{k=0}^{\infty} \binom{\frac{\mu}{1+\mu} k - 1}{k} \frac{\left( W^{-\frac{2}{1+\mu}} \right)^k}{\frac{\mu}{1+\mu} k - 1} \right]^{-1} = \frac{1}{g} \quad \text{where} \quad g = \frac{1}{h_R^2} = \left[ 1 - \mu \sum_{k=0}^{\infty} \binom{\frac{\mu}{1+\mu} k - 1}{k} \frac{\left( W^{-\frac{2}{1+\mu}} \right)^k}{\frac{\mu}{1+\mu} k - 1} \right] \quad (F38)$$

and thus

$$\begin{aligned}
\frac{\partial h_R^2}{\partial R} &= \frac{\partial}{\partial R} \left( \frac{1}{g} \right) = -\frac{1}{g^2} \frac{\partial g}{\partial R} = -\frac{1}{\frac{1}{h_R^4}} \frac{\partial}{\partial R} \left[ 1 - \mu \sum_{k=0}^{\infty} \binom{\frac{\mu}{1+\mu} k - 1}{k} \frac{\left( W^{-\frac{2}{1+\mu}} \right)^k}{\frac{\mu}{1+\mu} k - 1} \right] = \\
& -h_R^4 \left[ -\mu \sum_{k=0}^{\infty} \binom{\frac{\mu}{1+\mu} k - 1}{k} \frac{-\frac{2\mu k}{1+\mu}}{\frac{\mu}{1+\mu} k - 1} \frac{1}{R} \left( W^{-\frac{2}{1+\mu}} \right)^k \right] = -\frac{h_R^4}{R} \frac{2\mu^2}{1+\mu} \left[ 0 + \sum_{k=1}^{\infty} \binom{\frac{\mu}{1+\mu} k - 1}{k} \frac{k}{\frac{\mu}{1+\mu} k - 1} \left( W^{-\frac{2}{1+\mu}} \right)^k \right]
\end{aligned} \quad (F39)$$

After the use of (A4) identity from **Supplement A**, re-indexing, and subsequently applying the identity (A3), we arrive at

$$\begin{aligned}
\frac{\partial h_R^2}{\partial R} &= -\frac{h_R^4}{R} \frac{2\mu^2}{1+\mu} \left[ \sum_{k=1}^{\infty} \binom{\frac{\mu}{1+\mu} k - 1}{k-1} \frac{\frac{\mu}{1+\mu} k - 1 - k + 1}{k} \frac{k}{\frac{\mu}{1+\mu} k - 1} \left( W^{-\frac{2}{1+\mu}} \right)^k \right] = \\
& -\frac{h_R^4}{R} \frac{2\mu^2}{1+\mu} \left[ \sum_{k=1}^{\infty} \binom{\frac{\mu}{1+\mu} k - 1}{k-1} \frac{\frac{\mu}{1+\mu} k - k}{\frac{\mu}{1+\mu} k - 1} \left( W^{-\frac{2}{1+\mu}} \right)^k \right] = \\
& -\frac{h_R^4}{R} \frac{2\mu^2}{1+\mu} \left[ \sum_{M=0}^{\infty} \binom{\frac{\mu}{1+\mu} (M+1) - 1}{M} \frac{\left( \frac{\mu}{1+\mu} - 1 \right) (M+1)}{\frac{\mu}{1+\mu} (M+1) - 1} \left( W^{-\frac{2}{1+\mu}} \right)^{M+1} \right] = \\
& -\frac{h_R^4}{R} \frac{2\mu^2}{1+\mu} W^{-\frac{2}{1+\mu}} \left[ \sum_{M=0}^{\infty} \binom{\frac{\mu}{1+\mu} M - \frac{2+\mu}{1+\mu}}{M} \frac{\left( \frac{\mu}{1+\mu} - 1 \right) (M+1)}{-\frac{1}{1+\mu} M - \frac{1}{1+\mu}} \left( W^{-\frac{2}{1+\mu}} \right)^M \right] = \\
& -\frac{h_R^4}{R} \frac{2\mu^2}{1+\mu} W^{-\frac{2}{1+\mu}} \left[ \sum_{M=0}^{\infty} \binom{\frac{\mu}{1+\mu} M - \frac{2+\mu}{1+\mu}}{M} \left( W^{-\frac{2}{1+\mu}} \right)^M \right] = -\frac{h_R^4}{R} \frac{2\mu^2}{1+\mu} W^{-\frac{2}{1+\mu}} \frac{h_v^2}{\frac{R^2}{(1+\mu)^2} W^{-2} \frac{2+\mu}{1+\mu} \left( \frac{\partial W}{\partial v} \right)^2} = \\
& -\frac{2(1+\mu)\mu^2}{R^3} h_R^4 h_v^2 \frac{W^2}{\left( \frac{\partial W}{\partial v} \right)^2} . \quad (F40)
\end{aligned}$$

Now, we have all the relations (see (F37) and (F40)) needed to finalize the relation using (F15):

$$\begin{aligned}
\frac{\partial h_v^2}{\partial R} &= h_R^2 \frac{\partial (h_v^2/h_R^2)}{\partial R} + \frac{h_v^2}{h_R^2} \frac{\partial h_R^2}{\partial R} = h_R^2 \frac{2h_v^2}{R} \left( \mu + 2 - \frac{1}{h_R^2} \right) - \frac{h_v^2}{h_R^2} \frac{2(1+\mu)\mu^2}{R^3} h_R^4 h_v^2 \frac{W^2}{\left( \frac{\partial W}{\partial v} \right)^2} = h_R^2 \frac{2h_v^2}{R} \left( \mu + 2 - \frac{1}{h_R^2} \right) - \\
& \frac{2(1+\mu)\mu^2}{R^3} h_R^2 h_v^4 \frac{W^2}{\left( \frac{\partial W}{\partial v} \right)^2} = \frac{2}{R} h_R^2 h_v^2 \left( \mu + 2 - \frac{1}{h_R^2} \right) - \frac{2(1+\mu)\mu^2}{R^3} h_R^2 h_v^4 \left( \frac{\sin v \cos v}{1+\mu \sin^2 v} \right)^2 . \quad (F41)
\end{aligned}$$

Therefore,

$$\frac{1}{h_R h_v} \frac{\partial h_v}{\partial R} = \frac{h_R}{2h_R^2 h_v^2} \frac{\partial h_v^2}{\partial R} = \frac{1}{R} \left[ (\mu + 2) h_R - \frac{1}{h_R} - \frac{(1+\mu)\mu^2}{R^2} \left( \frac{\sin v \cos v}{1+\mu \sin^2 v} \right)^2 h_R h_v^2 \right] , \quad (F42)$$

the form identical to the one in the small- $v$  region.

### Large- $\nu$ region, term containing $\partial h_R / \partial \nu$

When we again use Eq. (86), we arrive - for the derivative of the squared  $h_R$  with respect to  $\nu$  - to

$$\begin{aligned} \frac{\partial h_R^2}{\partial \nu} &= \frac{\partial}{\partial \nu} \left( \frac{1}{g} \right) = -\frac{1}{g^2} \frac{\partial g}{\partial \nu} = -\frac{1}{h_R^4} \frac{\partial}{\partial \nu} \left[ 1 - \mu \sum_{k=0}^{\infty} \binom{\frac{\mu}{1+\mu}k-1}{k} \frac{\left( W^{-\frac{2}{1+\mu}} \right)^k}{\frac{\mu}{1+\mu}k-1} \right] = \\ &= -h_R^4 \left[ -\mu \sum_{k=0}^{\infty} \binom{\frac{\mu}{1+\mu}k-1}{k} \frac{-\frac{2k}{1+\mu}}{\frac{\mu}{1+\mu}k-1} \left( W^{-\frac{2}{1+\mu}} \right)^k \frac{1}{W} \frac{\partial W}{\partial \nu} \right] = \\ &= -2\mu h_R^4 \frac{1}{W} \frac{\partial W}{\partial \nu} \left[ 0 + \sum_{k=1}^{\infty} \binom{\frac{\mu}{1+\mu}k-1}{k} \frac{\frac{k}{1+\mu}}{\frac{\mu}{1+\mu}k-1} \left( W^{-\frac{2}{1+\mu}} \right)^k \right]. \quad (\text{F43}) \end{aligned}$$

After the use of (A4) identity from **Supplement A**, and subsequently the identity (A3) in a similar way as for (F40), we arrive at

$$\begin{aligned} \frac{\partial h_R^2}{\partial \nu} &= -2\mu h_R^4 \frac{1}{W} \frac{\partial W}{\partial \nu} \left[ 0 + \sum_{k=1}^{\infty} \binom{\frac{\mu}{1+\mu}k-1}{k} \frac{\frac{k}{1+\mu}}{\frac{\mu}{1+\mu}k-1} \left( W^{-\frac{2}{1+\mu}} \right)^k \right] = \\ &= -2\mu h_R^4 \frac{1}{W} \frac{\partial W}{\partial \nu} \left[ \sum_{k=1}^{\infty} \binom{\frac{\mu}{1+\mu}k-1}{k-1} \frac{\frac{\mu}{1+\mu}k-1-k+1}{k} \frac{\frac{k}{1+\mu}}{\frac{\mu}{1+\mu}k-1} \left( W^{-\frac{2}{1+\mu}} \right)^k \right] = \\ &= -2 \frac{\mu}{1+\mu} h_R^4 \frac{1}{W} \frac{\partial W}{\partial \nu} \left[ \sum_{k=1}^{\infty} \binom{\frac{\mu}{1+\mu}k-1}{k-1} \frac{\frac{\mu}{1+\mu}k-k}{\frac{\mu}{1+\mu}k-1} \left( W^{-\frac{2}{1+\mu}} \right)^k \right] = \\ &= -2 \frac{\mu}{1+\mu} h_R^4 \frac{1}{W} \frac{\partial W}{\partial \nu} \left[ \sum_{M=0}^{\infty} \binom{\frac{\mu}{1+\mu}(M+1)-1}{M} \frac{\left( \frac{\mu}{1+\mu}-1 \right)(M+1)}{\frac{\mu}{1+\mu}(M+1)-1} \left( W^{-\frac{2}{1+\mu}} \right)^{M+1} \right] = \\ &= -2 \frac{\mu}{1+\mu} h_R^4 \frac{1}{W} W^{-\frac{2}{1+\mu}} \frac{\partial W}{\partial \nu} \left[ \sum_{M=0}^{\infty} \binom{\frac{\mu}{1+\mu}M-\frac{2+\mu}{1+\mu}}{M} \frac{\left( \frac{\mu}{1+\mu}-1 \right)(M+1)}{-\frac{1}{1+\mu}M-\frac{1}{1+\mu}} \left( W^{-\frac{2}{1+\mu}} \right)^M \right] = \\ &= -2 \frac{\mu}{1+\mu} h_R^4 W^{-\frac{2}{1+\mu}-1} \frac{\partial W}{\partial \nu} \left[ \sum_{M=0}^{\infty} \binom{\frac{\mu}{1+\mu}M-\frac{2+\mu}{1+\mu}}{M} \left( W^{-\frac{2}{1+\mu}} \right)^M \right] = -2 \frac{\mu}{1+\mu} h_R^4 W^{-\frac{\mu+3}{1+\mu}} \frac{\partial W}{\partial \nu} \frac{h_v^2}{\frac{R^2}{(1+\mu)^2} W^{-2\frac{2+\mu}{1+\mu}} \left( \frac{\partial W}{\partial \nu} \right)^2} = \\ &= -2 \frac{(1+\mu)\mu}{R^2} h_R^4 W^{-\frac{\mu+3}{1+\mu}+2\frac{2+\mu}{1+\mu}} \frac{h_v^2}{\frac{\partial W}{\partial \nu}} = -2 \frac{(1+\mu)\mu}{R^2} h_R^4 W^{-\frac{-\mu-3+4+2\mu}{1+\mu}} \frac{h_v^2}{\frac{\partial W}{\partial \nu}} = -2 \frac{(1+\mu)\mu}{R^2} h_R^4 h_v^2 \frac{W}{\frac{\partial W}{\partial \nu}}. \quad (\text{F44}) \end{aligned}$$

Thus

$$\frac{1}{h_R h_v} \frac{\partial h_R}{\partial \nu} = \frac{1}{2h_R^2 h_v} \frac{\partial h_R^2}{\partial \nu} = -\frac{\mu(1+\mu)}{R^2} \frac{W}{\frac{\partial W}{\partial \nu}} h_R^2 h_v, \quad (\text{F45})$$

which is the form identical to the one in the small- $\nu$  region.

### Small- and large- $\nu$ regions, overview

The obtained relations for coefficients containing derivatives of the metric scale factors in both the small- and the large- $\nu$  region are listed here:

$$\frac{1}{h_R h_\lambda} \frac{\partial h_\lambda}{\partial R} = \frac{h_R}{R} \quad (\text{F46a})$$

$$\frac{1}{h_\nu h_\lambda} \frac{\partial h_\lambda}{\partial \nu} = -\sqrt{\frac{1}{h_\lambda^2} - \frac{h_R^2}{R^2}} \quad (\text{F46b})$$

$$\frac{1}{h_R h_\nu} \frac{\partial h_\nu}{\partial R} = \frac{1}{R} \left[ (\mu + 2) h_R - \frac{1}{h_R} - \frac{(1+\mu)\mu^2}{R^2} \left( \frac{\sin \nu \cos \nu}{1+\mu \sin^2 \nu} \right)^2 h_R h_\nu^2 \right] \quad (\text{F46c})$$

$$\frac{1}{h_R h_\nu} \frac{\partial h_R}{\partial \nu} = -\frac{\mu(1+\mu)}{R^2} \frac{\sin \nu \cos \nu}{1+\mu \sin^2 \nu} h_R^2 h_\nu \quad (\text{F46d})$$
