# Supplementary material for: Analytical Solution of Similar Oblate Spheroidal Coordinate System
Source: arXiv:2109.12057 ancillary file (2021-09-06)
Supplement: Supplementary file 6 [file Supplement_SOS_G.pdf]

# Analytical solution of Similar Oblate Spheroidal Coordinate System

---

Pavel Strunz

Nuclear Physics Institute of the CAS, Řež, Czech Republic

e-mail: strunz@ujf.cas.cz

## Supplement G

### Transformation between two families of SOS coordinates

In certain cases, transformation between two different (but concentric) SOS coordinates - denoted  $(R, \nu, \lambda)$  and  $(R_F, \nu_F, \lambda_F)$  in what follows - can be of advantage. For illustration, we derive the transformation relations for the small- $\nu$  region.

Their parameters determining eccentricity (see (2)) are  $\mu$  and  $\mu_F$ . Each of these two SOS coordinate systems contains the same family of half-planes for constant  $\lambda$  and  $\lambda_F$  (therefore,  $\lambda_F = \lambda$ ), but different family of oblate spheroid surfaces for constant  $R$  or  $R_F$ , and also different family of surfaces for constant  $\nu$  or  $\nu_F$ . Nevertheless, every point in space is unambiguously determined by both  $(R, \nu, \lambda)$  and  $(R_F, \nu_F, \lambda_F)$  coordinates. Transformation between them can be done through the Cartesian coordinates, as (see equations (1), (3), (5))

$$x^2 + y^2 + (1 + \mu) z^2 = R^2, \quad z = \frac{1}{(1 + \mu)^{1/2} R_0^\mu} \frac{\sin \nu}{\cos^{1+\mu} \nu} x^{1+\mu} \quad (G1a)$$

and, at the same time, the Cartesian coordinates can be expressed using the second family of SOS coordinates  $(R_F, \nu_F, \lambda_F)$

$$x^2 + y^2 + (1 + \mu_F) z^2 = R_F^2, \quad z = \frac{1}{(1 + \mu_F)^{1/2} R_0^{\mu_F}} \frac{\sin \nu_F}{\cos^{1+\mu_F} \nu_F} x^{1+\mu_F} \quad (G1b)$$

Note, that the parameter  $R_0$  (the equatorial radius of the reference oblate spheroid surface) is held the same for both SOS coordinate systems.

It comes out from the left-hand side relations in (G1a), (G1b) that

$$\frac{R^2 - R_F^2}{\mu - \mu_F} = z^2 \quad (G2)$$

$z$  can be expressed also in the form of sum, see (52), and then

$$R_F^2 = R^2 - (\mu - \mu_F) z^2 = R^2 - (\mu - \mu_F) W^2 (1 + \mu) \frac{R^2}{4} \left[ \sum_{k=0}^{\infty} \left( -\frac{1+\mu}{2} - \mu k \right) \frac{-(W^2)^k}{-\frac{1+\mu}{2} - \mu k} \right]^2 \quad (G3)$$

where we restricted the solution to the small- $\nu$  region only. In this way, the coordinate  $R_F$  of the second set of SOS coordinates  $(R_F, \nu_F, \lambda_F)$  is expressed explicitly in terms of  $(R, \nu, \lambda)$  SOS coordinate system.

Further simplification of the squared sum in the formula can be carried out using Cauchy product, Hagen-Rothe identity (Chu 2010, Chu 2013) and binomial identity (A4):

$$\begin{aligned}
& \left[ \sum_{k=0}^{\infty} \binom{-\frac{1+\mu}{2}-\mu k}{k} \frac{-(W^2)^k}{-\frac{1+\mu}{2}-\mu k} \right]^2 \\
&= \sum_{k=0}^{\infty} (W^2)^k \sum_{m=0}^k \binom{-\frac{1+\mu}{2}-\mu m}{m} \frac{-1}{-\frac{1+\mu}{2}-\mu m} \binom{-\frac{1+\mu}{2}-\mu(k-m)}{k-m} \frac{-1}{-\frac{1+\mu}{2}-\mu(k-m)} \\
&= \sum_{k=0}^{\infty} (W^2)^k \frac{1}{-\frac{1+\mu}{2}} \frac{1}{-\frac{1+\mu}{2}} \frac{-1-\mu}{-1-\mu-\mu k} \binom{-1-\mu-\mu k}{k} \\
&= \sum_{k=0}^{\infty} (W^2)^k \frac{-4}{1+\mu} \frac{1}{-\mu(k+1)-1} \binom{-\mu(k+1)-1}{k} \\
&= \sum_{M=1}^{\infty} (W^2)^{M-1} \frac{-4}{1+\mu} \frac{1}{-\mu M-1} \binom{-\mu M-1}{M-1} \\
&= \sum_{M=1}^{\infty} (W^2)^{M-1} \frac{-4}{1+\mu} \frac{1}{-\mu M-1} \binom{-\mu M-1}{M} \frac{M}{-\mu M-1-M+1} \\
&= \frac{4}{W^2(1+\mu)^2} \sum_{M=1}^{\infty} \frac{1}{-\mu M-1} \binom{-\mu M-1}{M} (W^2)^M \\
&= \frac{4}{W^2(1+\mu)^2} \left[ 1 + \sum_{M=0}^{\infty} \frac{1}{-\mu M-1} \binom{-\mu M-1}{M} (W^2)^M \right]
\end{aligned} \tag{G4}$$

Then, according to (G3),  $R_F$  is equal to

$$\begin{aligned}
R_F &= \sqrt{R^2 - R^2 \frac{\mu - \mu_F}{1 + \mu} \left[ 1 + \sum_{M=0}^{\infty} \frac{1}{-\mu M - 1} \binom{-\mu M - 1}{M} (W^2)^M \right]} \\
&= R \sqrt{\left[ \frac{1 + \mu_F}{1 + \mu} + \frac{\mu_F - \mu}{1 + \mu} \sum_{M=0}^{\infty} \frac{1}{-\mu M - 1} \binom{-\mu M - 1}{M} (W^2)^M \right]}
\end{aligned} \tag{G5}$$

In this way, we obtained  $R_F$  coordinate of the second SOS system expressed in terms containing only  $R$  and  $v$ .

For further use, we also substitute  $R_F$  from (G5) to (G2) and – after algebraic manipulations – obtain:

$$z^2 = \frac{R^2 - R_F^2}{\mu - \mu_F} = \frac{R^2}{1 + \mu} \left( 1 + \sum_{M=0}^{\infty} \frac{1}{-\mu M - 1} \binom{-\mu M - 1}{M} (W^2)^M \right) \tag{G6}$$

Now, we derive the transformation for  $v_F$  coordinate. It comes out from the ratio of the right-hand side relations in (G1a), (G1b) that

$$\frac{\frac{1}{z^{1+\mu}}}{\frac{1}{z^{1+\mu_F}}} = \frac{1}{z^{1+\mu}} - \frac{1}{1+\mu_F} = \frac{\mu_F - \mu}{z^{(1+\mu)(1+\mu_F)}} = \frac{\left( \frac{1}{(1+\mu)^{1/2} R_0^\mu} \frac{\sin v}{\cos^{1+\mu} v} \right)^{\frac{1}{1+\mu}} x}{\left( \frac{1}{(1+\mu_F)^{1/2} R_0^{\mu_F}} \frac{\sin v_F}{\cos^{1+\mu_F} v_F} \right)^{\frac{1}{1+\mu_F}} x} = \frac{R_0^{\frac{\mu_F}{1+\mu_F}} (\sqrt{1+\mu_F})^{\frac{1}{1+\mu_F}} \left( \frac{\sin v}{\cos^{1+\mu} v} \right)^{\frac{1}{1+\mu}}}{R_0^{\frac{\mu}{1+\mu}} (\sqrt{1+\mu})^{\frac{1}{1+\mu}} \left( \frac{\sin v_F}{\cos^{1+\mu_F} v_F} \right)^{\frac{1}{1+\mu_F}}} \tag{G7}$$

and then

$$z = \frac{R_0^{\frac{\mu_F(1+\mu)}{\mu_F-\mu}} (\sqrt{1+\mu_F})^{\frac{1+\mu}{\mu_F-\mu}} \left( \frac{\sin v}{\cos^{1+\mu} v} \right)^{\frac{1+\mu_F}{\mu_F-\mu}}}{R_0^{\frac{\mu(1+\mu_F)}{\mu_F-\mu}} (\sqrt{1+\mu})^{\frac{1+\mu_F}{\mu_F-\mu}} \left( \frac{\sin v_F}{\cos^{1+\mu_F} v_F} \right)^{\frac{1+\mu}{\mu_F-\mu}}} = R_0 \frac{(\sqrt{1+\mu_F})^{\frac{1+\mu}{\mu_F-\mu}} \left( \frac{\sin v}{\cos^{1+\mu} v} \right)^{\frac{1+\mu_F}{\mu_F-\mu}}}{(\sqrt{1+\mu})^{\frac{1+\mu_F}{\mu_F-\mu}} \left( \frac{\sin v_F}{\cos^{1+\mu_F} v_F} \right)^{\frac{1+\mu}{\mu_F-\mu}}} \quad (G8)$$

We can then separate the terms with  $v_F$  coordinate on the left side and use (G2) for expression of  $z$ . This leads to

$$\left( \frac{\sin v_F}{\cos^{1+\mu_F} v_F} \right)^{\frac{1+\mu}{\mu_F-\mu}} = \frac{R_0}{\sqrt{\frac{R^2 - R_F^2}{\mu - \mu_F}}} \frac{(\sqrt{1+\mu_F})^{\frac{1+\mu}{\mu_F-\mu}} \left( \frac{\sin v}{\cos^{1+\mu} v} \right)^{\frac{1+\mu_F}{\mu_F-\mu}}}{(\sqrt{1+\mu})^{\frac{1+\mu_F}{\mu_F-\mu}}} \quad (G9)$$

As  $R_F$  is determined (see (G5)), the transformation from  $(R, v, \lambda)$  to  $(R_F, v_F, \lambda_F)$  can be performed.

Nevertheless, in order to obtain  $v_F$  containing terms expressed in terms containing only  $R$  and  $v$ , we can also substitute the  $R_F$ -containing term from (G6), receiving thus

$$\begin{aligned} \frac{\sin v_F}{\cos^{1+\mu_F} v_F} &= \left( \frac{R_0}{\sqrt{\frac{R^2 - R_F^2}{\mu - \mu_F}}} \right)^{\frac{\mu_F-\mu}{1+\mu}} \frac{(\sqrt{1+\mu_F})^{\frac{1+\mu}{\mu_F-\mu}} \left( \frac{\sin v}{\cos^{1+\mu} v} \right)^{\frac{1+\mu_F}{\mu_F-\mu}}}{(\sqrt{1+\mu})^{\frac{1+\mu_F}{\mu_F-\mu}}} \\ &= \sqrt{\frac{1+\mu_F}{1+\mu}} \left( \frac{R_0}{R \sqrt{1 + \sum_{M=0}^{\infty} \frac{1}{-\mu M - 1} \binom{-\mu M - 1}{M} (W^2)^M}} \right)^{\frac{\mu_F-\mu}{1+\mu}} \left( \frac{\sin v}{\cos^{1+\mu} v} \right)^{\frac{1+\mu_F}{1+\mu}} = \end{aligned} \quad (G10)$$

In this way, we obtained  $v_F$  containing terms expressed in terms containing only  $R$  and  $v$ . For a full separation of  $v_F$ , procedure similar to the one described by equations (57)-(60) would be needed.

It should be also noted, that the abovementioned derivation is restricted to the small- $v$  region.
