# Supplementary material for: Analytical Solution of Similar Oblate Spheroidal Coordinate System
Source: arXiv:2109.12057 ancillary file (2021-09-06)
Supplement: Supplementary file 7 [file Supplement_SOS_B.pdf]

# Analytical solution of Similar Oblate Spheroidal Coordinate System

---

Pavel Strunz

Nuclear Physics Institute of the CAS, Řež, Czech Republic

e-mail: strunz@ujf.cas.cz

## Supplement B

### Partial derivatives with respect to $v$ in the small- $v$ region

Here, partial derivatives with respect to  $v$  are determined. First, let's determine the partial derivative of the coordinate  $x$  with respect to  $v$  in the **small  $v$  region**. In order to use Jensen ([Gould 1972](#)) and Hagen-Rothe ([Chu 2010, Chu 2013](#)) identities later, the 3<sup>rd</sup> form (A6c) of the coordinate  $x$  is used for the derivative determination. The dependence (22) of  $W$  on  $v$  has to be considered. Then

$$\begin{aligned}
 \frac{\partial x(v, R)}{\partial v} &= \frac{\partial}{\partial v} \left\{ \frac{R}{2} \sum_{k=0}^{\infty} \binom{-\frac{1}{2} - \mu k}{k} \frac{(W^2)^k}{-\frac{1}{2} - \mu k} \right\} = \frac{\partial}{\partial v} \left\{ W^{-\frac{1}{\mu}} \frac{R}{2} \sum_{k=0}^{\infty} \binom{-\frac{1}{2} - \mu k}{k} \frac{(W^{\frac{1}{\mu}})^{2\mu k + 1}}{\frac{1}{2} + \mu k} \right\} = \\
 &= \frac{R}{2} \left\{ \left[ \frac{\partial}{\partial v} (W^{-\frac{1}{\mu}}) \sum_{k=0}^{\infty} \binom{-\frac{1}{2} - \mu k}{k} \frac{(W^{\frac{1}{\mu}})^{2\mu k + 1}}{\frac{1}{2} + \mu k} \right] \right. \\
 &\quad \left. + \left[ W^{-\frac{1}{\mu}} \sum_{k=0}^{\infty} \binom{-\frac{1}{2} - \mu k}{k} \frac{\frac{\partial}{\partial v} ((W^{\frac{1}{\mu}})^{2\mu k + 1})}{\frac{1}{2} + \mu k} \right] \right\} \\
 &= \frac{R}{2} \left\{ (W^{\frac{1}{\mu}}) \frac{\partial}{\partial v} (W^{-\frac{1}{\mu}}) \sum_{k=0}^{\infty} \binom{-\frac{1}{2} - \mu k}{k} \frac{(W^{\frac{1}{\mu}})^{2\mu k}}{\frac{1}{2} + \mu k} \right. \\
 &\quad \left. + W^{-\frac{1}{\mu}} \frac{\partial}{\partial v} (W^{\frac{1}{\mu}}) \sum_{k=0}^{\infty} \binom{-\frac{1}{2} - \mu k}{k} \frac{(2\mu k + 1) (W^{\frac{1}{\mu}})^{2\mu k}}{\frac{1}{2} + \mu k} \right\} = \\
 &= \frac{R}{2} \frac{1}{\mu W} \frac{\partial W}{\partial v} \left\{ \sum_{k=0}^{\infty} \binom{-\frac{1}{2} - \mu k}{k} \frac{(W^2)^k}{-\frac{1}{2} - \mu k} + 2 \sum_{k=0}^{\infty} \binom{-\frac{1}{2} - \mu k}{k} (W^2)^k \right\}
 \end{aligned} \tag{B1}$$

where (see Eq. (22))

$$W = \left(\frac{R}{R_0}\right)^\mu \frac{\sin v}{\cos^{1+\mu} v} \quad \text{and} \quad \frac{\partial W}{\partial v} = \left(\frac{R}{R_0}\right)^\mu \frac{\partial}{\partial v} \frac{\sin v}{\cos^{1+\mu} v} =$$

$$= \left(\frac{R}{R_0}\right)^\mu \frac{1 + \mu \sin^2 v}{\cos^{2+\mu} v} \quad \text{and} \quad \frac{1}{W} \frac{\partial W}{\partial v} = \frac{1 + \mu \sin^2 v}{\sin v \cos v}$$
(B2)

The terms in the sums in (B1) with the same binomial coefficients can be put together and then the derivative reads

$$\frac{\partial x(v, R)}{\partial v} = R \frac{1}{W} \frac{\partial W}{\partial v} \sum_{k=1}^{\infty} \binom{-\frac{1}{2} - \mu k}{k} \frac{2k}{2\mu k + 1} (W^2)^k = R \frac{\partial W}{\partial v} \sum_{k=1}^{\infty} \binom{-\frac{1}{2} - \mu k}{k} \frac{2k}{2\mu k + 1} (W^2)^{k-\frac{1}{2}}$$
(B3)

This formula works also for  $\mu=0$ , and the last one also shows that there is no issue for  $v=0$ , for which  $\sin v$  is equal to zero and  $1/W$  thus tends to infinity.

For the metric factor calculation, which is to be carried out later, also the square of the derivative is needed. For further simplification, the (B1) expression of the derivative is best suited to proceed:

$$\left(\frac{\partial x(v, R)}{\partial v}\right)^2 = \left(\frac{R}{2}\right)^2 \frac{1}{\mu^2 W^2} \left(\frac{\partial W}{\partial v}\right)^2 \left\{ \sum_{k=0}^{\infty} \binom{-\frac{1}{2} - \mu k}{k} \frac{(W^2)^k}{-\frac{1}{2} - \mu k} + 2 \sum_{k=0}^{\infty} \binom{-\frac{1}{2} - \mu k}{k} (W^2)^k \right\}^2 =$$

$$= \left(\frac{R}{2}\right)^2 \frac{1}{\mu^2 W^2} \left(\frac{\partial W}{\partial v}\right)^2 \left\{ \left[ \sum_{k=0}^{\infty} \binom{-\frac{1}{2} - \mu k}{k} \frac{(W^2)^k}{-\frac{1}{2} - \mu k} \right]^2 \right.$$

$$+ 2 \left[ \sum_{k=0}^{\infty} \binom{-\frac{1}{2} - \mu k}{k} \frac{(W^2)^k}{-\frac{1}{2} - \mu k} \right] \left[ 2 \sum_{k=0}^{\infty} \binom{-\frac{1}{2} - \mu k}{k} (W^2)^k \right]$$

$$\left. + \left[ 2 \sum_{k=0}^{\infty} \binom{-\frac{1}{2} + (\mu + 1)k}{k} (-W^2)^k \right]^2 \right\}$$
(B4)

where the binomial identity (A3) was used in the third term.

The Cauchy products are then used for the three terms:

$$\left(\frac{\partial x(v, R)}{\partial v}\right)^2 =$$

$$= \left(\frac{R}{2}\right)^2 \frac{1}{\mu^2 W^2} \left(\frac{\partial W}{\partial v}\right)^2 \left\{ \left[ \sum_{k=0}^{\infty} (W^2)^k \sum_{m=0}^k \frac{1}{-\frac{1}{2} - \mu m} \binom{-\frac{1}{2} - \mu m}{m} \frac{1}{-\frac{1}{2} - \mu(k-m)} \binom{-\frac{1}{2} - \mu(k-m)}{k-m} \right] \right.$$

$$+ 4 \left[ \sum_{k=0}^{\infty} (W^2)^k \sum_{m=0}^k \binom{-\frac{1}{2} - \mu m}{m} \frac{1}{-\frac{1}{2} - \mu m} \binom{-\frac{1}{2} - \mu(k-m)}{k-m} \right]$$

$$\left. + 4 \left[ \sum_{k=0}^{\infty} (-W^2)^k \sum_{m=0}^k \binom{-\frac{1}{2} + (\mu + 1)m}{m} \binom{-\frac{1}{2} + (\mu + 1)(k-m)}{k-m} \right] \right\}$$
(B5)

This operation is followed by the use of Hagen-Rothe (Chu 2010, Chu 2013) and Jensen (Gould 1972) identities in order to simplify the squared derivative:

$$\begin{aligned}
\left(\frac{\partial x(v, R)}{\partial v}\right)^2 &= \left(\frac{R}{2}\right)^2 \frac{1}{\mu^2 W^2} \left(\frac{\partial W}{\partial v}\right)^2 \left\{ -4 \sum_{k=0}^{\infty} \frac{1}{-1-\mu k} \binom{-1-\mu k}{k} (W^2)^k - 8 \sum_{k=0}^{\infty} \binom{-1-\mu k}{k} (W^2)^k \right. \\
&\quad \left. + 4 \sum_{k=0}^{\infty} \left[ -(-1)^{k-1} (W^2)^k \sum_{m=0}^k \binom{\mu k - 1 + (k-m)}{k-m} (1+\mu)^m \right] \right\} = \\
&= \left(\frac{R}{2}\right)^2 \frac{1}{\mu^2} \left(\frac{\partial W}{\partial v}\right)^2 \left\{ -4 \sum_{k=0}^{\infty} \frac{1}{-\mu k - 1} \binom{-\mu k - 1}{k} (W^2)^{k-1} - 8 \sum_{k=0}^{\infty} \binom{-\mu k - 1}{k} (W^2)^{k-1} \right. \\
&\quad \left. - 4 \sum_{k=0}^{\infty} \left[ (-W^2)^{k-1} \sum_{m=0}^k \binom{\mu k - 1 + m}{m} (1+\mu)^{k-m} \right] \right\}
\end{aligned} \tag{B6}$$

For later use and with the help of binomial identity  $\binom{\alpha-1}{k} = \binom{\alpha}{k} \frac{\alpha-k}{\alpha}$  (which can be, however, used only when  $\alpha \neq 0$ , and some terms with  $k=0$  thus has to be treated separately), it is of advantage to rewrite the expression to the form

$$\begin{aligned}
\left(\frac{\partial x(v, R)}{\partial v}\right)^2 &= \left(\frac{R}{2}\right)^2 \frac{1}{\mu^2} \left(\frac{\partial W}{\partial v}\right)^2 \left\{ -4 \sum_{k=1}^{\infty} \frac{1}{-\mu k - 1} \binom{-\mu k - 1}{k} (W^2)^{k-1} + \frac{4}{W^2} \right. \\
&\quad \left. - 8 \sum_{k=1}^{\infty} \binom{-\mu k - 1}{k} (W^2)^{k-1} - \frac{8}{W^2} \right. \\
&\quad \left. - 4 \sum_{k=0}^{\infty} \left[ (-W^2)^{k-1} \sum_{m=0}^k \binom{\mu k - 1 + m}{m} (1+\mu)^{k-m} \right] \right\} = \\
&= \left(\frac{R}{2}\right)^2 \frac{1}{\mu^2} \left(\frac{\partial W}{\partial v}\right)^2 \left\{ -4 \frac{\mu+1}{\mu} \sum_{k=1}^{\infty} \frac{1}{-\mu k - 1} \binom{-\mu k}{k} (W^2)^{k-1} + \frac{4}{W^2} \right. \\
&\quad \left. - 8 \frac{\mu+1}{\mu} \sum_{k=1}^{\infty} \binom{-\mu k}{k} (W^2)^{k-1} - \frac{8}{W^2} \right. \\
&\quad \left. - 4 \sum_{k=0}^{\infty} \left[ (-W^2)^{k-1} \sum_{m=0}^k \binom{\mu k - 1 + m}{m} (1+\mu)^{k-m} \right] \right\}
\end{aligned} \tag{B7}$$

where reverse counting was used in the inner sum of the third term.

Similarly, the partial derivative of  $z$  with respect to  $v$  in the **small- $v$  region** is obtained using Eq. (A5c)

$$\begin{aligned}
\frac{\partial z(\nu, R)}{\partial \nu} &= \frac{\partial}{\partial \nu} \left\{ W(1+\mu)^{1/2} \frac{R}{2} \sum_{k=0}^{\infty} \binom{-\frac{1+\mu}{2} - \mu k}{k} \frac{-(W^2)^k}{-\frac{1+\mu}{2} - \mu k} \right\} \\
&= \frac{\partial}{\partial \nu} \left\{ W^{-\frac{1}{\mu}}(1+\mu)^{1/2} \frac{R}{2} \sum_{k=0}^{\infty} \binom{-\frac{1+\mu}{2} - \mu k}{k} \frac{(W^{\frac{1}{\mu}})^{2\mu k + \mu + 1}}{\frac{1+\mu}{2} + \mu k} \right\} = \\
&= (1+\mu)^{1/2} \frac{R}{2} \left\{ \left[ \frac{\partial}{\partial \nu} \left( W^{-\frac{1}{\mu}} \right) \sum_{k=0}^{\infty} \binom{-\frac{1+\mu}{2} - \mu k}{k} \frac{(W^{\frac{1}{\mu}})^{2\mu k + \mu + 1}}{\frac{1+\mu}{2} + \mu k} \right] \right. \\
&\quad \left. + \left[ W^{-\frac{1}{\mu}} \sum_{k=0}^{\infty} \binom{-\frac{1+\mu}{2} - \mu k}{k} \frac{\frac{\partial}{\partial \nu} \left( (W^{\frac{1}{\mu}})^{2\mu k + \mu + 1} \right)}{\frac{1+\mu}{2} + \mu k} \right] \right\} = \\
&= (1+\mu)^{1/2} \frac{R}{2} \left\{ \left( W^{\frac{1}{\mu}} \right) \frac{\partial}{\partial \nu} \left( W^{-\frac{1}{\mu}} \right) \sum_{k=0}^{\infty} \binom{-\frac{1+\mu}{2} - \mu k}{k} \frac{(W^{\frac{1}{\mu}})^{2\mu k + \mu}}{\frac{1+\mu}{2} + \mu k} \right. \\
&\quad \left. + W^{-\frac{1}{\mu}} \frac{\partial}{\partial \nu} \left( W^{\frac{1}{\mu}} \right) \sum_{k=0}^{\infty} \binom{-\frac{1+\mu}{2} - \mu k}{k} \frac{(2\mu k + \mu + 1) (W^{\frac{1}{\mu}})^{2\mu k + \mu}}{\frac{1+\mu}{2} + \mu k} \right\} \\
&= (1+\mu)^{1/2} \frac{R}{2} \frac{1}{\mu} \frac{\partial W}{\partial \nu} \left\{ \sum_{k=0}^{\infty} \binom{-\frac{1+\mu}{2} - \mu k}{k} \frac{(W^2)^k}{-\frac{1+\mu}{2} - \mu k} + 2 \sum_{k=0}^{\infty} \binom{-\frac{1+\mu}{2} - \mu k}{k} (W^2)^k \right\}
\end{aligned} \tag{B8}$$

The terms in sums with the same binomial coefficients can be put together and then the derivative reads

$$\frac{\partial z(\nu, R)}{\partial \nu} = (1+\mu)^{1/2} R \frac{\partial W}{\partial \nu} \sum_{k=0}^{\infty} \binom{-\frac{1+\mu}{2} - \mu k}{k} \frac{2k+1}{(2k+1)\mu+1} (W^2)^k \tag{B9}$$

This formula works also for  $\mu=0$ .

For the metric factor calculation, also square of the derivative is needed. For further simplification, the before last expression of the derivative is best suited to use:

$$\begin{aligned}
\left(\frac{\partial z(v, R)}{\partial v}\right)^2 &= (1 + \mu) \left(\frac{R}{2}\right)^2 \frac{1}{\mu^2} \left(\frac{\partial W}{\partial v}\right)^2 \left\{ \sum_{k=0}^{\infty} \binom{-\frac{1+\mu}{2} - \mu k}{k} \frac{(W^2)^k}{-\frac{1+\mu}{2} - \mu k} + 2 \sum_{k=0}^{\infty} \binom{-\frac{1+\mu}{2} - \mu k}{k} (W^2)^k \right\}^2 = \\
&= (1 + \mu) \left(\frac{R}{2}\right)^2 \frac{1}{\mu^2} \left(\frac{\partial W}{\partial v}\right)^2 \left\{ \left[ \sum_{k=0}^{\infty} \binom{-\frac{1+\mu}{2} - \mu k}{k} \frac{(W^2)^k}{-\frac{1+\mu}{2} - \mu k} \right]^2 \right. \\
&\quad + 2 \left[ \sum_{k=0}^{\infty} \binom{-\frac{1+\mu}{2} - \mu k}{k} \frac{(W^2)^k}{-\frac{1+\mu}{2} - \mu k} \right] \left[ 2 \sum_{k=0}^{\infty} \binom{-\frac{1+\mu}{2} - \mu k}{k} (W^2)^k \right] \\
&\quad \left. + \left[ 2 \sum_{k=0}^{\infty} \binom{\frac{\mu-1}{2} + (\mu+1)k}{k} (-W^2)^k \right]^2 \right\}
\end{aligned} \tag{B10}$$

where the binomial identity (A3) was used in the third term. The Cauchy products are then used for the three terms:

$$\begin{aligned}
\left(\frac{\partial z(v, R)}{\partial v}\right)^2 &= \\
&= (1 + \mu) \left(\frac{R}{2}\right)^2 \frac{1}{\mu^2} \left(\frac{\partial W}{\partial v}\right)^2 \left\{ \left[ \sum_{k=0}^{\infty} (W^2)^k \sum_{m=0}^k \frac{1}{-\frac{1+\mu}{2} - \mu m} \binom{-\frac{1+\mu}{2} - \mu m}{m} \frac{1}{-\frac{1+\mu}{2} - \mu(k-m)} \binom{-\frac{1+\mu}{2} - \mu(k-m)}{k-m} \right] \right. \\
&\quad + 4 \left[ \sum_{k=0}^{\infty} (W^2)^k \sum_{m=0}^k \binom{-\frac{1+\mu}{2} - \mu m}{m} \frac{1}{-\frac{1+\mu}{2} - \mu m} \binom{-\frac{1+\mu}{2} - \mu(k-m)}{k-m} \right] \\
&\quad \left. + 4 \left[ \sum_{k=0}^{\infty} (-W^2)^k \sum_{m=0}^k \binom{\frac{\mu-1}{2} + (\mu+1)m}{m} \binom{\frac{\mu-1}{2} + (\mu+1)(k-m)}{k-m} \right] \right\}
\end{aligned} \tag{B11}$$

This operation is followed by the use of Hagen-Rothe ([Chu 2010, Chu 2013](#)) and Jensen ([Gould 1972](#)) identities in order to simplify the squared derivative:

$$\begin{aligned}
\left(\frac{\partial z(v, R)}{\partial v}\right)^2 &= (1 + \mu) \left(\frac{R}{2}\right)^2 \frac{1}{\mu^2} \left(\frac{\partial W}{\partial v}\right)^2 \left\{ -4 \sum_{k=0}^{\infty} \frac{1}{1 + \mu} \cdot \frac{1}{-1 - \mu(k+1)} \binom{-1 - \mu(k+1)}{k} (W^2)^k \right. \\
&\quad - 8 \sum_{k=0}^{\infty} \frac{1}{1 + \mu} \cdot \binom{-1 - \mu(k+1)}{k} (W^2)^k \\
&\quad \left. + 4 \sum_{k=0}^{\infty} \left[ (-W^2)^k \sum_{m=0}^k \binom{\mu(k+1) - 1 + (k-m)}{k-m} (1 + \mu)^m \right] \right\} = \\
&= \left(\frac{R}{2}\right)^2 \frac{1}{\mu^2} \left(\frac{\partial W}{\partial v}\right)^2 \left\{ -4 \sum_{k=0}^{\infty} \frac{1}{-1 - \mu(k+1)} \binom{-1 - \mu(k+1)}{k} (W^2)^k \right. \\
&\quad - 8 \sum_{k=0}^{\infty} \binom{-1 - \mu(k+1)}{k} (W^2)^k \\
&\quad \left. + 4(1 + \mu) \sum_{k=0}^{\infty} \left[ (-W^2)^k \sum_{m=0}^k \binom{\mu(k+1) - 1 + m}{m} (1 + \mu)^{k-m} \right] \right\}
\end{aligned} \tag{B12}$$

where reverse counting was used in the inner sum of the third term. For the later use, it is advantageous to rewrite this expression using a substitution  $M=k+1$ ,

$$\begin{aligned} \left(\frac{\partial z(v, R)}{\partial v}\right)^2 &= \left(\frac{R}{2}\right)^2 \frac{1}{\mu^2} \left(\frac{\partial W}{\partial v}\right)^2 \left\{ -4 \sum_{M=1}^{\infty} \frac{1}{-\mu M - 1} \binom{-\mu M - 1}{M - 1} (W^2)^{M-1} \right. \\ &\quad - 8 \sum_{M=1}^{\infty} \binom{-\mu M - 1}{M - 1} (W^2)^{M-1} \\ &\quad \left. + 4 \sum_{M=1}^{\infty} \left[ (-W^2)^{M-1} \sum_{m=0}^{M-1} \binom{\mu M - 1 + m}{m} (1 + \mu)^{M-m} \right] \right\} \end{aligned} \quad (B13)$$

For the later use and with the help of binomial identity  $\binom{\alpha-1}{k-1} = \binom{\alpha}{k} \frac{k}{\alpha}$ , it is of advantage to rewrite the expression to the form

$$\begin{aligned} \left(\frac{\partial z(v, R)}{\partial v}\right)^2 &= \left(\frac{R}{2}\right)^2 \frac{1}{\mu^2} \left(\frac{\partial W}{\partial v}\right)^2 \left\{ \frac{4}{\mu} \sum_{M=1}^{\infty} \frac{1}{-\mu M - 1} \binom{-\mu M}{M} (W^2)^{M-1} + \frac{8}{\mu} \sum_{M=1}^{\infty} \binom{-\mu M}{M} (W^2)^{M-1} \right. \\ &\quad \left. + 4 \sum_{M=1}^{\infty} \left[ (-W^2)^{M-1} \left( \sum_{m=0}^M \binom{\mu M - 1 + m}{m} (1 + \mu)^{M-m} - \binom{(1 + \mu)M - 1}{M} \right) \right] \right\} \end{aligned} \quad (B14)$$

where we also added and subtracted the term with  $m=M$  at the end of the third part, the inner sum, of the series. Now, we also add and subtract the terms with  $M=0$  at the begin of the third series, arriving at the expression

$$\begin{aligned} \left(\frac{\partial z(v, R)}{\partial v}\right)^2 &= \left(\frac{R}{2}\right)^2 \frac{1}{\mu^2} \left(\frac{\partial W}{\partial v}\right)^2 \left\{ \frac{4}{\mu} \sum_{M=1}^{\infty} \frac{1}{-\mu M - 1} \binom{-\mu M}{M} (W^2)^{M-1} + \frac{8}{\mu} \sum_{M=1}^{\infty} \binom{-\mu M}{M} (W^2)^{M-1} \right. \\ &\quad + 4 \sum_{M=0}^{\infty} \left[ (-W^2)^{M-1} \sum_{m=0}^M \binom{\mu M - 1 + m}{m} (1 + \mu)^{M-m} \right] \\ &\quad \left. - 4 \sum_{M=0}^{\infty} (-W^2)^{M-1} \binom{\mu M + M - 1}{M} \right\} \end{aligned} \quad (B15)$$
